# Supplementary material for: Finite groups of symplectic birational transformations of IHS manifolds of $OG10$ type
Source: arXiv:2310.06580 ancillary file (2025-06-23)
Supplement: Supplementary file 1 [file Table2.pdf]

Table 2: Birational symplectic effective  $\chi$ -saturated groups

| $(X, G)$ | $\#G$ | Description of $G$           | $g(\Lambda_G)$                      | $g(\Lambda^G)$                     | K3  | Cubic    | Saturation |
|----------|-------|------------------------------|-------------------------------------|------------------------------------|-----|----------|------------|
| 1F1      | 1     | $C_1 \mid [1, 1]$            | $\Pi_{(0,0)}$                       | $\Pi_{(3,21)}3^1$                  | (0) | $\times$ | —          |
| 1F1.1    | 2     | $C_2 \mid [2, 1]$            | $\Pi_{(0,16)}2_6^{-8}3^1$           | $\Pi_{(3,5)}2_6^8$                 | —   | —        | —          |
| 1F1.2    | 2     | $C_2 \mid [2, 1]$            | $\Pi_{(0,12)}2_2^{-12}3^1$          | $\Pi_{(3,9)}2_2^{12}$              | —   | —        | —          |
| 1F1.3    | 2     | $C_2 \mid [2, 1]$            | $\Pi_{(0,10)}2_4^{-10}3^1$          | $\Pi_{(3,11)}2_0^{10}$             | —   | $\times$ | —          |
| 1F1.4    | 2     | $C_2 \mid [2, 1]$            | $\Pi_{(0,6)}2^{-6}3^1$              | $\Pi_{(3,15)}2^{-6}$               | —   | $\times$ | —          |
| 2F1      | 2     | $C_2 \mid [2, 1]$            | $\Pi_{(0,8)}2^8$                    | $\Pi_{(3,13)}2^83^1$               | (1) | $\times$ | —          |
| 2F1.1    | 4     | $C_2^2 \mid [4, 2]$          | $\Pi_{(0,20)}2_2^{-2}4^{-2}3^1$     | $\Pi_{(3,1)}2_6^{-2}4^{-2}$        | —   | —        | 768        |
| 2F1.2    | 4     | $C_2^2 \mid [4, 2]$          | $\Pi_{(0,18)}2_6^{-4}4_6^23^1$      | $\Pi_{(3,3)}2_0^44_0^2$            | —   | —        | 8          |
| 2F1.3    | 4     | $C_2^2 \mid [4, 2]$          | $\Pi_{(0,16)}2_6^{-6}4_2^23^1$      | $\Pi_{(3,5)}2_6^64^2$              | —   | —        | 8          |
| 2F1.4    | 4     | $C_4 \mid [4, 1]$            | $\Pi_{(0,16)}2_6^{-2}4_4^43^1$      | $\Pi_{(3,5)}2_6^24^4$              | —   | $\times$ | 8          |
| 2F1.5    | 4     | $C_4 \mid [4, 1]$            | $\Pi_{(0,16)}2_2^44_6^{-4}3^1$      | $\Pi_{(3,5)}2_6^44^4$              | —   | —        | —          |
| 2F1.6    | 4     | $C_2^2 \mid [4, 2]$          | $\Pi_{(0,16)}2_4^44_6^{-4}3^1$      | $\Pi_{(3,5)}2_0^44_6^4$            | —   | —        | —          |
| 2F1.7    | 4     | $C_2^2 \mid [4, 2]$          | $\Pi_{(0,15)}2_6^64_5^{-3}3^1$      | $\Pi_{(3,6)}2_4^{-6}4_5^{-3}$      | —   | —        | —          |
| 2F1.8    | 4     | $C_2^2 \mid [4, 2]$          | $\Pi_{(0,14)}2_0^24_4^{-4}3^1$      | $\Pi_{(3,7)}2_4^{-2}4_4^{-4}$      | —   | $\times$ | —          |
| 2F1.9    | 4     | $C_2^2 \mid [4, 2]$          | $\Pi_{(0,14)}2^{-6}4_2^23^1$        | $\Pi_{(3,7)}2^{-6}4^2$             | —   | —        | 8          |
| 2F1.10   | 4     | $C_4 \mid [4, 1]$            | $\Pi_{(0,14)}2^{-2}4_4^43^1$        | $\Pi_{(3,7)}2^{-2}4^4$             | —   | $\times$ | 8          |
| 2F1.11   | 4     | $C_2^2 \mid [4, 2]$          | $\Pi_{(0,12)}2^{-6}4_2^23^1$        | $\Pi_{(3,9)}2^64_2^{-2}$           | —   | $\times$ | —          |
| 2F1.12   | 4     | $C_2^2 \mid [4, 2]$          | $\Pi_{(0,10)}2^44^{-2}3^1$          | $\Pi_{(3,11)}2^44^{-2}$            | —   | $\times$ | —          |
| 3F1      | 4     | $C_2^2 \mid [4, 2]$          | $\Pi_{(0,12)}2^{-6}4^{-2}$          | $\Pi_{(3,9)}2^{-6}4^{-2}3^1$       | (3) | $\times$ | —          |
| 3F1.1    | 8     | $C_2^3 \mid [8, 5]$          | $\Pi_{(0,21)}2_2^{-2}8_7^13^1$      | $\Pi_{(3,0)}2_6^{-2}8_5^{-1}$      | —   | —        | 23040      |
| 3F1.2    | 8     | $D_8 \mid [8, 3]$            | $\Pi_{(0,20)}2_2^{-2}4_2^23^1$      | $\Pi_{(3,1)}2_6^{-2}4^{-2}$        | —   | —        | 768        |
| 3F1.3    | 8     | $D_8 \mid [8, 3]$            | $\Pi_{(0,20)}2_6^24_2^23^1$         | $\Pi_{(3,1)}2_6^{-2}4^{-2}$        | —   | —        | 768        |
| 3F1.4    | 8     | $C_2^3 \mid [8, 5]$          | $\Pi_{(0,20)}2_6^24_2^23^1$         | $\Pi_{(3,1)}2_6^{-2}4^{-2}$        | —   | —        | 768        |
| 3F1.5    | 8     | $C_2^3 \mid [8, 5]$          | $\Pi_{(0,19)}2_4^{-2}4_7^23^1$      | $\Pi_{(3,2)}2_0^24_1^3$            | —   | —        | 16         |
| 3F1.6    | 8     | $C_2^3 \mid [8, 5]$          | $\Pi_{(0,19)}2_6^48_1^13^1$         | $\Pi_{(3,2)}2_6^{-4}8_3^{-1}$      | —   | —        | 48         |
| 3F1.7    | 8     | $D_8 \mid [8, 3]$            | $\Pi_{(0,18)}2_6^{-2}4_5^28_1^13^1$ | $\Pi_{(3,3)}2_2^{-2}4_1^38_5^{-1}$ | —   | —        | —          |
| 3F1.8    | 8     | $C_2^3 \mid [8, 5]$          | $\Pi_{(0,18)}2_6^24_3^{-3}8_7^13^1$ | $\Pi_{(3,3)}2_2^{-2}4_1^38_5^{-1}$ | —   | —        | —          |
| 3F1.9    | 8     | $D_8 \mid [8, 3]$            | $\Pi_{(0,18)}2_2^{-2}4_2^23^1$      | $\Pi_{(3,3)}2_0^24_0^4$            | —   | —        | 32         |
| 3F1.10   | 8     | $C_2^3 \mid [8, 5]$          | $\Pi_{(0,18)}2_0^24_0^43^1$         | $\Pi_{(3,3)}2_0^24_0^4$            | —   | —        | 32         |
| 3F1.11   | 8     | $C_2 \times C_4 \mid [8, 2]$ | $\Pi_{(0,18)}2_4^{-2}4_0^43^1$      | $\Pi_{(3,3)}2_0^24_0^4$            | —   | —        | 32         |
| 3F1.12   | 8     | $D_8 \mid [8, 3]$            | $\Pi_{(0,18)}2_2^24_6^{-4}3^1$      | $\Pi_{(3,3)}2_0^24_0^4$            | —   | —        | 16         |
| 3F1.13   | 8     | $C_2^3 \mid [8, 5]$          | $\Pi_{(0,18)}2^24_4^43^1$           | $\Pi_{(3,3)}2^24^4$                | —   | —        | —          |
| 3F1.14   | 8     | $C_2 \times C_4 \mid [8, 2]$ | $\Pi_{(0,18)}2^{-2}4_4^{-4}3^1$     | $\Pi_{(3,3)}2^24_0^4$              | —   | —        | —          |
| 3F1.15   | 8     | $C_2 \times C_4 \mid [8, 2]$ | $\Pi_{(0,18)}2^24_0^43^1$           | $\Pi_{(3,3)}2^24_0^4$              | —   | —        | 32         |
| 3F1.16   | 8     | $C_2 \times C_4 \mid [8, 2]$ | $\Pi_{(0,18)}4_0^{-4}3^1$           | $\Pi_{(3,3)}4_0^{-4}$              | —   | —        | 96         |
| 3F1.17   | 8     | $C_2^3 \mid [8, 5]$          | $\Pi_{(0,18)}2_4^{-2}4_2^23^1$      | $\Pi_{(3,3)}2_0^44_0^2$            | —   | —        | 96         |
| 3F1.18   | 8     | $C_2^3 \mid [8, 5]$          | $\Pi_{(0,17)}2_4^44_6^28_7^13^1$    | $\Pi_{(3,4)}2_0^{-4}4_4^{-2}8_7^1$ | —   | —        | —          |
| 3F1.19   | 8     | $D_8 \mid [8, 3]$            | $\Pi_{(0,17)}2_6^{-4}4_2^28_7^13^1$ | $\Pi_{(3,4)}2_6^44_2^28_1^1$       | —   | —        | —          |

Table 2: Birational symplectic effective  $\chi$ -saturated groups

| $(X, G)$ | $\#G$ | Description of $G$           | $g(\Lambda_G)$                     | $g(\Lambda^G)$                | K3  | Cubic    | Saturation |
|----------|-------|------------------------------|------------------------------------|-------------------------------|-----|----------|------------|
| 3F1.20   | 8     | $C_2 \times C_4 \mid [8, 2]$ | $\Pi_{(0,17)} 4_1^5 3^1$           | $\Pi_{(3,4)} 4_7^5$           | —   | $\times$ | 16         |
| 3F1.21   | 8     | $D_8 \mid [8, 3]$            | $\Pi_{(0,17)} 2_4^{-4} 4_1^3 3^1$  | $\Pi_{(3,4)} 2_0^4 4_7^3$     | —   | —        | 16         |
| 3F1.22   | 8     | $D_8 \mid [8, 3]$            | $\Pi_{(0,17)} 4_1^{-5} 3^1$        | $\Pi_{(3,4)} 4_7^{-5}$        | —   | —        | 16         |
| 3F1.23   | 8     | $C_2^3 \mid [8, 5]$          | $\Pi_{(0,17)} 2_4^4 4_5^{-3} 3^1$  | $\Pi_{(3,4)} 2_0^4 4_7^3$     | —   | —        | 16         |
| 3F1.24   | 8     | $C_2^3 \mid [8, 5]$          | $\Pi_{(0,16)} 2^4 4_2^{-2} 3^1$    | $\Pi_{(3,5)} 2^4 4_6^{-2}$    | —   | —        | 32         |
| 3F1.25   | 8     | $C_2^3 \mid [8, 5]$          | $\Pi_{(0,16)} 2^2 4_2^{-4} 3^1$    | $\Pi_{(3,5)} 2^2 4_6^{-4}$    | —   | —        | 16         |
| 3F1.26   | 8     | $C_2 \times C_4 \mid [8, 2]$ | $\Pi_{(0,16)} 2^2 4_2^{-4} 3^1$    | $\Pi_{(3,5)} 2^2 4_6^{-4}$    | —   | —        | 16         |
| 3F1.27   | 8     | $D_8 \mid [8, 3]$            | $\Pi_{(0,16)} 2^2 4_2^{-4} 3^1$    | $\Pi_{(3,5)} 2^2 4_6^{-4}$    | —   | —        | 16         |
| 3F1.28   | 8     | $D_8 \mid [8, 3]$            | $\Pi_{(0,16)} 4_3^{-3} 8_7^1 3^1$  | $\Pi_{(3,5)} 4_7^3 8_3^{-1}$  | —   | $\times$ | 16         |
| 3F1.29   | 8     | $C_2^3 \mid [8, 5]$          | $\Pi_{(0,15)} 4_3^{-5} 3^1$        | $\Pi_{(3,6)} 4_5^{-5}$        | —   | $\times$ | —          |
| 3F1.30   | 8     | $C_2^3 \mid [8, 5]$          | $\Pi_{(0,15)} 2^{-6} 8_7^1 3^1$    | $\Pi_{(3,6)} 2^{-6} 8_1^1$    | —   | —        | 16         |
| 3F1.31   | 8     | $C_2^3 \mid [8, 5]$          | $\Pi_{(0,14)} 2^{-6} 4^2 3^1$      | $\Pi_{(3,7)} 2^{-6} 4^2$      | —   | —        | —          |
| 3F1.32   | 8     | $D_8 \mid [8, 3]$            | $\Pi_{(0,14)} 2^{-2} 4^4 3^1$      | $\Pi_{(3,7)} 2^{-2} 4^4$      | —   | $\times$ | —          |
| 3F1.33   | 8     | $C_2^3 \mid [8, 5]$          | $\Pi_{(0,13)} 2^{-6} 8_1^1 3^1$    | $\Pi_{(3,8)} 2^{-6} 8_7^1$    | —   | $\times$ | —          |
| 4C1      | 3     | $C_3 \mid [3, 1]$            | $\Pi_{(0,12)} 3^6$                 | $\Pi_{(3,9)} 3^{-5}$          | —   | $\times$ | 6          |
| 4C1.1    | 6     | $C_6 \mid [6, 2]$            | $\Pi_{(0,18)} 2_6^{-6} 3^{-4}$     | $\Pi_{(3,3)} 2_2^{-6} 3^3$    | —   | —        | 12         |
| 4C1.2    | 6     | $S_3 \mid [6, 1]$            | $\Pi_{(0,18)} 2_4^{-6} 3^{-3}$     | $\Pi_{(3,3)} 2_0^6 3^{-2}$    | —   | —        | 12         |
| 4C1.3    | 6     | $C_6 \mid [6, 2]$            | $\Pi_{(0,18)} 2_6^6 3^{-2}$        | $\Pi_{(3,3)} 2_6^{-6} 3^1$    | —   | —        | 12         |
| 4C1.4    | 6     | $S_3 \mid [6, 1]$            | $\Pi_{(0,16)} 2^4 3^4$             | $\Pi_{(3,5)} 2^4 3^{-3}$      | —   | $\times$ | 24         |
| 4C1.5    | 6     | $C_6 \mid [6, 2]$            | $\Pi_{(0,14)} 2^{-2} 3^5$          | $\Pi_{(3,7)} 2^{-2} 3^4$      | —   | $\times$ | 12         |
| 4C1.6    | 6     | $S_3 \mid [6, 1]$            | $\Pi_{(0,12)} 3^6$                 | $\Pi_{(3,9)} 3^{-5}$          | —   | $\times$ | —          |
| 4F1      | 3     | $C_3 \mid [3, 1]$            | $\Pi_{(0,12)} 3^6$                 | $\Pi_{(3,9)} 3^7$             | (2) | $\times$ | —          |
| 4F1.1    | 6     | $C_6 \mid [6, 2]$            | $\Pi_{(0,20)} 2_6^{-4} 3^3$        | $\Pi_{(3,1)} 2_6^4 3^2$       | —   | —        | 72         |
| 4F1.2    | 6     | $S_3 \mid [6, 1]$            | $\Pi_{(0,18)} 2_2^6 3^6$           | $\Pi_{(3,3)} 2_2^{-6} 3^{-5}$ | —   | —        | —          |
| 4F1.3    | 6     | $C_6 \mid [6, 2]$            | $\Pi_{(0,18)} 2_4^{-6} 3^5$        | $\Pi_{(3,3)} 2_0^6 3^4$       | —   | —        | —          |
| 4F1.4    | 6     | $C_6 \mid [6, 2]$            | $\Pi_{(0,18)} 2_6^{-6} 3^{-4}$     | $\Pi_{(3,3)} 2_2^{-6} 3^3$    | —   | —        | 12         |
| 4F1.5    | 6     | $S_3 \mid [6, 1]$            | $\Pi_{(0,18)} 2_6^6 3^4$           | $\Pi_{(3,3)} 2_6^{-6} 3^{-3}$ | —   | —        | —          |
| 4F1.6    | 6     | $S_3 \mid [6, 1]$            | $\Pi_{(0,18)} 2_0^6 3^{-3}$        | $\Pi_{(3,3)} 2_0^6 3^{-2}$    | —   | —        | 12         |
| 4F1.7    | 6     | $C_6 \mid [6, 2]$            | $\Pi_{(0,16)} 2^4 3^{-6}$          | $\Pi_{(3,5)} 2^4 3^5$         | —   | $\times$ | —          |
| 4F1.8    | 6     | $S_3 \mid [6, 1]$            | $\Pi_{(0,16)} 2_6^4 3^{-5}$        | $\Pi_{(3,5)} 2_2^4 3^{-4}$    | —   | $\times$ | —          |
| 4F1.9    | 6     | $C_6 \mid [6, 2]$            | $\Pi_{(0,16)} 2_4^4 3^{-4}$        | $\Pi_{(3,5)} 2_0^{-4} 3^3$    | —   | $\times$ | —          |
| 5F1      | 2     | $C_2 \mid [2, 1]$            | $\Pi_{(0,12)} 2_4^{12}$            | $\Pi_{(3,9)} 2_0^{-12} 3^1$   | —   | —        | —          |
| 5F1.1    | 4     | $C_2^2 \mid [4, 2]$          | $\Pi_{(0,19)} 2_6^{-2} 4_5^3 3^1$  | $\Pi_{(3,2)} 2_0^2 4_1^3$     | —   | —        | 16         |
| 5F1.2    | 4     | $C_2^2 \mid [4, 2]$          | $\Pi_{(0,18)} 2^4 4_0^2 3^1$       | $\Pi_{(3,3)} 2^4 4_0^2$       | —   | —        | —          |
| 5F1.3    | 4     | $C_2^2 \mid [4, 2]$          | $\Pi_{(0,18)} 4_0^6 3^1$           | $\Pi_{(3,3)} 4_0^6$           | —   | —        | —          |
| 5F1.4    | 4     | $C_4 \mid [4, 1]$            | $\Pi_{(0,18)} 4_0^6 3^1$           | $\Pi_{(3,3)} 4_0^6$           | —   | —        | —          |
| 5F1.5    | 4     | $C_2^2 \mid [4, 2]$          | $\Pi_{(0,17)} 2_6^6 4_3^{-1} 3^1$  | $\Pi_{(3,4)} 2_0^6 4_7^1$     | —   | —        | —          |
| 5F1.6    | 4     | $C_2^2 \mid [4, 2]$          | $\Pi_{(0,17)} 2^{-4} 4_5^{-3} 3^1$ | $\Pi_{(3,4)} 2^4 4_7^3$       | —   | —        | —          |

Table 2: Birational symplectic effective  $\chi$ -saturated groups

| $(X, G)$ | $\#G$ | Description of $G$               | $g(\Lambda_G)$                           | $g(\Lambda^G)$                         | K3  | Cubic    | Saturation |
|----------|-------|----------------------------------|------------------------------------------|----------------------------------------|-----|----------|------------|
| 5F1.7    | 4     | $C_2^2 \mid [4, 2]$              | $\Pi_{(0,17)} 2_2^{-2} 4_3^{-5} 3^1$     | $\Pi_{(3,4)} 2_0^2 4_7^5$              | —   | —        | —          |
| 5F1.8    | 4     | $C_2^2 \mid [4, 2]$              | $\Pi_{(0,16)} 2^4 4_2^3 3^1$             | $\Pi_{(3,5)} 2^4 4_6^4$                | —   | —        | —          |
| 5F1.9    | 4     | $C_2^2 \mid [4, 2]$              | $\Pi_{(0,15)} 2_6^{-6} 4_1^3 3^1$        | $\Pi_{(3,6)} 2_4^{-6} 4_5^{-3}$        | —   | —        | —          |
| 6F1      | 8     | $C_2^3 \mid [8, 5]$              | $\Pi_{(0,14)} 2^6 4_2^2$                 | $\Pi_{(3,7)} 2^6 4_6^2 3^1$            | (9) | —        | —          |
| 6F1.1    | 16    | $C_2^4 \mid [16, 14]$            | $\Pi_{(0,21)} 2_6^2 8_7^3 3^1$           | $\Pi_{(3,0)} 2_6^{-2} 8_5^{-1}$        | —   | —        | 23040      |
| 6F1.2    | 16    | $C_2 \times D_8 \mid [16, 11]$   | $\Pi_{(0,20)} 2_2^{-2} 4^2 3^1$          | $\Pi_{(3,1)} 2_6^{-2} 4^{-2}$          | —   | —        | 768        |
| 6F1.3    | 16    | $C_2^4 \mid [16, 14]$            | $\Pi_{(0,20)} 2_2^{-2} 4^2 3^1$          | $\Pi_{(3,1)} 2_6^{-2} 4^{-2}$          | —   | —        | 768        |
| 6F1.4    | 16    | $C_2 \times D_8 \mid [16, 11]$   | $\Pi_{(0,20)} 2_2^{-2} 4^2 3^1$          | $\Pi_{(3,1)} 2_6^{-2} 4^{-2}$          | —   | —        | 768        |
| 6F1.5    | 16    | $C_2^4 \mid [16, 14]$            | $\Pi_{(0,20)} 2_2^{-2} 4^2 3^1$          | $\Pi_{(3,1)} 2_6^{-2} 4^{-2}$          | —   | —        | 768        |
| 6F1.6    | 16    | $C_2 \times D_8 \mid [16, 11]$   | $\Pi_{(0,19)} 4_7^5 3^1$                 | $\Pi_{(3,2)} 4_1^5$                    | —   | —        | —          |
| 6F1.7    | 16    | $C_2^2 \rtimes C_4 \mid [16, 3]$ | $\Pi_{(0,19)} 4_7^5 3^1$                 | $\Pi_{(3,2)} 4_1^5$                    | —   | —        | —          |
| 6F1.8    | 16    | $C_2^2 \times C_4 \mid [16, 10]$ | $\Pi_{(0,19)} 2_2^{-2} 4^2 8_5^{-1} 3^1$ | $\Pi_{(3,2)} 2_6^{-2} 4^{-2} 8_7^1$    | —   | —        | 128        |
| 6F1.9    | 16    | $C_2 \times D_8 \mid [16, 11]$   | $\Pi_{(0,19)} 2_2^{-2} 4^2 8_5^{-1} 3^1$ | $\Pi_{(3,2)} 2_6^{-2} 4^{-2} 8_7^1$    | —   | —        | 64         |
| 6F1.10   | 16    | $C_2^2 \rtimes C_4 \mid [16, 3]$ | $\Pi_{(0,19)} 2_6^2 4_0^2 8_5^{-1} 3^1$  | $\Pi_{(3,2)} 2_4^{-2} 4_0^2 8_5^{-1}$  | —   | —        | 64         |
| 6F1.11   | 16    | $C_2 \times D_8 \mid [16, 11]$   | $\Pi_{(0,19)} 2_6^2 4_0^2 8_5^{-1} 3^1$  | $\Pi_{(3,2)} 2_4^{-2} 4_0^2 8_5^{-1}$  | —   | —        | 64         |
| 6F1.12   | 16    | $C_2^2 \times C_4 \mid [16, 10]$ | $\Pi_{(0,19)} 2^2 4_7^3 3^1$             | $\Pi_{(3,2)} 2^2 4_1^3$                | —   | —        | —          |
| 6F1.13   | 16    | $C_2^2 \rtimes C_4 \mid [16, 3]$ | $\Pi_{(0,19)} 4_6^2 8_5^{-1} 3^1$        | $\Pi_{(3,2)} 4_0^2 8_5^{-1}$           | —   | —        | 384        |
| 6F1.14   | 16    | $C_2^4 \mid [16, 14]$            | $\Pi_{(0,18)} 2_6^2 4_2^{-4} 3^1$        | $\Pi_{(3,3)} 2_0^2 4_0^4$              | —   | —        | 32         |
| 6F1.15   | 16    | $C_2^2 \rtimes C_4 \mid [16, 3]$ | $\Pi_{(0,18)} 2_6^2 4_2^{-4} 3^1$        | $\Pi_{(3,3)} 2_0^2 4_0^4$              | —   | —        | 32         |
| 6F1.16   | 16    | $C_2 \times D_8 \mid [16, 11]$   | $\Pi_{(0,18)} 2_2^2 4_6^{-4} 3^1$        | $\Pi_{(3,3)} 2_0^2 4_0^4$              | —   | —        | 32         |
| 6F1.17   | 16    | $C_2^2 \times C_4 \mid [16, 10]$ | $\Pi_{(0,18)} 2^2 4_0^3 3^1$             | $\Pi_{(3,3)} 2^2 4_0^4$                | —   | —        | 32         |
| 6F1.18   | 16    | $C_2 \times D_8 \mid [16, 11]$   | $\Pi_{(0,18)} 4_0^{-4} 3^1$              | $\Pi_{(3,3)} 4_0^{-4}$                 | —   | —        | 96         |
| 6F1.19   | 16    | $C_2^2 \rtimes C_4 \mid [16, 3]$ | $\Pi_{(0,18)} 4_0^{-4} 3^1$              | $\Pi_{(3,3)} 4_0^{-4}$                 | —   | —        | 96         |
| 6F1.20   | 16    | $C_2 \times D_8 \mid [16, 11]$   | $\Pi_{(0,18)} 2_6^2 4_2^{-2} 3^1$        | $\Pi_{(3,3)} 2_0^2 4_0^2$              | —   | —        | 96         |
| 6F1.21   | 16    | $C_2 \times D_8 \mid [16, 11]$   | $\Pi_{(0,18)} 4_0^{-4} 3^1$              | $\Pi_{(3,3)} 4_0^{-4}$                 | —   | —        | 96         |
| 6F1.22   | 16    | $C_2^4 \mid [16, 14]$            | $\Pi_{(0,18)} 2_4^{-4} 4_0^2 3^1$        | $\Pi_{(3,3)} 2_0^2 4_0^2$              | —   | —        | 96         |
| 6F1.23   | 16    | $C_2 \times D_8 \mid [16, 11]$   | $\Pi_{(0,18)} 2_6^2 4_2^{-4} 3^1$        | $\Pi_{(3,3)} 2_0^2 4_0^4$              | —   | —        | 32         |
| 6F1.24   | 16    | $C_2^2 \rtimes C_4 \mid [16, 3]$ | $\Pi_{(0,17)} 2^{-2} 4_6^2 8_7^1 3^1$    | $\Pi_{(3,4)} 2^{-2} 4_4^{-2} 8_3^{-1}$ | —   | —        | 32         |
| 6F1.25   | 16    | $C_2 \times D_8 \mid [16, 11]$   | $\Pi_{(0,17)} 2^2 4_2^{-2} 8_7^1 3^1$    | $\Pi_{(3,4)} 2^{-2} 4_4^{-2} 8_3^{-1}$ | —   | —        | 32         |
| 6F1.26   | 16    | $C_2^2 \times C_4 \mid [16, 10]$ | $\Pi_{(0,17)} 2^2 4^{-2} 8_1^1 3^1$      | $\Pi_{(3,4)} 2^2 4^2 8_3^{-1}$         | —   | —        | 32         |
| 6F1.27   | 16    | $C_2 \times D_8 \mid [16, 11]$   | $\Pi_{(0,17)} 2^2 4^{-2} 8_1^1 3^1$      | $\Pi_{(3,4)} 2^2 4^2 8_3^{-1}$         | —   | —        | 32         |
| 6F1.28   | 16    | $C_2^4 \mid [16, 14]$            | $\Pi_{(0,16)} 2^2 4_2^{-4} 3^1$          | $\Pi_{(3,5)} 2^2 4_6^{-4}$             | —   | —        | —          |
| 6F1.29   | 16    | $C_2 \times D_8 \mid [16, 11]$   | $\Pi_{(0,16)} 2^{-2} 4_6^4 3^1$          | $\Pi_{(3,5)} 2^2 4_6^{-4}$             | —   | —        | —          |
| 6F1.30   | 16    | $C_2^4 \mid [16, 14]$            | $\Pi_{(0,16)} 2^4 4_2^{-2} 3^1$          | $\Pi_{(3,5)} 2^4 4_6^{-2}$             | —   | —        | 32         |
| 6F1.31   | 16    | $C_2^4 \mid [16, 14]$            | $\Pi_{(0,15)} 2^{-6} 8_7^1 3^1$          | $\Pi_{(3,6)} 2^{-6} 8_1^1$             | —   | —        | —          |
| 7C1      | 6     | $S_3 \mid [6, 1]$                | $\Pi_{(0,14)} 2^{-2} 3^5$                | $\Pi_{(3,7)} 2^{-2} 3^4$               | —   | $\times$ | 12         |
| 7C1.1    | 12    | $D_{12} \mid [12, 4]$            | $\Pi_{(0,19)} 2_4^{-4} 4_7^1 3^{-3}$     | $\Pi_{(3,2)} 2_0^4 4_1^1 3^{-2}$       | —   | —        | 24         |
| 7C1.2    | 12    | $D_{12} \mid [12, 4]$            | $\Pi_{(0,19)} 2_6^{-4} 4_3^{-1} 3^{-2}$  | $\Pi_{(3,2)} 2_0^4 4_3^{-1} 3^1$       | —   | —        | 24         |

Table 2: Birational symplectic effective  $\chi$ -saturated groups

| $(X, G)$ | $\#G$ | Description of $G$           | $g(\Lambda_G)$                                | $g(\Lambda^G)$                        | K3  | Cubic    | Saturation |
|----------|-------|------------------------------|-----------------------------------------------|---------------------------------------|-----|----------|------------|
| 7C1.3    | 12    | $D_{12} \mid [12, 4]$        | $\Pi_{(0,16)} 2^4 3^4$                        | $\Pi_{(3,5)} 2^4 3^{-3}$              | —   | $\times$ | 24         |
| 7C1.4    | 12    | $D_{12} \mid [12, 4]$        | $\Pi_{(0,14)} 2^{-2} 3^5$                     | $\Pi_{(3,7)} 2^{-2} 3^4$              | —   | $\times$ | —          |
| 7F1      | 6     | $S_3 \mid [6, 1]$            | $\Pi_{(0,14)} 2^{-2} 3^5$                     | $\Pi_{(3,7)} 2^{-2} 3^{-6}$           | (6) | $\times$ | —          |
| 7F1.1    | 12    | $D_{12} \mid [12, 4]$        | $\Pi_{(0,20)} 2_6^{-4} 3^3$                   | $\Pi_{(3,1)} 2_6^4 3^2$               | —   | —        | 72         |
| 7F1.2    | 12    | $D_{12} \mid [12, 4]$        | $\Pi_{(0,19)} 2_4^{-4} 4_7^1 3^5$             | $\Pi_{(3,2)} 2_0^4 4_1^1 3^4$         | —   | —        | —          |
| 7F1.3    | 12    | $D_{12} \mid [12, 4]$        | $\Pi_{(0,19)} 2_2^4 4_3^{-1} 3^4$             | $\Pi_{(3,2)} 2_0^4 4_3^{-1} 3^{-3}$   | —   | —        | —          |
| 7F1.4    | 12    | $D_{12} \mid [12, 4]$        | $\Pi_{(0,19)} 2_2^{-4} 4_1^1 3^{-3}$          | $\Pi_{(3,2)} 2_0^4 4_1^1 3^{-2}$      | —   | —        | 24         |
| 7F1.5    | 12    | $D_{12} \mid [12, 4]$        | $\Pi_{(0,18)} 2_2^6 3^{-4}$                   | $\Pi_{(3,3)} 2_2^6 3^3$               | —   | —        | —          |
| 7F1.6    | 12    | $D_{12} \mid [12, 4]$        | $\Pi_{(0,18)} 2_4^{-6} 3^{-3}$                | $\Pi_{(3,3)} 2_0^6 3^{-2}$            | —   | —        | —          |
| 7F1.7    | 12    | $D_{12} \mid [12, 4]$        | $\Pi_{(0,17)} 2^{-2} 4_1^1 3^{-5}$            | $\Pi_{(3,4)} 2^{-2} 4_7^1 3^{-4}$     | —   | $\times$ | —          |
| 7F1.8    | 12    | $D_{12} \mid [12, 4]$        | $\Pi_{(0,17)} 2_4^{-2} 4_5^{-1} 3^{-4}$       | $\Pi_{(3,4)} 2_0^2 4_5^{-1} 3^3$      | —   | $\times$ | —          |
| 9F1      | 4     | $C_4 \mid [4, 1]$            | $\Pi_{(0,14)} 2_2^2 4^4$                      | $\Pi_{(3,7)} 2_2^{-2} 4^4 3^1$        | (4) | $\times$ | —          |
| 9F1.1    | 8     | $D_8 \mid [8, 3]$            | $\Pi_{(0,21)} 2_2^{-2} 8_1^1 3^1$             | $\Pi_{(3,0)} 2_6^{-2} 8_5^{-1}$       | —   | —        | 23040      |
| 9F1.2    | 8     | $C_8 \mid [8, 1]$            | $\Pi_{(0,20)} 2_5^{-1} 4_5^{-1} 8^2 3^1$      | $\Pi_{(3,1)} 2_1^1 4_1^1 8^2$         | —   | —        | 64         |
| 9F1.3    | 8     | $C_8 \mid [8, 1]$            | $\Pi_{(0,20)} 2_5^{-1} 4_1^1 8^{-2} 3^1$      | $\Pi_{(3,1)} 2_1^1 4_1^1 8^2$         | —   | —        | 32         |
| 9F1.4    | 8     | $C_2 \times C_4 \mid [8, 2]$ | $\Pi_{(0,20)} 2_2^2 4_7^1 8_3^{-1} 3^1$       | $\Pi_{(3,1)} 2_4^{-2} 4_1^1 8_5^{-1}$ | —   | —        | 96         |
| 9F1.5    | 8     | $C_2 \times C_4 \mid [8, 2]$ | $\Pi_{(0,20)} 2_2^{-2} 4^{-2} 3^1$            | $\Pi_{(3,1)} 2_6^{-2} 4^{-2}$         | —   | —        | 768        |
| 9F1.6    | 8     | $D_8 \mid [8, 3]$            | $\Pi_{(0,20)} 2_2^{-2} 4^2 3^1$               | $\Pi_{(3,1)} 2_6^{-2} 4^{-2}$         | —   | —        | 768        |
| 9F1.7    | 8     | $C_2 \times C_4 \mid [8, 2]$ | $\Pi_{(0,19)} 2_4^{-2} 4_5^{-1} 8_2^2 3^1$    | $\Pi_{(3,2)} 2_6^2 4_1^1 8_2^2$       | —   | —        | 16         |
| 9F1.8    | 8     | $D_8 \mid [8, 3]$            | $\Pi_{(0,19)} 2_4^{-2} 4_1^1 8_6^2 3^1$       | $\Pi_{(3,2)} 2_6^2 4_1^1 8_2^2$       | —   | —        | 16         |
| 9F1.9    | 8     | $C_8 \mid [8, 1]$            | $\Pi_{(0,19)} 2^2 4_1^1 8^2 3^1$              | $\Pi_{(3,2)} 2^{-2} 4_1^1 8^{-2}$     | —   | —        | —          |
| 9F1.10   | 8     | $C_2 \times C_4 \mid [8, 2]$ | $\Pi_{(0,19)} 4_7^5 3^1$                      | $\Pi_{(3,2)} 4_1^5$                   | —   | —        | 64         |
| 9F1.11   | 8     | $Q_8 \mid [8, 4]$            | $\Pi_{(0,19)} 4_7^5 3^1$                      | $\Pi_{(3,2)} 4_1^5$                   | —   | —        | 64         |
| 9F1.12   | 8     | $D_8 \mid [8, 3]$            | $\Pi_{(0,19)} 2_6^{-2} 4_4^{-2} 8_5^{-1} 3^1$ | $\Pi_{(3,2)} 2_4^{-2} 4_0^2 8_5^{-1}$ | —   | —        | 16         |
| 9F1.13   | 8     | $Q_8 \mid [8, 4]$            | $\Pi_{(0,19)} 2_7^{-3} 8^{-2} 3^1$            | $\Pi_{(3,2)} 2_1^{-3} 8^{-2}$         | —   | —        | 16         |
| 9F1.14   | 8     | $Q_8 \mid [8, 4]$            | $\Pi_{(0,19)} 2_3^3 8^{-2} 3^1$               | $\Pi_{(3,2)} 2_1^{-3} 8^{-2}$         | —   | —        | 32         |
| 9F1.15   | 8     | $D_8 \mid [8, 3]$            | $\Pi_{(0,19)} 2_3^{-3} 8^2 3^1$               | $\Pi_{(3,2)} 2_1^3 8^2$               | —   | —        | 32         |
| 9F1.16   | 8     | $D_8 \mid [8, 3]$            | $\Pi_{(0,19)} 2_0^2 4_7^3 3^1$                | $\Pi_{(3,2)} 2_0^2 4_1^3$             | —   | —        | 128        |
| 9F1.17   | 8     | $D_8 \mid [8, 3]$            | $\Pi_{(0,19)} 4_7^5 3^1$                      | $\Pi_{(3,2)} 4_1^5$                   | —   | —        | 64         |
| 9F1.18   | 8     | $Q_8 \mid [8, 4]$            | $\Pi_{(0,19)} 2_3^3 8^{-2} 3^1$               | $\Pi_{(3,2)} 2_1^{-3} 8^{-2}$         | —   | —        | 16         |
| 9F1.19   | 8     | $C_2 \times C_4 \mid [8, 2]$ | $\Pi_{(0,19)} 2_6^{-2} 4_5^3 3^1$             | $\Pi_{(3,2)} 2_0^2 4_1^3$             | —   | —        | 128        |
| 9F1.20   | 8     | $C_2 \times C_4 \mid [8, 2]$ | $\Pi_{(0,19)} 2_6^4 8_5^{-1} 3^1$             | $\Pi_{(3,2)} 2_6^{-4} 8_3^{-1}$       | —   | —        | 48         |
| 9F1.21   | 8     | $Q_8 \mid [8, 4]$            | $\Pi_{(0,19)} 4_7^{-3} 3^1$                   | $\Pi_{(3,2)} 4_1^{-3}$                | —   | —        | 384        |
| 9F1.22   | 8     | $Q_8 \mid [8, 4]$            | $\Pi_{(0,18)} 2_2^2 4_6^{-4} 3^1$             | $\Pi_{(3,3)} 2_0^2 4_0^4$             | —   | —        | 32         |
| 9F1.23   | 8     | $C_2 \times C_4 \mid [8, 2]$ | $\Pi_{(0,18)} 2_2^{-2} 4_2^4 3^1$             | $\Pi_{(3,3)} 2_0^2 4_0^4$             | —   | —        | 32         |
| 9F1.24   | 8     | $D_8 \mid [8, 3]$            | $\Pi_{(0,18)} 2_0^4 8_0^2 3^1$                | $\Pi_{(3,3)} 2_0^4 8_0^2$             | —   | —        | —          |
| 9F1.25   | 8     | $C_2 \times C_4 \mid [8, 2]$ | $\Pi_{(0,18)} 2_2^{-4} 8_2^2 3^1$             | $\Pi_{(3,3)} 2_2^4 8_6^2$             | —   | —        | 16         |
| 9F1.26   | 8     | $C_2 \times C_4 \mid [8, 2]$ | $\Pi_{(0,18)} 2_2^4 8_6^2 3^1$                | $\Pi_{(3,3)} 2_6^4 8_2^2$             | —   | —        | —          |

Table 2: Birational symplectic effective  $\chi$ -saturated groups

| $(X, G)$ | $\#G$ | Description of $G$               | $g(\Lambda_G)$                                | $g(\Lambda^G)$                         | K3   | Cubic    | Saturation |
|----------|-------|----------------------------------|-----------------------------------------------|----------------------------------------|------|----------|------------|
| 9F1.27   | 8     | $C_8 \mid [8, 1]$                | $\Pi_{(0,18)} 2_3^{-1} 4_1^1 8^2 3^1$         | $\Pi_{(3,3)} 2_7^1 4_1^1 8^2$          | —    | $\times$ | 16         |
| 9F1.28   | 8     | $D_8 \mid [8, 3]$                | $\Pi_{(0,18)} 2_6^{-2} 4_6^4 3^1$             | $\Pi_{(3,3)} 2_0^2 4_0^4$              | —    | —        | 32         |
| 9F1.29   | 8     | $C_2 \times C_4 \mid [8, 2]$     | $\Pi_{(0,18)} 2^2 4_0^2 3^1$                  | $\Pi_{(3,3)} 2^2 4_0^4$                | —    | —        | 32         |
| 9F1.30   | 8     | $C_2 \times C_4 \mid [8, 2]$     | $\Pi_{(0,18)} 2^{-2} 4_4^{-4} 3^1$            | $\Pi_{(3,3)} 2^2 4_0^4$                | —    | —        | 16         |
| 9F1.31   | 8     | $C_2 \times C_4 \mid [8, 2]$     | $\Pi_{(0,18)} 4_0^{-4} 3^1$                   | $\Pi_{(3,3)} 4_0^{-4}$                 | —    | —        | 96         |
| 9F1.32   | 8     | $C_2 \times C_4 \mid [8, 2]$     | $\Pi_{(0,18)} 2_2^2 8_6^{-2} 3^1$             | $\Pi_{(3,3)} 2_2^{-2} 8_6^{-2}$        | —    | $\times$ | 16         |
| 9F1.33   | 8     | $D_8 \mid [8, 3]$                | $\Pi_{(0,18)} 2_4^4 4_4^{-2} 3^1$             | $\Pi_{(3,3)} 2_0^4 4_0^2$              | —    | —        | 96         |
| 9F1.34   | 8     | $D_8 \mid [8, 3]$                | $\Pi_{(0,17)} 2_1^3 8^2 3^1$                  | $\Pi_{(3,4)} 2_7^3 8^2$                | —    | $\times$ | —          |
| 9F1.35   | 8     | $C_2 \times C_4 \mid [8, 2]$     | $\Pi_{(0,17)} 2_6^{-4} 4_7^2 8_7^1 3^1$       | $\Pi_{(3,4)} 2_6^4 4_7^2 8_1^1$        | —    | —        | —          |
| 9F1.36   | 8     | $D_8 \mid [8, 3]$                | $\Pi_{(0,17)} 4_1^{-5} 3^1$                   | $\Pi_{(3,4)} 4_7^{-5}$                 | —    | —        | 16         |
| 9F1.37   | 8     | $Q_8 \mid [8, 4]$                | $\Pi_{(0,17)} 4_1^5 3^1$                      | $\Pi_{(3,4)} 4_7^5$                    | —    | $\times$ | 16         |
| 9F1.38   | 8     | $C_2 \times C_4 \mid [8, 2]$     | $\Pi_{(0,17)} 2_6^{-4} 4_7^3 3^1$             | $\Pi_{(3,4)} 2_0^4 4_7^3$              | —    | —        | 16         |
| 9F1.39   | 8     | $D_8 \mid [8, 3]$                | $\Pi_{(0,17)} 2^2 4_0^2 8_5^{-1} 3^1$         | $\Pi_{(3,4)} 2^{-2} 4_4^{-2} 8_3^{-1}$ | —    | —        | 32         |
| 9F1.40   | 8     | $C_2 \times C_4 \mid [8, 2]$     | $\Pi_{(0,16)} 2_6^{-2} 4^4 3^1$               | $\Pi_{(3,5)} 2_6^2 4^4$                | —    | $\times$ | —          |
| 9F1.41   | 8     | $D_8 \mid [8, 3]$                | $\Pi_{(0,16)} 2_6^{-6} 4^2 3^1$               | $\Pi_{(3,5)} 2_6^6 4^2$                | —    | —        | —          |
| 9F1.42   | 8     | $C_2 \times C_4 \mid [8, 2]$     | $\Pi_{(0,16)} 4_1^3 8_5^{-1} 3^1$             | $\Pi_{(3,5)} 4_7^3 8_3^{-1}$           | —    | $\times$ | 16         |
| 9F1.43   | 8     | $D_8 \mid [8, 3]$                | $\Pi_{(0,15)} 2_2^2 4_8^2 8_1^1 3^1$          | $\Pi_{(3,6)} 2_2^{-2} 4^2 8_3^{-1}$    | —    | $\times$ | —          |
| 10F1     | 16    | $C_2^4 \mid [16, 14]$            | $\Pi_{(0,15)} 2^6 8_1^1$                      | $\Pi_{(3,6)} 2^6 8_7^1 3^1$            | (21) | —        | —          |
| 10F1.1   | 32    | $C_2^5 \mid [32, 51]$            | $\Pi_{(0,21)} 2^{-2} 8_7^1 3^1$               | $\Pi_{(3,0)} 2_6^{-2} 8_5^{-1}$        | —    | —        | 23040      |
| 10F1.2   | 32    | $C_2^2 \times D_8 \mid [32, 46]$ | $\Pi_{(0,20)} 2_2^{-2} 4^{-2} 3^1$            | $\Pi_{(3,1)} 2_6^{-2} 4^{-2}$          | —    | —        | 768        |
| 10F1.3   | 32    | $C_2^2 \wr C_2 \mid [32, 27]$    | $\Pi_{(0,19)} 2_2^{-2} 4_2^{-2} 8_3^{-1} 3^1$ | $\Pi_{(3,2)} 2_4^{-2} 4_0^2 8_5^{-1}$  | —    | —        | 64         |
| 10F1.4   | 32    | $C_2^2 \wr C_2 \mid [32, 27]$    | $\Pi_{(0,19)} 4_6^2 8_5^{-1} 3^1$             | $\Pi_{(3,2)} 4_0^2 8_5^{-1}$           | —    | —        | 384        |
| 10F1.5   | 32    | $C_2^2 \wr C_2 \mid [32, 27]$    | $\Pi_{(0,18)} 4_0^{-4} 3^1$                   | $\Pi_{(3,3)} 4_0^{-4}$                 | —    | —        | 96         |
| 10F1.6   | 32    | $C_2^2 \wr C_2 \mid [32, 27]$    | $\Pi_{(0,18)} 2_0^{-4} 4_4^{-2} 3^1$          | $\Pi_{(3,3)} 2_0^4 4_0^2$              | —    | —        | 96         |
| 10F1.7   | 32    | $C_2^2 \times D_8 \mid [32, 46]$ | $\Pi_{(0,17)} 2^2 4_2^2 8_5^{-1} 3^1$         | $\Pi_{(3,4)} 2^2 4_2^2 8_3^{-1}$       | —    | —        | —          |
| 10F1.8   | 32    | $C_2^5 \mid [32, 51]$            | $\Pi_{(0,16)} 2^{-4} 4_6^2 3^1$               | $\Pi_{(3,5)} 2^4 4_6^{-2}$             | —    | —        | —          |
| 13F1     | 8     | $D_8 \mid [8, 3]$                | $\Pi_{(0,15)} 4_1^5$                          | $\Pi_{(3,6)} 4_7^5 3^1$                | (10) | $\times$ | —          |
| 13F1.1   | 16    | $C_2 \times D_8 \mid [16, 11]$   | $\Pi_{(0,21)} 2_6^2 8_3^{-1} 3^1$             | $\Pi_{(3,0)} 2_6^{-2} 8_5^{-1}$        | —    | —        | 23040      |
| 13F1.2   | 16    | $D_{16} \mid [16, 7]$            | $\Pi_{(0,20)} 2_1^1 4_5^{-1} 8^2 3^1$         | $\Pi_{(3,1)} 2_1^1 4_1^1 8^2$          | —    | —        | 64         |
| 13F1.3   | 16    | $QD_{16} \mid [16, 8]$           | $\Pi_{(0,20)} 2_1^1 4_5^{-1} 8^2 3^1$         | $\Pi_{(3,1)} 2_1^1 4_1^1 8^2$          | —    | —        | 64         |
| 13F1.4   | 16    | $QD_{16} \mid [16, 8]$           | $\Pi_{(0,20)} 2_1^1 4_1^1 8^{-2} 3^1$         | $\Pi_{(3,1)} 2_1^1 4_1^1 8^2$          | —    | —        | 32         |
| 13F1.5   | 16    | $C_2 \times D_8 \mid [16, 11]$   | $\Pi_{(0,20)} 2_6^{-2} 4_3^{-1} 8_1^1 3^1$    | $\Pi_{(3,1)} 2_4^{-2} 4_1^1 8_5^{-1}$  | —    | —        | 96         |
| 13F1.6   | 16    | $C_2 \times D_8 \mid [16, 11]$   | $\Pi_{(0,20)} 2_2^{-2} 4^2 3^1$               | $\Pi_{(3,1)} 2_6^{-2} 4^{-2}$          | —    | —        | 768        |
| 13F1.7   | 16    | $C_4 \circ D_8 \mid [16, 13]$    | $\Pi_{(0,20)} 2_6^2 4^{-2} 3^1$               | $\Pi_{(3,1)} 2_6^{-2} 4^{-2}$          | —    | —        | 768        |
| 13F1.8   | 16    | $C_2 \times D_8 \mid [16, 11]$   | $\Pi_{(0,20)} 2_2^{-2} 4^2 3^1$               | $\Pi_{(3,1)} 2_6^{-2} 4^{-2}$          | —    | —        | 768        |
| 13F1.9   | 16    | $C_2 \times D_8 \mid [16, 11]$   | $\Pi_{(0,19)} 2_4^{-2} 4_1^1 8_6^2 3^1$       | $\Pi_{(3,2)} 2_6^2 4_1^1 8_2^2$        | —    | —        | —          |
| 13F1.10  | 16    | $C_2 \times D_8 \mid [16, 11]$   | $\Pi_{(0,19)} 2_6^2 4_1^1 8_4^{-2} 3^1$       | $\Pi_{(3,2)} 2_6^2 4_1^1 8_2^2$        | —    | —        | —          |
| 13F1.11  | 16    | $C_4 \circ D_8 \mid [16, 13]$    | $\Pi_{(0,19)} 4_7^5 3^1$                      | $\Pi_{(3,2)} 4_1^5$                    | —    | —        | 64         |

Table 2: Birational symplectic effective  $\chi$ -saturated groups

| $(X, G)$ | $\#G$ | Description of $G$                      | $g(\Lambda_G)$                        | $g(\Lambda^G)$                         | K3   | Cubic | Saturation |
|----------|-------|-----------------------------------------|---------------------------------------|----------------------------------------|------|-------|------------|
| 13F1.12  | 16    | $C_4 \circ D_8$   [16, 13]              | $\Pi_{(0,19)} 4_7^5 3^1$              | $\Pi_{(3,2)} 4_1^5$                    | —    | —     | 64         |
| 13F1.13  | 16    | $QD_{16}$   [16, 8]                     | $\Pi_{(0,19)} 2_3^3 8^{-2} 3^1$       | $\Pi_{(3,2)} 2_1^{-3} 8^{-2}$          | —    | —     | 32         |
| 13F1.14  | 16    | $D_{16}$   [16, 7]                      | $\Pi_{(0,19)} 2_3^{-3} 8^2 3^1$       | $\Pi_{(3,2)} 2_1^3 8^2$                | —    | —     | 32         |
| 13F1.15  | 16    | $C_4 \circ D_8$   [16, 13]              | $\Pi_{(0,19)} 4_7^5 3^1$              | $\Pi_{(3,2)} 4_1^5$                    | —    | —     | 64         |
| 13F1.16  | 16    | $C_2 \times D_8$   [16, 11]             | $\Pi_{(0,19)} 4_7^5 3^1$              | $\Pi_{(3,2)} 4_1^5$                    | —    | —     | 64         |
| 13F1.17  | 16    | $C_2 \times D_8$   [16, 11]             | $\Pi_{(0,19)} 2_6^2 4_1^{-3} 3^1$     | $\Pi_{(3,2)} 2_0^2 4_1^3$              | —    | —     | 128        |
| 13F1.18  | 16    | $C_2 \times D_8$   [16, 11]             | $\Pi_{(0,19)} 2_2^{-2} 4_1^{-3} 3^1$  | $\Pi_{(3,2)} 2_0^2 4_1^3$              | —    | —     | 128        |
| 13F1.19  | 16    | $C_2 \times D_8$   [16, 11]             | $\Pi_{(0,19)} 2_2^{-2} 4_1^3 3^1$     | $\Pi_{(3,2)} 2_0^2 4_1^3$              | —    | —     | 128        |
| 13F1.20  | 16    | $C_4 \circ D_8$   [16, 13]              | $\Pi_{(0,19)} 2_6^{-2} 4_5^{-3} 3^1$  | $\Pi_{(3,2)} 2_0^2 4_1^3$              | —    | —     | 128        |
| 13F1.21  | 16    | $C_2 \times D_8$   [16, 11]             | $\Pi_{(0,19)} 2_2^2 4_5^{-3} 3^1$     | $\Pi_{(3,2)} 2_0^2 4_1^3$              | —    | —     | 128        |
| 13F1.22  | 16    | $C_4 \circ D_8$   [16, 13]              | $\Pi_{(0,19)} 4_7^{-3} 3^1$           | $\Pi_{(3,2)} 4_1^{-3}$                 | —    | —     | 384        |
| 13F1.23  | 16    | $C_4 \circ D_8$   [16, 13]              | $\Pi_{(0,18)} 2^2 4_0^4 3^1$          | $\Pi_{(3,3)} 2^2 4_0^4$                | —    | —     | 32         |
| 13F1.24  | 16    | $D_{16}$   [16, 7]                      | $\Pi_{(0,18)} 2_3^{-1} 4_1^1 8^2 3^1$ | $\Pi_{(3,3)} 2_7^1 4_1^1 8^2$          | —    | ×     | —          |
| 13F1.25  | 16    | $C_2 \times D_8$   [16, 11]             | $\Pi_{(0,18)} 4_0^{-4} 3^1$           | $\Pi_{(3,3)} 4_0^{-4}$                 | —    | —     | 96         |
| 13F1.26  | 16    | $C_2 \times D_8$   [16, 11]             | $\Pi_{(0,18)} 2_4^{-4} 4_0^2 3^1$     | $\Pi_{(3,3)} 2_0^4 4_0^2$              | —    | —     | 96         |
| 13F1.27  | 16    | $C_2 \times D_8$   [16, 11]             | $\Pi_{(0,18)} 2_0^2 4_0^4 3^1$        | $\Pi_{(3,3)} 2_0^2 4_0^4$              | —    | —     | 32         |
| 13F1.28  | 16    | $C_4 \circ D_8$   [16, 13]              | $\Pi_{(0,18)} 2_4^{-2} 4_0^4 3^1$     | $\Pi_{(3,3)} 2_0^2 4_0^4$              | —    | —     | 32         |
| 13F1.29  | 16    | $C_2 \times D_8$   [16, 11]             | $\Pi_{(0,18)} 2_2^{-2} 4_2^{-4} 3^1$  | $\Pi_{(3,3)} 2_0^2 4_0^4$              | —    | —     | 32         |
| 13F1.30  | 16    | $C_4 \circ D_8$   [16, 13]              | $\Pi_{(0,18)} 2_6^2 4_2^3 3^1$        | $\Pi_{(3,3)} 2_0^2 4_0^4$              | —    | —     | 32         |
| 13F1.31  | 16    | $C_2 \times D_8$   [16, 11]             | $\Pi_{(0,17)} 4_1^{-5} 3^1$           | $\Pi_{(3,4)} 4_7^{-5}$                 | —    | —     | —          |
| 13F1.32  | 16    | $C_4 \circ D_8$   [16, 13]              | $\Pi_{(0,17)} 4_1^5 3^1$              | $\Pi_{(3,4)} 4_7^5$                    | —    | ×     | —          |
| 13F1.33  | 16    | $C_2 \times D_8$   [16, 11]             | $\Pi_{(0,17)} 2_4^{-4} 4_1^3 3^1$     | $\Pi_{(3,4)} 2_0^4 4_7^3$              | —    | —     | —          |
| 13F1.34  | 16    | $C_2 \times D_8$   [16, 11]             | $\Pi_{(0,17)} 2^2 4_0^2 8_5^{-1} 3^1$ | $\Pi_{(3,4)} 2^{-2} 4_4^{-2} 8_3^{-1}$ | —    | —     | 32         |
| 13F1.35  | 16    | $C_2 \times D_8$   [16, 11]             | $\Pi_{(0,16)} 4_1^3 8_5^{-1} 3^1$     | $\Pi_{(3,5)} 4_7^3 8_3^{-1}$           | —    | ×     | —          |
| 15C1     | 18    | $A_{3,3}$   [18, 4]                     | $\Pi_{(0,16)} 3^4 9^{-1}$             | $\Pi_{(3,5)} 3^{-3} 9^1$               | —    | ×     | 36         |
| 15C1.1   | 36    | $S_3^2$   [36, 10]                      | $\Pi_{(0,20)} 2_0^{-4} 3^4$           | $\Pi_{(3,1)} 2_0^{-4} 3^{-3}$          | —    | —     | 72         |
| 15C1.2   | 36    | $C_2 \times C_3 \rtimes S_3$   [36, 13] | $\Pi_{(0,20)} 2_6^4 3^1 9^{-1}$       | $\Pi_{(3,1)} 2_2^4 9^1$                | —    | —     | 144        |
| 15C1.3   | 36    | $C_3^2 \rtimes C_4$   [36, 9]           | $\Pi_{(0,20)} 2_2^4 3^3$              | $\Pi_{(3,1)} 2_6^4 3^2$                | —    | —     | 72         |
| 15C1.4   | 36    | $C_2 \times C_3 \rtimes S_3$   [36, 13] | $\Pi_{(0,20)} 2_2^4 3^3$              | $\Pi_{(3,1)} 2_6^4 3^2$                | —    | —     | 72         |
| 15C1.5   | 36    | $C_3^2 \rtimes C_4$   [36, 9]           | $\Pi_{(0,18)} 2^{-2} 3^3 9^{-1}$      | $\Pi_{(3,3)} 2^{-2} 3^2 9^1$           | —    | ×     | 72         |
| 15C1.6   | 36    | $C_2 \times C_3 \rtimes S_3$   [36, 13] | $\Pi_{(0,18)} 2^{-2} 3^3 9^{-1}$      | $\Pi_{(3,3)} 2^{-2} 3^2 9^1$           | —    | ×     | 72         |
| 15C1.7   | 36    | $S_3^2$   [36, 10]                      | $\Pi_{(0,18)} 2_6^{-2} 3^2 9^{-1}$    | $\Pi_{(3,3)} 2_2^{-2} 3^{-1} 9^1$      | —    | ×     | 72         |
| 15C1.8   | 36    | $S_3^2$   [36, 10]                      | $\Pi_{(0,16)} 3^4 9^{-1}$             | $\Pi_{(3,5)} 3^{-3} 9^1$               | —    | ×     | —          |
| 15F1     | 18    | $A_{3,3}$   [18, 4]                     | $\Pi_{(0,16)} 3^4 9^{-1}$             | $\Pi_{(3,5)} 3^5 9^1$                  | (30) | ×     | —          |
| 15F1.1   | 36    | $S_3^2$   [36, 10]                      | $\Pi_{(0,20)} 2_6^4 3^{-3} 9^{-1}$    | $\Pi_{(3,1)} 2_2^4 3^{-2} 9^1$         | —    | —     | —          |
| 15F1.2   | 36    | $S_3^2$   [36, 10]                      | $\Pi_{(0,20)} 2_0^{-4} 3^4$           | $\Pi_{(3,1)} 2_0^{-4} 3^{-3}$          | —    | —     | 72         |
| 15F1.3   | 36    | $C_2 \times C_3 \rtimes S_3$   [36, 13] | $\Pi_{(0,20)} 2_0^{-4} 3^{-2} 9^{-1}$ | $\Pi_{(3,1)} 2_0^{-4} 3^1 9^1$         | —    | —     | —          |
| 15F1.4   | 36    | $C_3^2 \rtimes C_4$   [36, 9]           | $\Pi_{(0,20)} 2_2^4 3^3$              | $\Pi_{(3,1)} 2_6^4 3^2$                | —    | —     | 72         |

Table 2: Birational symplectic effective  $\chi$ -saturated groups

| $(X, G)$ | $\#G$ | Description of $G$                         | $g(\Lambda_G)$                                | $g(\Lambda^G)$                        | K3   | Cubic    | Saturation |
|----------|-------|--------------------------------------------|-----------------------------------------------|---------------------------------------|------|----------|------------|
| 15F1.5   | 36    | $C_3^2 \rtimes C_4 \mid [36, 9]$           | $\Pi_{(0,20)} 2_2^2 3^3$                      | $\Pi_{(3,1)} 2_6^2 3^2$               | —    | $\times$ | 3888       |
| 15F1.6   | 36    | $C_2 \times C_3 \rtimes S_3 \mid [36, 13]$ | $\Pi_{(0,18)} 2_4^{-2} 3^5$                   | $\Pi_{(3,3)} 2_0^2 3^4$               | —    | $\times$ | —          |
| 17F1     | 16    | $C_2 \times D_8 \mid [16, 11]$             | $\Pi_{(0,16)} 2^2 4_0^4$                      | $\Pi_{(3,5)} 2^2 4_0^4 3^1$           | (22) | —        | —          |
| 17F1.1   | 32    | $C_2^2 \wr C_2 \mid [32, 27]$              | $\Pi_{(0,21)} 2_2^{-2} 8_3^{-1} 3^1$          | $\Pi_{(3,0)} 2_6^{-2} 8_5^{-1}$       | —    | —        | 23040      |
| 17F1.2   | 32    | $C_2^2 \times D_8 \mid [32, 46]$           | $\Pi_{(0,21)} 2_6^2 8_7^1 3^1$                | $\Pi_{(3,0)} 2_6^{-2} 8_5^{-1}$       | —    | —        | 23040      |
| 17F1.3   | 32    | $C_2^2 \wr C_2 \mid [32, 27]$              | $\Pi_{(0,21)} 2_6^2 8_7^1 3^1$                | $\Pi_{(3,0)} 2_6^{-2} 8_5^{-1}$       | —    | —        | 23040      |
| 17F1.4   | 32    | $\text{Aut}(D_{16}) \mid [32, 43]$         | $\Pi_{(0,20)} 2_7^1 4_7^1 8^2 3^1$            | $\Pi_{(3,1)} 2_1^1 4_1^1 8^2$         | —    | —        | 64         |
| 17F1.5   | 32    | $C_2 \times D_{16} \mid [32, 39]$          | $\Pi_{(0,20)} 2_3^{-1} 4_3^{-1} 8^{-2} 3^1$   | $\Pi_{(3,1)} 2_1^1 4_1^1 8^2$         | —    | —        | 64         |
| 17F1.6   | 32    | [32, 34]                                   | $\Pi_{(0,20)} 2_6^2 8_4^{-2} 3^1$             | $\Pi_{(3,1)} 2_2^2 8_0^2$             | —    | —        | 256        |
| 17F1.7   | 32    | [32, 28]                                   | $\Pi_{(0,20)} 2_6^2 8_4^{-2} 3^1$             | $\Pi_{(3,1)} 2_2^2 8_0^2$             | —    | —        | 256        |
| 17F1.8   | 32    | [32, 28]                                   | $\Pi_{(0,20)} 4_6^4 3^1$                      | $\Pi_{(3,1)} 4_2^4$                   | —    | —        | —          |
| 17F1.9   | 32    | $C_2^3 \rtimes C_4 \mid [32, 6]$           | $\Pi_{(0,20)} 2_4^{-2} 4_5^{-1} 8_5^{-1} 3^1$ | $\Pi_{(3,1)} 2_4^{-2} 4_1^1 8_5^{-1}$ | —    | —        | 768        |
| 17F1.10  | 32    | $C_2^3 \rtimes C_4 \mid [32, 6]$           | $\Pi_{(0,20)} 2_4^{-2} 4_5^{-1} 8_5^{-1} 3^1$ | $\Pi_{(3,1)} 2_4^{-2} 4_1^1 8_5^{-1}$ | —    | —        | 768        |
| 17F1.11  | 32    | $C_2^2 \times D_8 \mid [32, 46]$           | $\Pi_{(0,20)} 2_6^2 4^2 3^1$                  | $\Pi_{(3,1)} 2_6^{-2} 4^{-2}$         | —    | —        | 768        |
| 17F1.12  | 32    | $C_2^2 \wr C_2 \mid [32, 27]$              | $\Pi_{(0,20)} 2_2^{-2} 4^2 3^1$               | $\Pi_{(3,1)} 2_6^{-2} 4^{-2}$         | —    | —        | 768        |
| 17F1.13  | 32    | $C_2^2 \times D_8 \mid [32, 46]$           | $\Pi_{(0,20)} 2_6^2 4^2 3^1$                  | $\Pi_{(3,1)} 2_6^{-2} 4^{-2}$         | —    | —        | 768        |
| 17F1.14  | 32    | [32, 28]                                   | $\Pi_{(0,20)} 2_6^2 4^2 3^1$                  | $\Pi_{(3,1)} 2_6^{-2} 4^{-2}$         | —    | —        | 768        |
| 17F1.15  | 32    | $2_+^{1+4} \mid [32, 49]$                  | $\Pi_{(0,20)} 2_6^2 4^{-2} 3^1$               | $\Pi_{(3,1)} 2_6^{-2} 4^{-2}$         | —    | —        | 768        |
| 17F1.16  | 32    | $C_2^3 \rtimes C_4 \mid [32, 6]$           | $\Pi_{(0,20)} 4_5^{-1} 8_1^1 3^1$             | $\Pi_{(3,1)} 4_1^1 8_5^{-1}$          | —    | —        | 11520      |
| 17F1.17  | 32    | $C_2^2 \times D_8 \mid [32, 46]$           | $\Pi_{(0,20)} 2_2^{-2} 4^2 3^1$               | $\Pi_{(3,1)} 2_6^{-2} 4^{-2}$         | —    | —        | 768        |
| 17F1.18  | 32    | $C_2 \times C_4 \circ D_8 \mid [32, 48]$   | $\Pi_{(0,19)} 4_7^5 3^1$                      | $\Pi_{(3,2)} 4_1^5$                   | —    | —        | 64         |
| 17F1.19  | 32    | $2_+^{1+4} \mid [32, 49]$                  | $\Pi_{(0,19)} 4_7^5 3^1$                      | $\Pi_{(3,2)} 4_1^5$                   | —    | —        | 64         |
| 17F1.20  | 32    | [32, 30]                                   | $\Pi_{(0,19)} 2_6^2 4^2 8_5^{-1} 3^1$         | $\Pi_{(3,2)} 2_6^{-2} 4^{-2} 8_7^1$   | —    | —        | 128        |
| 17F1.21  | 32    | [32, 28]                                   | $\Pi_{(0,19)} 2_6^2 4^2 8_5^{-1} 3^1$         | $\Pi_{(3,2)} 2_6^{-2} 4^{-2} 8_7^1$   | —    | —        | 64         |
| 17F1.22  | 32    | $C_2^2 \wr C_2 \mid [32, 27]$              | $\Pi_{(0,19)} 2_6^2 4^2 8_5^{-1} 3^1$         | $\Pi_{(3,2)} 2_6^{-2} 4^{-2} 8_7^1$   | —    | —        | 64         |
| 17F1.23  | 32    | [32, 30]                                   | $\Pi_{(0,19)} 2_4^{-2} 4_0^2 8_7^1 3^1$       | $\Pi_{(3,2)} 2_4^{-2} 4_0^2 8_5^{-1}$ | —    | —        | 64         |
| 17F1.24  | 32    | $C_2^2 \wr C_2 \mid [32, 27]$              | $\Pi_{(0,19)} 2_4^{-2} 4_0^2 8_7^1 3^1$       | $\Pi_{(3,2)} 2_4^{-2} 4_0^2 8_5^{-1}$ | —    | —        | 64         |
| 17F1.25  | 32    | $\text{Aut}(D_{16}) \mid [32, 43]$         | $\Pi_{(0,19)} 2_3^3 8^{-2} 3^1$               | $\Pi_{(3,2)} 2_1^3 8^{-2}$            | —    | —        | —          |
| 17F1.26  | 32    | $C_2 \times D_{16} \mid [32, 39]$          | $\Pi_{(0,19)} 2_3^{-3} 8^2 3^1$               | $\Pi_{(3,2)} 2_1^3 8^2$               | —    | —        | —          |
| 17F1.27  | 32    | $\Gamma_{7a_2} \mid [32, 7]$               | $\Pi_{(0,19)} 4_7^1 8_4^{-2} 3^1$             | $\Pi_{(3,2)} 4_3^{-1} 8_6^2$          | —    | —        | 128        |
| 17F1.28  | 32    | $C_2^2 \times D_8 \mid [32, 46]$           | $\Pi_{(0,19)} 2_4^{-2} 4_7^3 3^1$             | $\Pi_{(3,2)} 2_0^2 4_1^3$             | —    | —        | 128        |
| 17F1.29  | 32    | $2_+^{1+4} \mid [32, 49]$                  | $\Pi_{(0,19)} 2_4^{-2} 4_7^3 3^1$             | $\Pi_{(3,2)} 2_0^2 4_1^3$             | —    | —        | 128        |
| 17F1.30  | 32    | $2_+^{1+4} \mid [32, 49]$                  | $\Pi_{(0,19)} 2_6^{-2} 4_5^{-3} 3^1$          | $\Pi_{(3,2)} 2_0^2 4_1^3$             | —    | —        | 128        |
| 17F1.31  | 32    | $2_+^{1+4} \mid [32, 49]$                  | $\Pi_{(0,19)} 2_4^{-2} 4_7^3 3^1$             | $\Pi_{(3,2)} 2_0^2 4_1^3$             | —    | —        | 128        |
| 17F1.32  | 32    | [32, 30]                                   | $\Pi_{(0,19)} 4_6^2 8_5^{-1} 3^1$             | $\Pi_{(3,2)} 4_0^2 8_5^{-1}$          | —    | —        | 384        |
| 17F1.33  | 32    | [32, 28]                                   | $\Pi_{(0,19)} 4_6^2 8_5^{-1} 3^1$             | $\Pi_{(3,2)} 4_0^2 8_5^{-1}$          | —    | —        | 384        |
| 17F1.34  | 32    | $2_+^{1+4} \mid [32, 49]$                  | $\Pi_{(0,19)} 4_7^{-3} 3^1$                   | $\Pi_{(3,2)} 4_1^{-3}$                | —    | —        | 384        |
| 17F1.35  | 32    | $C_2^2 \times D_8 \mid [32, 46]$           | $\Pi_{(0,18)} 4_0^{-4} 3^1$                   | $\Pi_{(3,3)} 4_0^{-4}$                | —    | —        | 96         |

Table 2: Birational symplectic effective  $\chi$ -saturated groups

| $(X, G)$ | $\#G$ | Description of $G$                       | $g(\Lambda_G)$                                | $g(\Lambda^G)$                            | K3   | Cubic | Saturation |
|----------|-------|------------------------------------------|-----------------------------------------------|-------------------------------------------|------|-------|------------|
| 17F1.36  | 32    | $C_2^2 \wr C_2 \mid [32, 27]$            | $\Pi_{(0,18)} 4_0^{-4} 3^1$                   | $\Pi_{(3,3)} 4_0^{-4}$                    | —    | —     | 96         |
| 17F1.37  | 32    | $C_2^2 \times D_8 \mid [32, 46]$         | $\Pi_{(0,18)} 2_4^4 4_4^{-2} 3^1$             | $\Pi_{(3,3)} 2_0^4 4_0^2$                 | —    | —     | 96         |
| 17F1.38  | 32    | $C_2^2 \times D_8 \mid [32, 46]$         | $\Pi_{(0,18)} 2_4^{-2} 4_0^4 3^1$             | $\Pi_{(3,3)} 2_0^2 4_0^4$                 | —    | —     | —          |
| 17F1.39  | 32    | [32, 28]                                 | $\Pi_{(0,18)} 2_0^2 4_0^4 3^1$                | $\Pi_{(3,3)} 2_0^2 4_0^4$                 | —    | —     | —          |
| 17F1.40  | 32    | $2_+^{1+4} \mid [32, 49]$                | $\Pi_{(0,18)} 2_4^{-2} 4_0^4 3^1$             | $\Pi_{(3,3)} 2_0^2 4_0^4$                 | —    | —     | —          |
| 17F1.41  | 32    | $C_2 \times C_4 \circ D_8 \mid [32, 48]$ | $\Pi_{(0,18)} 2^{-2} 4_4^{-4} 3^1$            | $\Pi_{(3,3)} 2^2 4_0^4$                   | —    | —     | —          |
| 17F1.42  | 32    | $C_2^3 \rtimes C_4 \mid [32, 6]$         | $\Pi_{(0,18)} 4_7^3 8_5^{-1} 3^1$             | $\Pi_{(3,3)} 4_1^{-3} 8_7^1$              | —    | —     | 64         |
| 17F1.43  | 32    | [32, 34]                                 | $\Pi_{(0,18)} 2^2 8_4^{-2} 3^1$               | $\Pi_{(3,3)} 2^2 8_4^{-2}$                | —    | —     | 64         |
| 17F1.44  | 32    | [32, 28]                                 | $\Pi_{(0,18)} 2^2 8_4^{-2} 3^1$               | $\Pi_{(3,3)} 2^2 8_4^{-2}$                | —    | —     | 64         |
| 17F1.45  | 32    | $C_2^2 \wr C_2 \mid [32, 27]$            | $\Pi_{(0,17)} 2^{-2} 4_4^{-2} 8_5^{-1} 3^1$   | $\Pi_{(3,4)} 2^{-2} 4_4^{-2} 8_3^{-1}$    | —    | —     | —          |
| 17F1.46  | 32    | $C_2^2 \times D_8 \mid [32, 46]$         | $\Pi_{(0,17)} 2^{-2} 4_6^{-2} 8_3^{-1} 3^1$   | $\Pi_{(3,4)} 2^{-2} 4_4^{-2} 8_3^{-1}$    | —    | —     | —          |
| 18C1     | 12    | $D_{12} \mid [12, 4]$                    | $\Pi_{(0,16)} 2^4 3^4$                        | $\Pi_{(3,5)} 2^4 3^{-3}$                  | —    | ×     | 24         |
| 18C1.1   | 24    | $C_3 \rtimes D_8 \mid [24, 8]$           | $\Pi_{(0,20)} 2_6^{-2} 4_2^2 3^3$             | $\Pi_{(3,1)} 2_6^2 4_2^2 3^2$             | —    | —     | 48         |
| 18C1.2   | 24    | $C_2^2 \times S_3 \mid [24, 14]$         | $\Pi_{(0,20)} 2_4^{-2} 4_4^{-2} 3^{-2}$       | $\Pi_{(3,1)} 2_0^2 4_4^{-2} 3^1$          | —    | —     | 48         |
| 18C1.3   | 24    | $C_3 \rtimes D_8 \mid [24, 8]$           | $\Pi_{(0,20)} 2_2^{-2} 4_2^2 3^1$             | $\Pi_{(3,1)} 2_6^{-2} 4^{-2}$             | —    | —     | 768        |
| 18C1.4   | 24    | $D_{24} \mid [24, 6]$                    | $\Pi_{(0,18)} 4^{-2} 3^{-3}$                  | $\Pi_{(3,3)} 4^{-2} 3^{-2}$               | —    | ×     | 144        |
| 18C1.5   | 24    | $C_2^2 \times S_3 \mid [24, 14]$         | $\Pi_{(0,16)} 2^4 3^4$                        | $\Pi_{(3,5)} 2^4 3^{-3}$                  | —    | ×     | —          |
| 18F1     | 12    | $D_{12} \mid [12, 4]$                    | $\Pi_{(0,16)} 2^4 3^4$                        | $\Pi_{(3,5)} 2^4 3^5$                     | (18) | ×     | —          |
| 18F1.1   | 24    | $C_2^2 \times S_3 \mid [24, 14]$         | $\Pi_{(0,20)} 2_0^2 4_4^{-2} 3^4$             | $\Pi_{(3,1)} 2_0^2 4_4^{-2} 3^{-3}$       | —    | —     | —          |
| 18F1.2   | 24    | $D_{24} \mid [24, 6]$                    | $\Pi_{(0,20)} 2_2^{-2} 4_2^2 3^{-3}$          | $\Pi_{(3,1)} 2_6^{-2} 4^{-2} 3^{-2}$      | —    | —     | —          |
| 18F1.3   | 24    | $C_2^2 \times S_3 \mid [24, 14]$         | $\Pi_{(0,19)} 2_0^4 4_7^1 3^{-3}$             | $\Pi_{(3,2)} 2_0^4 4_1^1 3^{-2}$          | —    | —     | —          |
| 18F1.4   | 24    | $C_3 \rtimes D_8 \mid [24, 8]$           | $\Pi_{(0,18)} 4^{-2} 3^5$                     | $\Pi_{(3,3)} 4^{-2} 3^4$                  | —    | ×     | —          |
| 18F1.5   | 24    | $C_2^2 \times S_3 \mid [24, 14]$         | $\Pi_{(0,18)} 4_2^2 3^{-4}$                   | $\Pi_{(3,3)} 4_6^2 3^3$                   | —    | ×     | —          |
| 19C1     | 12    | $A_4 \mid [12, 3]$                       | $\Pi_{(0,16)} 2^{-2} 4^{-2} 3^2$              | $\Pi_{(3,5)} 2^{-2} 4^{-2} 3^{-1}$        | —    | ×     | 24         |
| 19C1.1   | 24    | $C_2 \times A_4 \mid [24, 13]$           | $\Pi_{(0,21)} 2_6^2 8_3^{-1} 3^1$             | $\Pi_{(3,0)} 2_6^{-2} 8_5^{-1}$           | —    | —     | 23040      |
| 19C1.2   | 24    | $S_4 \mid [24, 12]$                      | $\Pi_{(0,20)} 2_6^{-2} 4_3^{-1} 8_5^{-1} 3^1$ | $\Pi_{(3,1)} 2_4^{-2} 4_1^1 8_5^{-1}$     | —    | —     | 96         |
| 19C1.3   | 24    | $C_2 \times A_4 \mid [24, 13]$           | $\Pi_{(0,19)} 2_2^{-4} 8_1^1 3^1$             | $\Pi_{(3,2)} 2_6^{-4} 8_3^{-1}$           | —    | —     | 48         |
| 19C1.4   | 24    | $S_4 \mid [24, 12]$                      | $\Pi_{(0,18)} 2^{-2} 4_6^{-2} 3^2$            | $\Pi_{(3,3)} 2^2 4_6^2 3^{-1}$            | —    | —     | 96         |
| 19C1.5   | 24    | $C_2 \times A_4 \mid [24, 13]$           | $\Pi_{(0,17)} 4_3^3 3^2$                      | $\Pi_{(3,4)} 4_5^3 3^{-1}$                | —    | ×     | 48         |
| 19C1.6   | 24    | $S_4 \mid [24, 12]$                      | $\Pi_{(0,16)} 2^{-2} 4^{-2} 3^2$              | $\Pi_{(3,5)} 2^{-2} 4^{-2} 3^{-1}$        | —    | ×     | —          |
| 19F1     | 12    | $A_4 \mid [12, 3]$                       | $\Pi_{(0,16)} 2^{-2} 4^{-2} 3^2$              | $\Pi_{(3,5)} 2^{-2} 4^{-2} 3^3$           | (17) | ×     | —          |
| 19F1.1   | 24    | $C_2 \times A_4 \mid [24, 13]$           | $\Pi_{(0,21)} 2_2^2 8_1^1 3^{-2}$             | $\Pi_{(3,0)} 2_6^2 8_3^{-1} 3^1$          | —    | —     | 288        |
| 19F1.2   | 24    | $C_2 \times A_4 \mid [24, 13]$           | $\Pi_{(0,21)} 2_6^2 4_1^1 3^2$                | $\Pi_{(3,0)} 2_4^{-2} 4_1^1 3^{-1}$       | —    | —     | 1440       |
| 19F1.3   | 24    | $C_2 \times A_4 \mid [24, 13]$           | $\Pi_{(0,21)} 2_2^{-2} 8_3^{-1} 3^1$          | $\Pi_{(3,0)} 2_6^{-2} 8_5^{-1}$           | —    | —     | 23040      |
| 19F1.4   | 24    | $S_4 \mid [24, 12]$                      | $\Pi_{(0,20)} 2_6^{-2} 4_3^{-1} 8_5^{-1} 3^1$ | $\Pi_{(3,1)} 2_4^{-2} 4_1^1 8_5^{-1}$     | —    | —     | 768        |
| 19F1.5   | 24    | $S_4 \mid [24, 12]$                      | $\Pi_{(0,20)} 2_0^2 4_0^2 3^2$                | $\Pi_{(3,1)} 2_4^{-2} 4_0^2 3^{-1}$       | —    | —     | 48         |
| 19F1.6   | 24    | $C_2 \times A_4 \mid [24, 13]$           | $\Pi_{(0,20)} 2_0^2 4_4^{-2} 3^{-2}$          | $\Pi_{(3,1)} 2_0^2 4_4^{-2} 3^1$          | —    | —     | 384        |
| 19F1.7   | 24    | $C_2 \times A_4 \mid [24, 13]$           | $\Pi_{(0,20)} 2_0^2 4_7^1 8_5^{-1} 3^2$       | $\Pi_{(3,1)} 2_6^2 4_1^1 8_5^{-1} 3^{-1}$ | —    | —     | 48         |



Table 2: Birational symplectic effective  $\chi$ -saturated groups

| $(X, G)$ | $\#G$ | Description of $G$             | $g(\Lambda_G)$                                | $g(\Lambda^G)$                               | K3   | Cubic    | Saturation |
|----------|-------|--------------------------------|-----------------------------------------------|----------------------------------------------|------|----------|------------|
| 19F1.8   | 24    | $S_4 \mid [24, 12]$            | $\Pi_{(0,20)} 2_4^{-2} 4_5^{-1} 8_7^1 3^{-2}$ | $\Pi_{(3,1)} 2_4^{-2} 4_3^{-1} 8_5^{-1} 3^1$ | —    | —        | —          |
| 19F1.9   | 24    | $S_4 \mid [24, 12]$            | $\Pi_{(0,19)} 2_6^{-4} 8_3^{-1} 3^2$          | $\Pi_{(3,2)} 2_2^{-4} 8_1^1 3^{-1}$          | —    | —        | —          |
| 19F1.10  | 24    | $S_4 \mid [24, 12]$            | $\Pi_{(0,19)} 2_6^{-4} 4_3^{-1} 3^{-2}$       | $\Pi_{(3,2)} 2_0^4 4_3^{-1} 3^1$             | —    | —        | 192        |
| 19F1.11  | 24    | $C_2 \times A_4 \mid [24, 13]$ | $\Pi_{(0,19)} 2^{-2} 8_7^1 3^3$               | $\Pi_{(3,2)} 2^{-2} 8_1^1 3^2$               | —    | —        | 96         |
| 19F1.12  | 24    | $S_4 \mid [24, 12]$            | $\Pi_{(0,19)} 4_5^3 3^{-2}$                   | $\Pi_{(3,2)} 4_3^3 3^1$                      | —    | —        | 192        |
| 19F1.13  | 24    | $S_4 \mid [24, 12]$            | $\Pi_{(0,18)} 4_3^{-1} 8_1^1 3^3$             | $\Pi_{(3,3)} 4_5^{-1} 8_7^1 3^2$             | —    | $\times$ | 48         |
| 19F1.14  | 24    | $C_2 \times A_4 \mid [24, 13]$ | $\Pi_{(0,18)} 2^{-2} 4_2^{-2} 3^{-2}$         | $\Pi_{(3,3)} 2^2 4_2^2 3^1$                  | —    | —        | 96         |
| 19F1.15  | 24    | $C_2 \times A_4 \mid [24, 13]$ | $\Pi_{(0,17)} 2^{-2} 8_1^1 3^3$               | $\Pi_{(3,4)} 2^{-2} 8_7^1 3^2$               | —    | $\times$ | —          |
| 20F1     | 10    | $D_{10} \mid [10, 1]$          | $\Pi_{(0,16)} 5^4$                            | $\Pi_{(3,5)} 3^1 5^4$                        | (16) | $\times$ | —          |
| 20F1.1   | 20    | $D_{20} \mid [20, 4]$          | $\Pi_{(0,20)} 2_6^4 3^1 5^2$                  | $\Pi_{(3,1)} 2_2^4 5^2$                      | —    | —        | —          |
| 20F1.2   | 20    | $F_5 \mid [20, 3]$             | $\Pi_{(0,20)} 2_2^4 3^1 5^{-2}$               | $\Pi_{(3,1)} 2_6^4 5^{-2}$                   | —    | —        | 40         |
| 20F1.3   | 20    | $F_5 \mid [20, 3]$             | $\Pi_{(0,20)} 2_2^4 3^1 5^1$                  | $\Pi_{(3,1)} 2_2^{-4} 5^1$                   | —    | —        | 120        |
| 20F1.4   | 20    | $D_{20} \mid [20, 4]$          | $\Pi_{(0,20)} 2_6^4 3^1 5^{-1}$               | $\Pi_{(3,1)} 2_6^{-4} 5^{-1}$                | —    | —        | 240        |
| 20F1.5   | 20    | $D_{20} \mid [20, 4]$          | $\Pi_{(0,18)} 2^2 3^1 5^{-3}$                 | $\Pi_{(3,3)} 2^2 5^{-3}$                     | —    | $\times$ | —          |
| 20F1.6   | 20    | $F_5 \mid [20, 3]$             | $\Pi_{(0,18)} 2^{-2} 3^1 5^{-2}$              | $\Pi_{(3,3)} 2^{-2} 5^{-2}$                  | —    | $\times$ | 120        |
| 22C1     | 6     | $S_3 \mid [6, 1]$              | $\Pi_{(0,16)} 3^8$                            | $\Pi_{(3,5)} 3^{-7}$                         | —    | —        | —          |
| 23F1     | 4     | $C_2^2 \mid [4, 2]$            | $\Pi_{(0,16)} 2_0^{-4} 4_4^{-4}$              | $\Pi_{(3,5)} 2_6^{-4} 4_6^4 3^1$             | —    | —        | —          |
| 23F1.1   | 8     | $D_8 \mid [8, 3]$              | $\Pi_{(0,21)} 2_2^{-2} 8_7^1 3^1$             | $\Pi_{(3,0)} 2_6^{-2} 8_5^{-1}$              | —    | —        | 23040      |
| 23F1.2   | 8     | $C_2^3 \mid [8, 5]$            | $\Pi_{(0,21)} 2_2^{-2} 8_3^{-1} 3^1$          | $\Pi_{(3,0)} 2_6^{-2} 8_5^{-1}$              | —    | —        | 23040      |
| 23F1.3   | 8     | $C_2 \times C_4 \mid [8, 2]$   | $\Pi_{(0,20)} 4_6^{-2} 8_4^{-2} 3^1$          | $\Pi_{(3,1)} 4_0^2 8_2^2$                    | —    | —        | —          |
| 23F1.4   | 8     | $D_8 \mid [8, 3]$              | $\Pi_{(0,20)} 2_7^4 4_1^8 3^1$                | $\Pi_{(3,1)} 2_1^4 4_1^8 2$                  | —    | —        | 32         |
| 23F1.5   | 8     | $C_2^3 \mid [8, 5]$            | $\Pi_{(0,20)} 4_7^3 8_7^1 3^1$                | $\Pi_{(3,1)} 4_1^3 8_1^1$                    | —    | —        | 32         |
| 23F1.6   | 8     | $D_8 \mid [8, 3]$              | $\Pi_{(0,20)} 4_5^{-3} 8_5^{-1} 3^1$          | $\Pi_{(3,1)} 4_1^3 8_1^1$                    | —    | —        | 32         |
| 23F1.7   | 8     | $D_8 \mid [8, 3]$              | $\Pi_{(0,20)} 2_6^2 8_4^{-2} 3^1$             | $\Pi_{(3,1)} 2_2^2 8_0^2$                    | —    | —        | 64         |
| 23F1.8   | 8     | $C_2 \times C_4 \mid [8, 2]$   | $\Pi_{(0,20)} 2^{-2} 8_6^{-2} 3^1$            | $\Pi_{(3,1)} 2^{-2} 8_2^{-2}$                | —    | —        | 64         |
| 23F1.9   | 8     | $C_2^3 \mid [8, 5]$            | $\Pi_{(0,20)} 4_6^4 3^1$                      | $\Pi_{(3,1)} 4_2^4$                          | —    | —        | —          |
| 23F1.10  | 8     | $C_2^3 \mid [8, 5]$            | $\Pi_{(0,20)} 2_0^2 4_1^8 7^1 3^1$            | $\Pi_{(3,1)} 2_4^{-2} 4_1^8 5^{-1}$          | —    | —        | 96         |
| 23F1.11  | 8     | $C_2^3 \mid [8, 5]$            | $\Pi_{(0,20)} 2_2^{-2} 4_2^2 3^1$             | $\Pi_{(3,1)} 2_6^{-2} 4^{-2}$                | —    | —        | 768        |
| 23F1.12  | 8     | $C_2^3 \mid [8, 5]$            | $\Pi_{(0,20)} 2_2^{-2} 4_2^2 3^1$             | $\Pi_{(3,1)} 2_6^{-2} 4^{-2}$                | —    | —        | 768        |
| 23F1.13  | 8     | $D_8 \mid [8, 3]$              | $\Pi_{(0,19)} 2_2^{-2} 4_3^{-1} 8_6^2 3^1$    | $\Pi_{(3,2)} 2_2^2 4_1^1 8_2^2$              | —    | —        | 16         |
| 23F1.14  | 8     | $D_8 \mid [8, 3]$              | $\Pi_{(0,19)} 2_6^2 4_1^8 2_2^2 3^1$          | $\Pi_{(3,2)} 2_6^2 4_1^8 2_2^2$              | —    | —        | 16         |
| 23F1.15  | 8     | $C_2 \times C_4 \mid [8, 2]$   | $\Pi_{(0,19)} 2_6^{-2} 4_5^{-1} 8_4^{-2} 3^1$ | $\Pi_{(3,2)} 2_6^2 4_1^8 2_2^2$              | —    | —        | 16         |
| 23F1.16  | 8     | $C_2^3 \mid [8, 5]$            | $\Pi_{(0,19)} 4_7^5 3^1$                      | $\Pi_{(3,2)} 4_1^5$                          | —    | —        | —          |
| 23F1.17  | 8     | $C_2^3 \mid [8, 5]$            | $\Pi_{(0,19)} 4_7^5 3^1$                      | $\Pi_{(3,2)} 4_1^5$                          | —    | —        | 16         |
| 23F1.18  | 8     | $C_2^3 \mid [8, 5]$            | $\Pi_{(0,19)} 2_2^{-2} 4_2^2 8_1^1 3^1$       | $\Pi_{(3,2)} 2_6^{-2} 4^{-2} 8_7^1$          | —    | —        | 64         |
| 23F1.19  | 8     | $C_2^3 \mid [8, 5]$            | $\Pi_{(0,19)} 2_2^{-2} 4_0^2 8_5^{-1} 3^1$    | $\Pi_{(3,2)} 2_4^{-2} 4_0^2 8_5^{-1}$        | —    | —        | 16         |
| 23F1.20  | 8     | $D_8 \mid [8, 3]$              | $\Pi_{(0,19)} 2_3^3 8^{-2} 3^1$               | $\Pi_{(3,2)} 2_1^{-3} 8^{-2}$                | —    | —        | 16         |
| 23F1.21  | 8     | $D_8 \mid [8, 3]$              | $\Pi_{(0,19)} 2_2^{-2} 4_2^2 8_1^1 3^1$       | $\Pi_{(3,2)} 2_6^{-2} 4^{-2} 8_7^1$          | —    | —        | 64         |

Table 2: Birational symplectic effective  $\chi$ -saturated groups

| $(X, G)$ | $\#G$ | Description of $G$                            | $g(\Lambda_G)$                             | $g(\Lambda^G)$                        | K3   | Cubic | Saturation |
|----------|-------|-----------------------------------------------|--------------------------------------------|---------------------------------------|------|-------|------------|
| 23F1.22  | 8     | $C_2^3 \mid [8, 5]$                           | $\Pi_{(0,19)} 2_6^{-2} 4_5^3 3^1$          | $\Pi_{(3,2)} 2_0^2 4_1^3$             | —    | —     | 16         |
| 23F1.23  | 8     | $D_8 \mid [8, 3]$                             | $\Pi_{(0,19)} 2_2^{-4} 8_1^1 3^1$          | $\Pi_{(3,2)} 2_6^{-4} 8_3^{-1}$       | —    | —     | 48         |
| 23F1.24  | 8     | $C_2^3 \mid [8, 5]$                           | $\Pi_{(0,19)} 4_6^4 8_1^1 3^1$             | $\Pi_{(3,2)} 4_0^4 8_1^1$             | —    | —     | —          |
| 23F1.25  | 8     | $C_2^3 \mid [8, 5]$                           | $\Pi_{(0,18)} 2_6^2 4_3^{-3} 8_7^1 3^1$    | $\Pi_{(3,3)} 2_2^{-2} 4_1^3 8_5^{-1}$ | —    | —     | —          |
| 23F1.26  | 8     | $D_8 \mid [8, 3]$                             | $\Pi_{(0,18)} 2_2^{-4} 8_2^2 3^1$          | $\Pi_{(3,3)} 2_2^4 8_6^2$             | —    | —     | 16         |
| 23F1.27  | 8     | $C_2^3 \mid [8, 5]$                           | $\Pi_{(0,18)} 2_2^2 4_6^{-4} 3^1$          | $\Pi_{(3,3)} 2_0^2 4_0^4$             | —    | —     | 16         |
| 23F1.28  | 8     | $C_2^3 \mid [8, 5]$                           | $\Pi_{(0,18)} 2^2 4_0^4 3^1$               | $\Pi_{(3,3)} 2^2 4_0^4$               | —    | —     | 16         |
| 23F1.29  | 8     | $C_2^3 \mid [8, 5]$                           | $\Pi_{(0,18)} 2^2 4_0^4 3^1$               | $\Pi_{(3,3)} 2^2 4_0^4$               | —    | —     | —          |
| 23F1.30  | 8     | $C_2^3 \mid [8, 5]$                           | $\Pi_{(0,18)} 2_2^{-4} 4_2^2 3^1$          | $\Pi_{(3,3)} 2_0^4 4_0^2$             | —    | —     | —          |
| 23F1.31  | 8     | $C_2^3 \mid [8, 5]$                           | $\Pi_{(0,17)} 2_6^4 4_2^{-2} 8_1^1 3^1$    | $\Pi_{(3,4)} 2_0^{-4} 4_4^{-2} 8_7^1$ | —    | —     | —          |
| 23F1.32  | 8     | $D_8 \mid [8, 3]$                             | $\Pi_{(0,17)} 2_6^{-4} 4_2^2 8_7^1 3^1$    | $\Pi_{(3,4)} 2_6^4 4_2^2 8_1^1$       | —    | —     | —          |
| 24F1     | 48    | $C_2^2 \rtimes A_4 \mid [48, 50]$             | $\Pi_{(0,17)} 2^{-4} 8_1^1 3^{-1}$         | $\Pi_{(3,4)} 2^{-4} 8_7^1 3^2$        | (49) | —     | —          |
| 24F1.1   | 96    | $C_2 \times C_2^2 \rtimes A_4 \mid [96, 229]$ | $\Pi_{(0,21)} 2_2^{-2} 8_3^{-1} 3^1$       | $\Pi_{(3,0)} 2_6^{-2} 8_5^{-1}$       | —    | —     | 23040      |
| 24F1.2   | 96    | $[96, 70]$                                    | $\Pi_{(0,20)} 2_0^2 4_4^{-2} 3^{-2}$       | $\Pi_{(3,1)} 2_0^2 4_4^{-2} 3^1$      | —    | —     | 384        |
| 24F1.3   | 96    | $C_2^2 \rtimes S_4 \mid [96, 227]$            | $\Pi_{(0,20)} 2_2^2 4_7^1 8_3^{-1} 3^1$    | $\Pi_{(3,1)} 2_4^{-2} 4_1^1 8_5^{-1}$ | —    | —     | 768        |
| 24F1.4   | 96    | $C_2^2 \rtimes S_4 \mid [96, 227]$            | $\Pi_{(0,20)} 4_5^{-1} 8_1^1 3^1$          | $\Pi_{(3,1)} 4_1^1 8_5^{-1}$          | —    | —     | 11520      |
| 24F1.5   | 96    | $C_2^2 \rtimes S_4 \mid [96, 227]$            | $\Pi_{(0,19)} 4_5^3 3^{-2}$                | $\Pi_{(3,2)} 4_3^3 3^1$               | —    | —     | 192        |
| 24F1.6   | 96    | $C_2^2 \rtimes S_4 \mid [96, 227]$            | $\Pi_{(0,19)} 2_4^{-4} 4_5^{-1} 3^{-2}$    | $\Pi_{(3,2)} 2_0^4 4_3^{-1} 3^1$      | —    | —     | 192        |
| 24F1.7   | 96    | $[96, 70]$                                    | $\Pi_{(0,19)} 4_6^{-2} 8_1^1 3^1$          | $\Pi_{(3,2)} 4_0^2 8_5^{-1}$          | —    | —     | 384        |
| 24F1.8   | 96    | $C_2 \times C_2^2 \rtimes A_4 \mid [96, 229]$ | $\Pi_{(0,18)} 2^2 4_6^2 3^{-2}$            | $\Pi_{(3,3)} 2^2 4_2^2 3^1$           | —    | —     | —          |
| 26F1     | 32    | $C_2^2 \wr C_2 \mid [32, 27]$                 | $\Pi_{(0,17)} 2^2 4_6^2 8_1^1$             | $\Pi_{(3,4)} 2^2 4_2^2 8_7^1 3^1$     | (39) | —     | —          |
| 26F1.1   | 64    | $D_8^2 \mid [64, 226]$                        | $\Pi_{(0,21)} 2_6^2 8_7^1 3^1$             | $\Pi_{(3,0)} 2_6^{-2} 8_5^{-1}$       | —    | —     | 23040      |
| 26F1.2   | 64    | $C_2 \times C_2^2 \wr C_2 \mid [96, 227]$     | $\Pi_{(0,21)} 2_6^2 8_7^1 3^1$             | $\Pi_{(3,0)} 2_6^{-2} 8_5^{-1}$       | —    | —     | 23040      |
| 26F1.3   | 64    | $C_2 \times C_2^2 \wr C_2 \mid [96, 227]$     | $\Pi_{(0,21)} 2_2^{-2} 8_7^1 3^1$          | $\Pi_{(3,0)} 2_6^{-2} 8_5^{-1}$       | —    | —     | 23040      |
| 26F1.4   | 64    | $[64, 241]$                                   | $\Pi_{(0,20)} 2_2^{-2} 8_4^{-2} 3^1$       | $\Pi_{(3,1)} 2_2^2 8_0^2$             | —    | —     | 256        |
| 26F1.5   | 64    | $\text{ASL}(\mathbb{F}_{16}) \mid [64, 32]$   | $\Pi_{(0,20)} 2_0^2 4_5^{-1} 8_5^{-1} 3^1$ | $\Pi_{(3,1)} 2_4^{-2} 4_1^1 8_5^{-1}$ | —    | —     | 768        |
| 26F1.6   | 64    | $\Gamma_{25} a_1 \mid [64, 138]$              | $\Pi_{(0,20)} 2_0^2 4_7^1 8_3^{-1} 3^1$    | $\Pi_{(3,1)} 2_4^{-2} 4_1^1 8_5^{-1}$ | —    | —     | 768        |
| 26F1.7   | 64    | $\Gamma_{25} a_1 \mid [64, 138]$              | $\Pi_{(0,20)} 2_0^2 4_7^1 8_7^1 3^1$       | $\Pi_{(3,1)} 2_4^{-2} 4_1^1 8_5^{-1}$ | —    | —     | 768        |
| 26F1.8   | 64    | $[64, 215]$                                   | $\Pi_{(0,20)} 2_6^2 4^2 3^1$               | $\Pi_{(3,1)} 2_6^{-2} 4^{-2}$         | —    | —     | 768        |
| 26F1.9   | 64    | $[64, 215]$                                   | $\Pi_{(0,20)} 2_2^{-2} 4^2 3^1$            | $\Pi_{(3,1)} 2_6^{-2} 4^{-2}$         | —    | —     | 768        |
| 26F1.10  | 64    | $\text{ASL}(\mathbb{F}_{16}) \mid [64, 32]$   | $\Pi_{(0,20)} 4_7^1 8_3^{-1} 3^1$          | $\Pi_{(3,1)} 4_1^1 8_5^{-1}$          | —    | —     | 11520      |
| 26F1.11  | 64    | $\Gamma_{25} a_1 \mid [64, 138]$              | $\Pi_{(0,20)} 4_5^{-1} 8_1^1 3^1$          | $\Pi_{(3,1)} 4_1^1 8_5^{-1}$          | —    | —     | 11520      |
| 26F1.12  | 64    | $\Gamma_{25} a_1 \mid [64, 138]$              | $\Pi_{(0,19)} 4_7^{-3} 3^1$                | $\Pi_{(3,2)} 4_1^{-3}$                | —    | —     | 384        |
| 26F1.13  | 64    | $[64, 215]$                                   | $\Pi_{(0,19)} 2_0^2 4_0^2 8_7^1 3^1$       | $\Pi_{(3,2)} 2_4^{-2} 4_0^2 8_5^{-1}$ | —    | —     | —          |
| 26F1.14  | 64    | $\text{ASL}(\mathbb{F}_{16}) \mid [64, 32]$   | $\Pi_{(0,19)} 4_7^1 8_4^{-2} 3^1$          | $\Pi_{(3,2)} 4_3^{-1} 8_6^2$          | —    | —     | 128        |
| 26F1.15  | 64    | $\Gamma_{25} a_1 \mid [64, 138]$              | $\Pi_{(0,19)} 2_4^{-2} 4_7^3 3^1$          | $\Pi_{(3,2)} 2_0^2 4_1^3$             | —    | —     | 128        |
| 26F1.16  | 64    | $\Gamma_{25} a_1 \mid [64, 138]$              | $\Pi_{(0,19)} 2_0^2 4_7^3 3^1$             | $\Pi_{(3,2)} 2_0^2 4_1^3$             | —    | —     | 128        |
| 26F1.17  | 64    | $[64, 241]$                                   | $\Pi_{(0,19)} 4_6^2 8_5^{-1} 3^1$          | $\Pi_{(3,2)} 4_0^2 8_5^{-1}$          | —    | —     | 384        |

Table 2: Birational symplectic effective  $\chi$ -saturated groups

| $(X, G)$ | $\#G$ | Description of $G$                        | $g(\Lambda_G)$                          | $g(\Lambda^G)$                        | K3   | Cubic    | Saturation |
|----------|-------|-------------------------------------------|-----------------------------------------|---------------------------------------|------|----------|------------|
| 26F1.18  | 64    | [64, 215]                                 | $\Pi_{(0,19)}4_6^28_5^{-1}3^1$          | $\Pi_{(3,2)}4_0^28_5^{-1}$            | —    | —        | 384        |
| 26F1.19  | 64    | $D_8^2 \mid [64, 226]$                    | $\Pi_{(0,18)}2_6^28_4^{-2}3^1$          | $\Pi_{(3,3)}2^28_4^{-2}$              | —    | —        | —          |
| 26F1.20  | 64    | $C_2 \times C_2^2 \wr C_2 \mid [96, 227]$ | $\Pi_{(0,18)}4_0^{-4}3^1$               | $\Pi_{(3,3)}4_0^{-4}$                 | —    | —        | —          |
| 26F1.21  | 64    | $C_2 \times C_2^2 \wr C_2 \mid [96, 227]$ | $\Pi_{(0,18)}2_4^{-4}4_0^23^1$          | $\Pi_{(3,3)}2_0^44_0^2$               | —    | —        | —          |
| 28F1     | 32    | $2_+^{1+4} \mid [32, 49]$                 | $\Pi_{(0,17)}4_7^5$                     | $\Pi_{(3,4)}4_1^53^1$                 | (40) | —        | —          |
| 28F1.1   | 64    | $\Gamma_{25}a_1 \mid [64, 138]$           | $\Pi_{(0,21)}2_6^28_3^{-1}3^1$          | $\Pi_{(3,0)}2_6^{-2}8_5^{-1}$         | —    | —        | 23040      |
| 28F1.2   | 64    | $\Gamma_{25}a_1 \mid [64, 138]$           | $\Pi_{(0,21)}2_2^{-2}8_7^13^1$          | $\Pi_{(3,0)}2_6^{-2}8_5^{-1}$         | —    | —        | 23040      |
| 28F1.3   | 64    | $C_2 \times 2_+^{1+4} \mid [64, 264]$     | $\Pi_{(0,20)}2_6^24^{-2}3^1$            | $\Pi_{(3,1)}2_6^{-2}4^{-2}$           | —    | —        | 768        |
| 28F1.4   | 64    | $C_2 \times 2_+^{1+4} \mid [64, 264]$     | $\Pi_{(0,20)}2_2^{-2}4^23^1$            | $\Pi_{(3,1)}2_6^{-2}4^{-2}$           | —    | —        | 768        |
| 28F1.5   | 64    | [64, 139]                                 | $\Pi_{(0,20)}4_7^18_3^{-1}3^1$          | $\Pi_{(3,1)}4_1^18_5^{-1}$            | —    | —        | 11520      |
| 28F1.6   | 64    | $D_8 \circ D_{16} \mid [64, 257]$         | $\Pi_{(0,20)}2_3^{-1}4_3^{-1}8^{-2}3^1$ | $\Pi_{(3,1)}2_1^14_1^18^2$            | —    | —        | —          |
| 28F1.7   | 64    | [64, 134]                                 | $\Pi_{(0,20)}2_6^28_4^{-2}3^1$          | $\Pi_{(3,1)}2_2^28_0^2$               | —    | —        | 256        |
| 28F1.8   | 64    | [64, 139]                                 | $\Pi_{(0,20)}2_4^{-2}4_7^18_3^13^1$     | $\Pi_{(3,1)}2_4^{-2}4_1^18_5^{-1}$    | —    | —        | 768        |
| 28F1.9   | 64    | [64, 266]                                 | $\Pi_{(0,19)}4_7^53^1$                  | $\Pi_{(3,2)}4_1^5$                    | —    | —        | —          |
| 28F1.10  | 64    | [64, 139]                                 | $\Pi_{(0,19)}2_6^24^28_5^{-1}3^1$       | $\Pi_{(3,2)}2_6^{-2}4^{-2}8_7^1$      | —    | —        | 128        |
| 28F1.11  | 64    | [64, 134]                                 | $\Pi_{(0,19)}4_1^18_2^{-2}3^1$          | $\Pi_{(3,2)}4_3^{-1}8_6^2$            | —    | —        | 128        |
| 28F1.12  | 64    | $C_2 \times 2_+^{1+4} \mid [64, 264]$     | $\Pi_{(0,19)}2_4^{-2}4_7^33^1$          | $\Pi_{(3,2)}2_0^24_1^3$               | —    | —        | 128        |
| 28F1.13  | 64    | $C_2 \times 2_+^{1+4} \mid [64, 264]$     | $\Pi_{(0,19)}4_7^{-3}3^1$               | $\Pi_{(3,2)}4_1^{-3}$                 | —    | —        | 384        |
| 28F1.14  | 64    | $\Gamma_{25}a_1 \mid [64, 138]$           | $\Pi_{(0,18)}4_7^38_5^{-1}3^1$          | $\Pi_{(3,3)}4_1^{-3}8_7^1$            | —    | —        | —          |
| 29C1     | 24    | $S_4 \mid [24, 12]$                       | $\Pi_{(0,17)}4_3^33^2$                  | $\Pi_{(3,4)}4_5^33^{-1}$              | —    | $\times$ | 48         |
| 29C1.1   | 48    | $C_2 \times S_4 \mid [48, 48]$            | $\Pi_{(0,21)}2_6^28_3^{-1}3^1$          | $\Pi_{(3,0)}2_6^{-2}8_5^{-1}$         | —    | —        | 23040      |
| 29C1.2   | 48    | $C_2 \times S_4 \mid [48, 48]$            | $\Pi_{(0,20)}2_2^24_5^{-1}8_7^13^1$     | $\Pi_{(3,1)}2_4^{-2}4_1^18_5^{-1}$    | —    | —        | 96         |
| 29C1.3   | 48    | $C_2 \times S_4 \mid [48, 48]$            | $\Pi_{(0,18)}2^{-2}4_6^{-2}3^2$         | $\Pi_{(3,3)}2^24_6^23^{-1}$           | —    | —        | 96         |
| 29C1.4   | 48    | $C_2 \times S_4 \mid [48, 48]$            | $\Pi_{(0,17)}4_3^33^2$                  | $\Pi_{(3,4)}4_5^33^{-1}$              | —    | $\times$ | —          |
| 29F1     | 24    | $S_4 \mid [24, 12]$                       | $\Pi_{(0,17)}4_3^33^2$                  | $\Pi_{(3,4)}4_5^33^3$                 | (34) | $\times$ | —          |
| 29F1.1   | 48    | $C_2 \times S_4 \mid [48, 48]$            | $\Pi_{(0,21)}2_6^{-2}4_5^{-1}3^2$       | $\Pi_{(3,0)}2_4^{-2}4_1^13^{-1}$      | —    | —        | 1440       |
| 29F1.2   | 48    | $C_2 \times S_4 \mid [48, 48]$            | $\Pi_{(0,21)}2_2^28_1^13^{-2}$          | $\Pi_{(3,0)}2_6^28_3^{-1}3^1$         | —    | —        | 288        |
| 29F1.3   | 48    | $C_2 \times S_4 \mid [48, 48]$            | $\Pi_{(0,21)}2_6^28_3^{-1}3^1$          | $\Pi_{(3,0)}2_6^{-2}8_5^{-1}$         | —    | —        | 23040      |
| 29F1.4   | 48    | $C_2 \times S_4 \mid [48, 48]$            | $\Pi_{(0,20)}2_2^{-2}4_1^18_1^13^2$     | $\Pi_{(3,1)}2_6^24_1^18_5^{-1}3^{-1}$ | —    | —        | —          |
| 29F1.5   | 48    | $C_2 \times S_4 \mid [48, 48]$            | $\Pi_{(0,20)}2_2^{-2}4_6^{-2}3^{-2}$    | $\Pi_{(3,1)}2_0^24_4^{-2}3^1$         | —    | —        | 384        |
| 29F1.6   | 48    | $C_2 \times S_4 \mid [48, 48]$            | $\Pi_{(0,20)}2_2^24_2^23^{-2}$          | $\Pi_{(3,1)}2_0^24_4^{-2}3^1$         | —    | —        | 384        |
| 29F1.7   | 48    | $C_2 \times S_4 \mid [48, 48]$            | $\Pi_{(0,19)}2^{-2}8_7^13^3$            | $\Pi_{(3,2)}2^{-2}8_1^13^2$           | —    | —        | 96         |
| 29F1.8   | 48    | $C_2 \times S_4 \mid [48, 48]$            | $\Pi_{(0,19)}4_5^33^{-2}$               | $\Pi_{(3,2)}4_3^33^1$                 | —    | —        | 192        |
| 29F1.9   | 48    | $C_2 \times S_4 \mid [48, 48]$            | $\Pi_{(0,19)}2_4^{-4}4_5^{-1}3^{-2}$    | $\Pi_{(3,2)}2_0^44_3^{-1}3^1$         | —    | —        | 192        |
| 29F1.10  | 48    | $C_2 \times S_4 \mid [48, 48]$            | $\Pi_{(0,18)}4_5^{-1}8_7^13^3$          | $\Pi_{(3,3)}4_5^{-1}8_1^13^2$         | —    | $\times$ | —          |
| 30F1     | 8     | $D_8 \mid [8, 3]$                         | $\Pi_{(0,17)}2_6^44^{-2}8_1^1$          | $\Pi_{(3,4)}2_2^44^{-2}8_7^13^1$      | —    | —        | —          |
| 30F1.1   | 16    | $C_2 \times D_8 \mid [16, 11]$            | $\Pi_{(0,21)}2_6^28_3^{-1}3^1$          | $\Pi_{(3,0)}2_6^{-2}8_5^{-1}$         | —    | —        | 23040      |
| 30F1.2   | 16    | $C_2 \times D_8 \mid [16, 11]$            | $\Pi_{(0,21)}2_2^{-2}8_7^13^1$          | $\Pi_{(3,0)}2_6^{-2}8_5^{-1}$         | —    | —        | 23040      |

Table 2: Birational symplectic effective  $\chi$ -saturated groups

| $(X, G)$ | $\#G$ | Description of $G$          | $g(\Lambda_G)$                                 | $g(\Lambda^G)$                         | K3   | Cubic    | Saturation |
|----------|-------|-----------------------------|------------------------------------------------|----------------------------------------|------|----------|------------|
| 30F1.3   | 16    | $C_2 \times D_8$   [16, 11] | $\Pi_{(0,20)} 4_7^3 8_7^1 3^1$                 | $\Pi_{(3,1)} 4_1^3 8_1^1$              | —    | —        | 32         |
| 30F1.4   | 16    | $C_2 \times D_8$   [16, 11] | $\Pi_{(0,20)} 2_6^2 8_0^2 3^1$                 | $\Pi_{(3,1)} 2_2^2 8_0^2$              | —    | —        | 64         |
| 30F1.5   | 16    | $C_4 \circ D_8$   [16, 13]  | $\Pi_{(0,20)} 2^{-2} 8_6^{-2} 3^1$             | $\Pi_{(3,1)} 2^{-2} 8_2^{-2}$          | —    | —        | 64         |
| 30F1.6   | 16    | $C_2 \times D_8$   [16, 11] | $\Pi_{(0,20)} 2_4^{-2} 4_5^{-1} 8_1^1 3^1$     | $\Pi_{(3,1)} 2_4^{-2} 4_1^1 8_5^{-1}$  | —    | —        | 96         |
| 30F1.7   | 16    | $C_2 \times D_8$   [16, 11] | $\Pi_{(0,20)} 2_6^2 4^2 3^1$                   | $\Pi_{(3,1)} 2_6^{-2} 4^{-2}$          | —    | —        | 768        |
| 30F1.8   | 16    | $C_2 \times D_8$   [16, 11] | $\Pi_{(0,20)} 2_2^{-2} 4^2 3^1$                | $\Pi_{(3,1)} 2_6^{-2} 4^{-2}$          | —    | —        | 768        |
| 30F1.9   | 16    | $C_4 \circ D_8$   [16, 13]  | $\Pi_{(0,20)} 2_7^1 4_7^1 8^2 3^1$             | $\Pi_{(3,1)} 2_1^1 4_1^1 8^2$          | —    | —        | 32         |
| 30F1.10  | 16    | $C_2 \times D_8$   [16, 11] | $\Pi_{(0,20)} 4_7^3 8_7^1 3^1$                 | $\Pi_{(3,1)} 4_1^3 8_1^1$              | —    | —        | 32         |
| 30F1.11  | 16    | $C_2 \times D_8$   [16, 11] | $\Pi_{(0,19)} 2_6^2 4_1^1 8_4^{-2} 3^1$        | $\Pi_{(3,2)} 2_6^2 4_1^1 8_2^2$        | —    | —        | —          |
| 30F1.12  | 16    | $C_2 \times D_8$   [16, 11] | $\Pi_{(0,19)} 2_2^{-2} 4^2 8_5^{-1} 3^1$       | $\Pi_{(3,2)} 2_6^{-2} 4^{-2} 8_7^1$    | —    | —        | 64         |
| 30F1.13  | 16    | $C_2 \times D_8$   [16, 11] | $\Pi_{(0,19)} 2_2^{-2} 4^2 8_1^1 3^1$          | $\Pi_{(3,2)} 2_6^{-2} 4^{-2} 8_7^1$    | —    | —        | 64         |
| 30F1.14  | 16    | $C_2 \times D_8$   [16, 11] | $\Pi_{(0,19)} 2_6^4 8_5^{-1} 3^1$              | $\Pi_{(3,2)} 2_6^{-4} 8_3^{-1}$        | —    | —        | 48         |
| 30F1.15  | 16    | $C_2 \times D_8$   [16, 11] | $\Pi_{(0,18)} 2_4^{-2} 4_0^{-4} 3^1$           | $\Pi_{(3,3)} 2_0^2 4_0^4$              | —    | —        | —          |
| 30F1.16  | 16    | $C_2 \times D_8$   [16, 11] | $\Pi_{(0,18)} 2^2 4_0^4 3^1$                   | $\Pi_{(3,3)} 2^2 4_0^4$                | —    | —        | —          |
| 30F1.17  | 16    | $C_2 \times D_8$   [16, 11] | $\Pi_{(0,18)} 2_2^{-2} 4^2 8_2^2 3^1$          | $\Pi_{(3,3)} 2_2^2 8_6^2$              | —    | —        | —          |
| 31F1     | 8     | $Q_8$   [8, 4]              | $\Pi_{(0,17)} 2_7^{-3} 8^{-2}$                 | $\Pi_{(3,4)} 2_5^3 8^{-2} 3^1$         | (12) | $\times$ | —          |
| 31F1.1   | 16    | $Q_{16}$   [16, 9]          | $\Pi_{(0,21)} 4_3^{-1} 8_6^{-2} 3^1$           | $\Pi_{(3,0)} 4_3^{-1} 8_4^{-2}$        | —    | —        | 128        |
| 31F1.2   | 16    | $QD_{16}$   [16, 8]         | $\Pi_{(0,21)} 2_3^{-1} 4_3^{-1} 16_3^{-1} 3^1$ | $\Pi_{(3,0)} 2_1^1 4_1^1 16_1^1$       | —    | —        | 768        |
| 31F1.3   | 16    | $QD_{16}$   [16, 8]         | $\Pi_{(0,21)} 2_1^1 4_1^1 16_3^{-1} 3^1$       | $\Pi_{(3,0)} 2_1^1 4_1^1 16_1^1$       | —    | —        | 64         |
| 31F1.4   | 16    | $C_4 \circ D_8$   [16, 13]  | $\Pi_{(0,21)} 2_6^2 8_3^{-1} 3^1$              | $\Pi_{(3,0)} 2_6^{-2} 8_5^{-1}$        | —    | —        | 23040      |
| 31F1.5   | 16    | $QD_{16}$   [16, 8]         | $\Pi_{(0,20)} 2_0^2 4_5^{-1} 8_5^{-1} 3^1$     | $\Pi_{(3,1)} 2_4^{-2} 4_1^1 8_5^{-1}$  | —    | —        | 768        |
| 31F1.6   | 16    | $C_2 \times Q_8$   [16, 12] | $\Pi_{(0,20)} 2^{-2} 8_6^{-2} 3^1$             | $\Pi_{(3,1)} 2^{-2} 8_2^{-2}$          | —    | —        | 64         |
| 31F1.7   | 16    | $C_2 \times Q_8$   [16, 12] | $\Pi_{(0,20)} 2_3^3 16_3^{-1} 3^1$             | $\Pi_{(3,1)} 2_1^{-3} 16_5^{-1}$       | —    | —        | 384        |
| 31F1.8   | 16    | $C_2 \times Q_8$   [16, 12] | $\Pi_{(0,20)} 2_3^3 16_3^{-1} 3^1$             | $\Pi_{(3,1)} 2_1^{-3} 16_5^{-1}$       | —    | —        | 32         |
| 31F1.9   | 16    | $Q_{16}$   [16, 9]          | $\Pi_{(0,20)} 4_5^{-1} 8_1^1 3^1$              | $\Pi_{(3,1)} 4_1^1 8_5^{-1}$           | —    | —        | 11520      |
| 31F1.10  | 16    | $Q_{16}$   [16, 9]          | $\Pi_{(0,20)} 2_3^{-1} 4_3^{-1} 8^{-2} 3^1$    | $\Pi_{(3,1)} 2_1^1 4_1^1 8^2$          | —    | —        | 32         |
| 31F1.11  | 16    | $C_4 \circ D_8$   [16, 13]  | $\Pi_{(0,20)} 2_2^{-2} 8_4^{-2} 3^1$           | $\Pi_{(3,1)} 2_2^2 8_0^2$              | —    | —        | 64         |
| 31F1.12  | 16    | $QD_{16}$   [16, 8]         | $\Pi_{(0,20)} 2_2^{-2} 4_3^{-1} 16_5^{-1} 3^1$ | $\Pi_{(3,1)} 2_4^{-2} 4_3^{-1} 16_7^1$ | —    | —        | 32         |
| 31F1.13  | 16    | $C_2 \times Q_8$   [16, 12] | $\Pi_{(0,19)} 2_7^{-3} 8^{-2} 3^1$             | $\Pi_{(3,2)} 2_1^{-3} 8^{-2}$          | —    | —        | —          |
| 31F1.14  | 16    | $QD_{16}$   [16, 8]         | $\Pi_{(0,19)} 4_1^1 8_2^{-2} 3^1$              | $\Pi_{(3,2)} 4_3^{-1} 8_6^2$           | —    | —        | 32         |
| 31F1.15  | 16    | $Q_{16}$   [16, 9]          | $\Pi_{(0,19)} 4_7^1 8_0^2 3^1$                 | $\Pi_{(3,2)} 4_7^1 8_2^2$              | —    | $\times$ | 32         |
| 31F1.16  | 16    | $C_4 \circ D_8$   [16, 13]  | $\Pi_{(0,19)} 2_4^1 16_5^{-1} 3^1$             | $\Pi_{(3,2)} 2_2^{-4} 16_3^{-1}$       | —    | —        | —          |
| 31F1.17  | 16    | $C_4 \circ D_8$   [16, 13]  | $\Pi_{(0,19)} 4_6^{-2} 8_1^1 3^1$              | $\Pi_{(3,2)} 4_0^2 8_5^{-1}$           | —    | —        | 384        |
| 31F1.18  | 16    | $C_4 \circ D_8$   [16, 13]  | $\Pi_{(0,18)} 2_6^{-2} 8_6^2 3^1$              | $\Pi_{(3,3)} 2_2^{-2} 8_6^{-2}$        | —    | $\times$ | —          |
| 35C1     | 486   | [486, 249]                  | $\Pi_{(0,18)} 3^5$                             | $\Pi_{(3,3)} 3^4$                      | —    | $\times$ | 972        |
| 35C1.1   | 972   | [972, 811]                  | $\Pi_{(0,21)} 2_5^3 3^{-3}$                    | $\Pi_{(3,0)} 2_3^3 3^{-2}$             | —    | —        | 3888       |
| 35C1.2   | 972   | [972, 776]                  | $\Pi_{(0,21)} 2_7^{-3} 3^{-2}$                 | $\Pi_{(3,0)} 2_1^{-3} 3^1$             | —    | —        | 7776       |
| 35C1.3   | 972   | [972, 777]                  | $\Pi_{(0,20)} 2^{-2} 3^4$                      | $\Pi_{(3,1)} 2^{-2} 3^{-3}$            | —    | —        | 1944       |

Table 2: Birational symplectic effective  $\chi$ -saturated groups

| $(X, G)$ | $\#G$ | Description of $G$                              | $g(\Lambda_G)$                             | $g(\Lambda^G)$                      | K3   | Cubic | Saturation |
|----------|-------|-------------------------------------------------|--------------------------------------------|-------------------------------------|------|-------|------------|
| 35C1.4   | 972   | [972, 777]                                      | $\Pi_{(0,20)}2_2^23^3$                     | $\Pi_{(3,1)}2_6^23^2$               | —    | ×     | 3888       |
| 35C1.5   | 972   | [972, 811]                                      | $\Pi_{(0,19)}2_5^{-1}3^{-4}$               | $\Pi_{(3,2)}2_3^{-1}3^3$            | —    | ×     | 1944       |
| 35C1.6   | 972   | [972, 812]                                      | $\Pi_{(0,18)}3^5$                          | $\Pi_{(3,3)}3^4$                    | —    | ×     | —          |
| 35F1     | 486   | [486, 249]                                      | $\Pi_{(0,18)}3^5$                          | $\Pi_{(3,3)}3^{-6}$                 | —    | —     | —          |
| 37F1     | 192   | $C_4^2 \rtimes A_4 \mid [192, 1023]$            | $\Pi_{(0,18)}2^{-2}8_6^{-2}$               | $\Pi_{(3,3)}2^{-2}8_2^{-2}3^1$      | (75) | —     | —          |
| 37F1.1   | 384   | [384, 591]                                      | $\Pi_{(0,21)}2_3^{-1}4_3^{-1}16_3^{-1}3^1$ | $\Pi_{(3,0)}2_1^14_1^116_1^1$       | —    | —     | 768        |
| 37F1.2   | 384   | [384, 18235]                                    | $\Pi_{(0,21)}2_2^{-2}8_7^13^1$             | $\Pi_{(3,0)}2_6^{-2}8_5^{-1}$       | —    | —     | 23040      |
| 37F1.3   | 384   | $F_{384} \mid [384, 18135]$                     | $\Pi_{(0,20)}2_4^{-2}4_7^18_7^13^1$        | $\Pi_{(3,1)}2_4^{-2}4_1^18_5^{-1}$  | —    | —     | 768        |
| 37F1.4   | 384   | [384, 18134]                                    | $\Pi_{(0,20)}2_3^316_3^{-1}3^1$            | $\Pi_{(3,1)}2_1^{-3}16_5^{-1}$      | —    | —     | —          |
| 37F1.5   | 384   | $F_{384} \mid [384, 18135]$                     | $\Pi_{(0,20)}4_7^18_3^{-1}3^1$             | $\Pi_{(3,1)}4_1^18_5^{-1}$          | —    | —     | 11520      |
| 37F1.6   | 384   | [384, 18235]                                    | $\Pi_{(0,19)}4_0^28_3^{-1}3^1$             | $\Pi_{(3,2)}4_0^28_5^{-1}$          | —    | —     | —          |
| 38F1     | 96    | $C_2^2 \rtimes S_4 \mid [96, 227]$              | $\Pi_{(0,18)}2^24_3^{-1}8_1^13^{-1}$       | $\Pi_{(3,3)}2^24_5^{-1}8_7^13^2$    | (65) | —     | —          |
| 38F1.1   | 192   | $C_2 \times C_2^2 \rtimes S_4 \mid [192, 1538]$ | $\Pi_{(0,21)}2_2^{-2}8_3^13^1$             | $\Pi_{(3,0)}2_6^{-2}8_5^{-1}$       | —    | —     | 23040      |
| 38F1.2   | 192   | $C_2 \times C_2^2 \rtimes S_4 \mid [192, 1538]$ | $\Pi_{(0,21)}2_2^{-2}8_7^13^1$             | $\Pi_{(3,0)}2_6^{-2}8_5^{-1}$       | —    | —     | 23040      |
| 38F1.3   | 192   | $H_{192} \mid [192, 955]$                       | $\Pi_{(0,20)}2_4^{-2}4_4^{-2}3^{-2}$       | $\Pi_{(3,1)}2_0^24_4^{-2}3^1$       | —    | —     | 384        |
| 38F1.4   | 192   | $H_{192} \mid [192, 955]$                       | $\Pi_{(0,20)}2_4^{-2}4_4^{-2}3^{-2}$       | $\Pi_{(3,1)}2_0^24_4^{-2}3^1$       | —    | —     | 384        |
| 38F1.5   | 192   | $H_{192} \mid [192, 955]$                       | $\Pi_{(0,20)}2_2^{-2}4_1^18_3^13^1$        | $\Pi_{(3,1)}2_4^{-2}4_1^18_5^{-1}$  | —    | —     | 768        |
| 38F1.6   | 192   | $H_{192} \mid [192, 955]$                       | $\Pi_{(0,20)}4_7^18_3^{-1}3^1$             | $\Pi_{(3,1)}4_1^18_5^{-1}$          | —    | —     | 11520      |
| 38F1.7   | 192   | $C_2 \times C_2^2 \rtimes S_4 \mid [192, 1538]$ | $\Pi_{(0,19)}4_5^33^{-2}$                  | $\Pi_{(3,2)}4_3^33^1$               | —    | —     | —          |
| 38F1.8   | 192   | $C_2 \times C_2^2 \rtimes S_4 \mid [192, 1538]$ | $\Pi_{(0,19)}2_4^{-4}4_5^{-1}3^{-2}$       | $\Pi_{(3,2)}2_0^44_3^{-1}3^1$       | —    | —     | —          |
| 39C1     | 72    | $A_{4,3} \mid [72, 43]$                         | $\Pi_{(0,18)}4^{-2}3^{-3}$                 | $\Pi_{(3,3)}4^{-2}3^{-2}$           | —    | ×     | 144        |
| 39C1.1   | 144   | $C_2 \times A_{4,3} \mid [144, 189]$            | $\Pi_{(0,21)}2_2^28_1^13^{-2}$             | $\Pi_{(3,0)}2_6^28_3^{-1}3^1$       | —    | —     | 288        |
| 39C1.2   | 144   | $C_2 \times A_{4,3} \mid [144, 189]$            | $\Pi_{(0,21)}2_6^28_3^{-1}3^1$             | $\Pi_{(3,0)}2_6^{-2}8_5^{-1}$       | —    | —     | 23040      |
| 39C1.3   | 144   | $S_3 \times S_4 \mid [144, 183]$                | $\Pi_{(0,18)}4^{-2}3^{-3}$                 | $\Pi_{(3,3)}4^{-2}3^{-2}$           | —    | ×     | —          |
| 39F1     | 72    | $A_{4,3} \mid [72, 43]$                         | $\Pi_{(0,18)}4^{-2}3^{-3}$                 | $\Pi_{(3,3)}4^{-2}3^4$              | (61) | ×     | —          |
| 39F1.1   | 144   | $S_3 \times S_4 \mid [144, 183]$                | $\Pi_{(0,21)}2_2^{-2}8_3^{-1}3^{-3}$       | $\Pi_{(3,0)}2_6^{-2}8_5^{-1}3^{-2}$ | —    | —     | —          |
| 39F1.2   | 144   | $C_2 \times A_{4,3} \mid [144, 189]$            | $\Pi_{(0,19)}8_1^13^{-4}$                  | $\Pi_{(3,2)}8_7^13^3$               | —    | ×     | —          |
| 41F1     | 64    | [64, 266]                                       | $\Pi_{(0,18)}2_2^{-2}4^4$                  | $\Pi_{(3,3)}2_6^{-2}4^43^1$         | —    | —     | —          |
| 41F1.1   | 128   | [128, 1757]                                     | $\Pi_{(0,21)}2_2^{-2}8_7^13^1$             | $\Pi_{(3,0)}2_6^{-2}8_5^{-1}$       | —    | —     | 23040      |
| 41F1.2   | 128   | [128, 1753]                                     | $\Pi_{(0,20)}2_2^{-2}8_0^23^1$             | $\Pi_{(3,1)}2_2^28_0^2$             | —    | —     | 256        |
| 41F1.3   | 128   | $2_+^{1+6} \mid [128, 2326]$                    | $\Pi_{(0,20)}2_2^{-2}4^23^1$               | $\Pi_{(3,1)}2_6^{-2}4^{-2}$         | —    | —     | 768        |
| 41F1.4   | 128   | [128, 1757]                                     | $\Pi_{(0,19)}2_6^24^28_1^13^1$             | $\Pi_{(3,2)}2_6^{-2}4^{-2}8_7^1$    | —    | —     | —          |
| 43F1     | 64    | $\Gamma_{25}a_1 \mid [64, 138]$                 | $\Pi_{(0,18)}4_7^38_7^1$                   | $\Pi_{(3,3)}4_1^38_1^13^1$          | (56) | —     | —          |
| 43F1.1   | 128   | $C_2 \wr D_8 \mid [128, 928]$                   | $\Pi_{(0,21)}2_6^28_3^{-1}3^1$             | $\Pi_{(3,0)}2_6^{-2}8_5^{-1}$       | —    | —     | 23040      |
| 43F1.2   | 128   | $C_2 \wr D_8 \mid [128, 928]$                   | $\Pi_{(0,21)}2_2^{-2}8_3^{-1}3^1$          | $\Pi_{(3,0)}2_6^{-2}8_5^{-1}$       | —    | —     | 23040      |
| 43F1.3   | 128   | $C_2 \times \Gamma_{25}a_1 \mid [128, 1755]$    | $\Pi_{(0,21)}2_2^{-2}8_7^13^1$             | $\Pi_{(3,0)}2_6^{-2}8_5^{-1}$       | —    | —     | 23040      |
| 43F1.4   | 128   | $C_2 \times \Gamma_{25}a_1 \mid [128, 1755]$    | $\Pi_{(0,21)}2_2^{-2}8_3^{-1}3^1$          | $\Pi_{(3,0)}2_6^{-2}8_5^{-1}$       | —    | —     | 23040      |
| 43F1.5   | 128   | [128, 1758]                                     | $\Pi_{(0,20)}4_7^18_3^{-1}3^1$             | $\Pi_{(3,1)}4_1^18_5^{-1}$          | —    | —     | 11520      |

Table 2: Birational symplectic effective  $\chi$ -saturated groups

| $(X, G)$ | $\#G$ | Description of $G$                           | $g(\Lambda_G)$                            | $g(\Lambda^G)$                     | K3   | Cubic | Saturation |
|----------|-------|----------------------------------------------|-------------------------------------------|------------------------------------|------|-------|------------|
| 43F1.6   | 128   | [128, 932]                                   | $\Pi_{(0,20)}2_2^{-2}8_0^23^1$            | $\Pi_{(3,1)}2_2^28_0^2$            | —    | —     | 256        |
| 43F1.7   | 128   | [128, 932]                                   | $\Pi_{(0,20)}2_0^24_5^{-1}8_5^{-1}3^1$    | $\Pi_{(3,1)}2_4^{-2}4_1^18_5^{-1}$ | —    | —     | 768        |
| 43F1.8   | 128   | [128, 1758]                                  | $\Pi_{(0,20)}2_6^{-2}4_5^{-1}8_3^{-1}3^1$ | $\Pi_{(3,1)}2_4^{-2}4_1^18_5^{-1}$ | —    | —     | 768        |
| 43F1.9   | 128   | [128, 1758]                                  | $\Pi_{(0,20)}2_2^{-2}4^23^1$              | $\Pi_{(3,1)}2_6^{-2}4^{-2}$        | —    | —     | 768        |
| 43F1.10  | 128   | [128, 1758]                                  | $\Pi_{(0,20)}2_2^{-2}4^23^1$              | $\Pi_{(3,1)}2_6^{-2}4^{-2}$        | —    | —     | 768        |
| 43F1.11  | 128   | [128, 932]                                   | $\Pi_{(0,20)}4_7^18_3^{-1}3^1$            | $\Pi_{(3,1)}4_1^18_5^{-1}$         | —    | —     | 11520      |
| 43F1.12  | 128   | $C_2 \wr D_8 \mid [128, 928]$                | $\Pi_{(0,19)}4_7^18_4^{-1}3^1$            | $\Pi_{(3,2)}4_3^{-1}8_6^2$         | —    | —     | —          |
| 43F1.13  | 128   | $C_2 \times \Gamma_{25}a_1 \mid [128, 1755]$ | $\Pi_{(0,19)}2_4^{-2}4_7^23^1$            | $\Pi_{(3,2)}2_0^24_1^3$            | —    | —     | —          |
| 43F1.14  | 128   | $C_2 \times \Gamma_{25}a_1 \mid [128, 1755]$ | $\Pi_{(0,19)}4_7^{-3}3^1$                 | $\Pi_{(3,2)}4_1^{-3}$              | —    | —     | 384        |
| 44C1     | 60    | $A_5 \mid [60, 5]$                           | $\Pi_{(0,18)}2^{-2}3^15^{-2}$             | $\Pi_{(3,3)}2^{-2}5^{-2}$          | —    | ×     | 120        |
| 44C1.1   | 120   | $S_5 \mid [120, 34]$                         | $\Pi_{(0,21)}2_6^{-2}4_3^{-1}3^15^{-1}$   | $\Pi_{(3,0)}2_0^24_3^{-1}5^{-1}$   | —    | —     | 480        |
| 44C1.2   | 120   | $C_2 \times A_5 \mid [120, 35]$              | $\Pi_{(0,20)}2_6^43^15^{-1}$              | $\Pi_{(3,1)}2_6^{-4}5^{-1}$        | —    | —     | 240        |
| 44C1.3   | 120   | $C_2 \times A_5 \mid [120, 35]$              | $\Pi_{(0,19)}4_3^{-1}3^15^{-2}$           | $\Pi_{(3,2)}4_5^{-1}5^{-2}$        | —    | ×     | 240        |
| 44C1.4   | 120   | $S_5 \mid [120, 34]$                         | $\Pi_{(0,18)}2^{-2}3^15^{-2}$             | $\Pi_{(3,3)}2^{-2}5^{-2}$          | —    | ×     | —          |
| 44F1     | 60    | $A_5 \mid [60, 5]$                           | $\Pi_{(0,18)}2^{-2}3^15^{-2}$             | $\Pi_{(3,3)}2^{-2}3^{-2}5^{-2}$    | (55) | ×     | —          |
| 44F1.1   | 120   | $C_2 \times A_5 \mid [120, 35]$              | $\Pi_{(0,21)}2_6^{-2}4_5^{-1}3^2$         | $\Pi_{(3,0)}2_4^{-2}4_1^13^{-1}$   | —    | —     | 1440       |
| 44F1.2   | 120   | $C_2 \times A_5 \mid [120, 35]$              | $\Pi_{(0,21)}2_4^{-2}4_1^13^15^1$         | $\Pi_{(3,0)}2_4^{-2}4_1^15^1$      | —    | —     | 240        |
| 44F1.3   | 120   | $C_2 \times A_5 \mid [120, 35]$              | $\Pi_{(0,21)}2_4^{-2}4_1^13^15^1$         | $\Pi_{(3,0)}2_4^{-2}4_1^15^1$      | —    | —     | 240        |
| 44F1.4   | 120   | $S_5 \mid [120, 34]$                         | $\Pi_{(0,21)}2_4^{-2}4_5^{-1}3^15^{-1}$   | $\Pi_{(3,0)}2_0^24_3^{-1}5^{-1}$   | —    | —     | 3840       |
| 44F1.5   | 120   | $S_5 \mid [120, 34]$                         | $\Pi_{(0,20)}2_2^43^15^1$                 | $\Pi_{(3,1)}2_2^{-4}5^1$           | —    | —     | —          |
| 44F1.6   | 120   | $C_2 \times A_5 \mid [120, 35]$              | $\Pi_{(0,20)}2^{-2}3^25^1$                | $\Pi_{(3,1)}2^{-2}3^{-1}5^1$       | —    | —     | 1440       |
| 44F1.7   | 120   | $S_5 \mid [120, 34]$                         | $\Pi_{(0,19)}4_5^{-1}3^25^1$              | $\Pi_{(3,2)}4_3^{-1}3^{-1}5^1$     | —    | ×     | 720        |
| 45C1     | 48    | $C_2 \times S_4 \mid [48, 48]$               | $\Pi_{(0,18)}2^{-2}4_6^{-2}3^2$           | $\Pi_{(3,3)}2^{-2}4_2^{-2}3^{-1}$  | —    | —     | 96         |
| 45C1.1   | 96    | $C_2^2 \times S_4 \mid [96, 226]$            | $\Pi_{(0,21)}2_2^{-2}8_7^13^1$            | $\Pi_{(3,0)}2_6^{-2}8_5^{-1}$      | —    | —     | 23040      |
| 45C1.2   | 96    | $A_4 \rtimes D_8 \mid [96, 195]$             | $\Pi_{(0,20)}2_2^{-2}4^23^1$              | $\Pi_{(3,1)}2_6^{-2}4^{-2}$        | —    | —     | 768        |
| 45C1.3   | 96    | $C_4 \rtimes S_4 \mid [96, 187]$             | $\Pi_{(0,19)}2^28_1^13^2$                 | $\Pi_{(3,2)}2^28_7^13^{-1}$        | —    | —     | 576        |
| 45C1.4   | 96    | $C_2^2 \times S_4 \mid [96, 226]$            | $\Pi_{(0,18)}2^24_2^23^2$                 | $\Pi_{(3,3)}2^{-2}4_2^{-2}3^{-1}$  | —    | —     | —          |
| 45F1     | 48    | $C_2 \times S_4 \mid [48, 48]$               | $\Pi_{(0,18)}2^{-2}4_6^{-2}3^2$           | $\Pi_{(3,3)}2^{-2}4_2^{-2}3^3$     | (51) | —     | —          |
| 45F1.1   | 96    | $C_4 \rtimes S_4 \mid [96, 187]$             | $\Pi_{(0,21)}4_3^{-3}3^{-2}$              | $\Pi_{(3,0)}4_5^{-3}3^1$           | —    | —     | —          |
| 45F1.2   | 96    | $C_4 \rtimes S_4 \mid [96, 187]$             | $\Pi_{(0,21)}2_6^28_1^13^2$               | $\Pi_{(3,0)}2_2^28_3^{-1}3^{-1}$   | —    | —     | 768        |
| 45F1.3   | 96    | $C_2^2 \times S_4 \mid [96, 226]$            | $\Pi_{(0,20)}2_6^24_6^{-2}3^{-2}$         | $\Pi_{(3,1)}2_0^24_4^{-2}3^1$      | —    | —     | 384        |
| 45F1.4   | 96    | $A_4 \rtimes D_8 \mid [96, 195]$             | $\Pi_{(0,20)}4_2^{-2}3^3$                 | $\Pi_{(3,1)}4_6^{-2}3^2$           | —    | —     | 576        |
| 45F1.5   | 96    | $C_2^2 \times S_4 \mid [96, 226]$            | $\Pi_{(0,19)}2^{-2}8_7^13^3$              | $\Pi_{(3,2)}2^{-2}8_1^13^2$        | —    | —     | —          |
| 46C1     | 36    | $C_3^2 \rtimes C_4 \mid [36, 9]$             | $\Pi_{(0,18)}2_2^23^29^{-1}$              | $\Pi_{(3,3)}2_2^{-2}3^{-1}9^1$     | —    | ×     | 72         |
| 46C1.1   | 72    | $C_2 \times C_3^2 \rtimes C_4 \mid [72, 45]$ | $\Pi_{(0,21)}2_2^{-2}4_1^13^2$            | $\Pi_{(3,0)}2_4^{-2}4_1^13^{-1}$   | —    | —     | 1440       |
| 46C1.2   | 72    | $C_2 \times C_3^2 \rtimes C_4 \mid [72, 45]$ | $\Pi_{(0,20)}2_6^43^19^{-1}$              | $\Pi_{(3,1)}2_2^49^1$              | —    | —     | 144        |
| 46C1.3   | 72    | $C_2 \times C_3^2 \rtimes C_4 \mid [72, 45]$ | $\Pi_{(0,19)}4_1^13^29^{-1}$              | $\Pi_{(3,2)}4_7^13^{-1}9^1$        | —    | ×     | 144        |
| 46C1.4   | 72    | $N_{72} \mid [72, 40]$                       | $\Pi_{(0,18)}2_6^{-2}3^29^{-1}$           | $\Pi_{(3,3)}2_2^{-2}3^{-1}9^1$     | —    | ×     | —          |

Table 2: Birational symplectic effective  $\chi$ -saturated groups

| $(X, G)$ | $\#G$ | Description of $G$                           | $g(\Lambda_G)$                              | $g(\Lambda^G)$                       | K3   | Cubic    | Saturation |
|----------|-------|----------------------------------------------|---------------------------------------------|--------------------------------------|------|----------|------------|
| 46F1     | 36    | $C_3^2 \rtimes C_4 \mid [36, 9]$             | $\Pi_{(0,18)} 2_2^2 3^2 9^{-1}$             | $\Pi_{(3,3)} 2_2^{-2} 3^3 9^1$       | (46) | $\times$ | —          |
| 46F1.1   | 72    | $F_9 \mid [72, 39]$                          | $\Pi_{(0,21)} 2^{-2} 4_7^1 3^{-2} 9^{-1}$   | $\Pi_{(3,0)} 2^2 4_5^{-1} 3^1 9^1$   | —    | —        | —          |
| 46F1.2   | 72    | $F_9 \mid [72, 39]$                          | $\Pi_{(0,21)} 2^{-2} 4_7^1 3^{-2} 9^{-1}$   | $\Pi_{(3,0)} 2^{-2} 4_1^1 3^1 9^1$   | —    | —        | —          |
| 46F1.3   | 72    | $N_{72} \mid [72, 40]$                       | $\Pi_{(0,21)} 2_4^{-2} 4_1^1 3^3$           | $\Pi_{(3,0)} 2_6^2 4_1^1 3^2$        | —    | —        | 144        |
| 46F1.4   | 72    | $M_9 \mid [72, 41]$                          | $\Pi_{(0,21)} 2_7^{-3} 3^{-2}$              | $\Pi_{(3,0)} 2_1^{-3} 3^1$           | —    | —        | 7776       |
| 46F1.5   | 72    | $M_9 \mid [72, 41]$                          | $\Pi_{(0,21)} 2_7^{-3} 3^{-2}$              | $\Pi_{(3,0)} 2_1^{-3} 3^1$           | —    | —        | 40320      |
| 46F1.6   | 72    | $M_9 \mid [72, 41]$                          | $\Pi_{(0,21)} 2_7^{-3} 3^{-2}$              | $\Pi_{(3,0)} 2_1^{-3} 3^1$           | —    | —        | 7776       |
| 46F1.7   | 72    | $C_2 \times C_3^2 \rtimes C_4 \mid [72, 45]$ | $\Pi_{(0,20)} 2_2^4 3^3$                    | $\Pi_{(3,1)} 2_6^4 3^2$              | —    | —        | —          |
| 46F1.8   | 72    | $C_2 \times C_3^2 \rtimes C_4 \mid [72, 45]$ | $\Pi_{(0,20)} 2_6^{-2} 3^3$                 | $\Pi_{(3,1)} 2_6^2 3^2$              | —    | $\times$ | 3888       |
| 47C1     | 36    | $S_3^2 \mid [36, 10]$                        | $\Pi_{(0,18)} 2^{-2} 3^3 9^{-1}$            | $\Pi_{(3,3)} 2^{-2} 3^2 9^1$         | —    | $\times$ | 72         |
| 47C1.1   | 72    | $C_2 \times S_3^2 \mid [72, 46]$             | $\Pi_{(0,21)} 2_6^2 4_3^{-1} 3^3$           | $\Pi_{(3,0)} 2_6^2 4_1^1 3^2$        | —    | —        | 144        |
| 47C1.2   | 72    | $N_{72} \mid [72, 40]$                       | $\Pi_{(0,19)} 4_1^1 3^2 9^{-1}$             | $\Pi_{(3,2)} 4_7^1 3^{-1} 9^1$       | —    | $\times$ | 144        |
| 47C1.3   | 72    | $C_2 \times S_3^2 \mid [72, 46]$             | $\Pi_{(0,18)} 2^{-2} 3^3 9^{-1}$            | $\Pi_{(3,3)} 2^{-2} 3^2 9^1$         | —    | $\times$ | —          |
| 47C2     | 36    | $S_3^2 \mid [36, 10]$                        | $\Pi_{(0,18)} 2^{-2} 3^3 9^{-1}$            | $\Pi_{(3,3)} 2^{-2} 3^2 9^1$         | —    | $\times$ | 72         |
| 47C2.1   | 72    | $N_{72} \mid [72, 40]$                       | $\Pi_{(0,21)} 2_6^2 4_3^{-1} 3^3$           | $\Pi_{(3,0)} 2_6^2 4_1^1 3^2$        | —    | —        | 144        |
| 47C2.2   | 72    | $C_2 \times S_3^2 \mid [72, 46]$             | $\Pi_{(0,20)} 2_6^4 3^1 9^{-1}$             | $\Pi_{(3,1)} 2_2^4 9^1$              | —    | —        | 144        |
| 47C2.3   | 72    | $C_2 \times S_3^2 \mid [72, 46]$             | $\Pi_{(0,19)} 4_1^1 3^2 9^{-1}$             | $\Pi_{(3,2)} 4_7^1 3^{-1} 9^1$       | —    | $\times$ | 144        |
| 47C2.4   | 72    | $N_{72} \mid [72, 40]$                       | $\Pi_{(0,18)} 2^{-2} 3^3 9^{-1}$            | $\Pi_{(3,3)} 2^{-2} 3^2 9^1$         | —    | $\times$ | —          |
| 47F1     | 36    | $S_3^2 \mid [36, 10]$                        | $\Pi_{(0,18)} 2^{-2} 3^3 9^{-1}$            | $\Pi_{(3,3)} 2^{-2} 3^{-4} 9^1$      | (48) | —        | —          |
| 47F1.1   | 72    | $C_2 \times S_3^2 \mid [72, 46]$             | $\Pi_{(0,21)} 2_0^2 4_3^{-1} 3^{-2} 9^{-1}$ | $\Pi_{(3,0)} 2_0^2 4_5^{-1} 3^1 9^1$ | —    | —        | —          |
| 47F1.2   | 72    | $N_{72} \mid [72, 40]$                       | $\Pi_{(0,21)} 2_4^{-2} 4_1^1 3^3$           | $\Pi_{(3,0)} 2_6^2 4_1^1 3^2$        | —    | —        | 144        |
| 47F1.3   | 72    | $N_{72} \mid [72, 40]$                       | $\Pi_{(0,21)} 2_4^{-2} 4_1^1 3^3$           | $\Pi_{(3,0)} 2_6^2 4_1^1 3^2$        | —    | —        | 144        |
| 47F1.4   | 72    | $C_2 \times S_3^2 \mid [72, 46]$             | $\Pi_{(0,20)} 2_0^{-4} 3^4$                 | $\Pi_{(3,1)} 2_0^{-4} 3^{-3}$        | —    | —        | —          |
| 48F1     | 32    | $[32, 34]$                                   | $\Pi_{(0,18)} 2_2^{-2} 4^4$                 | $\Pi_{(3,3)} 2_6^{-2} 4^4 3^1$       | —    | —        | —          |
| 48F1.1   | 64    | $[64, 34]$                                   | $\Pi_{(0,21)} 4_5^{-1} 8_4^{-2} 3^1$        | $\Pi_{(3,0)} 4_3^{-1} 8_4^{-2}$      | —    | —        | —          |
| 48F1.2   | 64    | $[64, 241]$                                  | $\Pi_{(0,21)} 4_3^3 3^1$                    | $\Pi_{(3,0)} 4_3^3$                  | —    | —        | —          |
| 48F1.3   | 64    | $D_8^2 \mid [64, 226]$                       | $\Pi_{(0,21)} 2_2^{-2} 8_7^1 3^1$           | $\Pi_{(3,0)} 2_6^{-2} 8_5^{-1}$      | —    | —        | 23040      |
| 48F1.4   | 64    | $[64, 241]$                                  | $\Pi_{(0,20)} 2_6^2 8_4^{-2} 3^1$           | $\Pi_{(3,1)} 2_2^2 8_0^2$            | —    | —        | 256        |
| 48F1.5   | 64    | $D_8^2 \mid [64, 226]$                       | $\Pi_{(0,20)} 2_2^{-2} 4^2 3^1$             | $\Pi_{(3,1)} 2_6^{-2} 4^{-2}$        | —    | —        | 768        |
| 48F1.6   | 64    | $D_8^2 \mid [64, 226]$                       | $\Pi_{(0,19)} 2_2^{-2} 4^2 8_1^1 3^1$       | $\Pi_{(3,2)} 2_6^{-2} 4^{-2} 8_7^1$  | —    | —        | —          |
| 52F1     | 21    | $C_7 \rtimes C_3 \mid [21, 1]$               | $\Pi_{(0,18)} 7^3$                          | $\Pi_{(3,3)} 3^1 7^{-3}$             | (33) | $\times$ | —          |
| 52F1.1   | 42    | $F_7 \mid [42, 1]$                           | $\Pi_{(0,21)} 2_7^3 3^1 7^{-1}$             | $\Pi_{(3,0)} 2_1^3 7^1$              | —    | —        | 672        |
| 52F1.2   | 42    | $F_7 \mid [42, 1]$                           | $\Pi_{(0,21)} 2_7^3 3^1 7^{-1}$             | $\Pi_{(3,0)} 2_1^3 7^1$              | —    | —        | 672        |
| 52F1.3   | 42    | $F_7 \mid [42, 1]$                           | $\Pi_{(0,19)} 2_3^{-1} 3^1 7^{-2}$          | $\Pi_{(3,2)} 2_5^{-1} 7^{-2}$        | —    | $\times$ | —          |
| 53F1     | 20    | $F_5 \mid [20, 3]$                           | $\Pi_{(0,18)} 2_6^{-2} 5^3$                 | $\Pi_{(3,3)} 2_6^2 3^1 5^3$          | (32) | $\times$ | —          |
| 53F1.1   | 40    | $C_2 \times F_5 \mid [40, 12]$               | $\Pi_{(0,21)} 2_6^2 4_3^{-1} 3^1 5^1$       | $\Pi_{(3,0)} 2_4^{-2} 4_7^1 5^1$     | —    | —        | 240        |
| 53F1.2   | 40    | $C_2 \times F_5 \mid [40, 12]$               | $\Pi_{(0,21)} 2_6^2 4_3^{-1} 3^1 5^1$       | $\Pi_{(3,0)} 2_4^{-2} 4_7^1 5^1$     | —    | —        | 240        |
| 53F1.3   | 40    | $C_2 \times F_5 \mid [40, 12]$               | $\Pi_{(0,21)} 2_6^{-2} 4_3^{-1} 3^1 5^{-1}$ | $\Pi_{(3,0)} 2_0^2 4_3^{-1} 5^{-1}$  | —    | —        | 480        |

Table 2: Birational symplectic effective  $\chi$ -saturated groups

| $(X, G)$ | $\#G$ | Description of $G$                 | $g(\Lambda_G)$                                | $g(\Lambda^G)$                                  | K3       | Cubic    | Saturation |
|----------|-------|------------------------------------|-----------------------------------------------|-------------------------------------------------|----------|----------|------------|
| 53F1.4   | 40    | $C_2 \times F_5 \mid [40, 12]$     | $\Pi_{(0,20)} 2_6^{-4} 3^1 5^{-2}$            | $\Pi_{(3,1)} 2_6^4 5^{-2}$                      | —        | —        | —          |
| 53F1.5   | 40    | $C_2 \times F_5 \mid [40, 12]$     | $\Pi_{(0,20)} 2_6^4 3^1 5^{-1}$               | $\Pi_{(3,1)} 2_6^{-4} 5^{-1}$                   | —        | —        | 240        |
| 53F1.6   | 40    | $C_2 \times F_5 \mid [40, 12]$     | $\Pi_{(0,19)} 4_3^{-1} 3^1 5^{-2}$            | $\Pi_{(3,2)} 4_5^{-1} 5^{-2}$                   | —        | $\times$ | 240        |
| 55F1     | 16    | $QD_{16} \mid [16, 8]$             | $\Pi_{(0,18)} 2_1^1 4_5^{-1} 8^2$             | $\Pi_{(3,3)} 2_5^{-1} 4_5^{-1} 8^{-2} 3^1$ (26) | $\times$ | —        | —          |
| 55F1.1   | 32    | $C_4 \circ D_{16} \mid [32, 42]$   | $\Pi_{(0,21)} 4_5^{-1} 8_4^{-2} 3^1$          | $\Pi_{(3,0)} 4_3^{-1} 8_4^{-2}$                 | —        | —        | 128        |
| 55F1.2   | 32    | $\Gamma_6 a_2 \mid [32, 44]$       | $\Pi_{(0,21)} 4_5^{-1} 8_4^{-2} 3^1$          | $\Pi_{(3,0)} 4_3^{-1} 8_4^{-2}$                 | —        | —        | 128        |
| 55F1.3   | 32    | $C_2 \times QD_{16} \mid [32, 40]$ | $\Pi_{(0,21)} 2_1^1 4_1^1 16_3^{-1} 3^1$      | $\Pi_{(3,0)} 2_1^1 4_1^1 16_1^1$                | —        | —        | 768        |
| 55F1.4   | 32    | $C_2 \times QD_{16} \mid [32, 40]$ | $\Pi_{(0,21)} 2_1^1 4_5^{-1} 16_7^1 3^1$      | $\Pi_{(3,0)} 2_1^1 4_1^1 16_1^1$                | —        | —        | 64         |
| 55F1.5   | 32    | $\text{Aut}(D_{16}) \mid [32, 43]$ | $\Pi_{(0,21)} 2_6^2 8_3^{-1} 3^1$             | $\Pi_{(3,0)} 2_6^{-2} 8_5^{-1}$                 | —        | —        | 23040      |
| 55F1.6   | 32    | $C_4 \circ D_{16} \mid [32, 42]$   | $\Pi_{(0,21)} 2_2^{-2} 8_7^1 3^1$             | $\Pi_{(3,0)} 2_6^{-2} 8_5^{-1}$                 | —        | —        | 23040      |
| 55F1.7   | 32    | $\Gamma_6 a_2 \mid [32, 44]$       | $\Pi_{(0,20)} 2_5^{-1} 4_5^{-1} 8^2 3^1$      | $\Pi_{(3,1)} 2_1^1 4_1^1 8^2$                   | —        | —        | —          |
| 55F1.8   | 32    | $C_4 \circ D_{16} \mid [32, 42]$   | $\Pi_{(0,20)} 2_2^{-2} 8_4^{-2} 3^1$          | $\Pi_{(3,1)} 2_2^2 8_0^2$                       | —        | —        | 64         |
| 55F1.9   | 32    | $\text{Aut}(D_{16}) \mid [32, 43]$ | $\Pi_{(0,20)} 2_6^2 8_4^{-2} 3^1$             | $\Pi_{(3,1)} 2_2^2 8_0^2$                       | —        | —        | 64         |
| 55F1.10  | 32    | $\Gamma_6 a_2 \mid [32, 44]$       | $\Pi_{(0,20)} 2^{-2} 8_6^{-2} 3^1$            | $\Pi_{(3,1)} 2^{-2} 8_2^{-2}$                   | —        | —        | 64         |
| 55F1.11  | 32    | $\text{Aut}(D_{16}) \mid [32, 43]$ | $\Pi_{(0,20)} 2_0^2 4_5^{-1} 16_1^1 3^1$      | $\Pi_{(3,1)} 2_4^{-2} 4_3^{-1} 16_7^1$          | —        | —        | —          |
| 55F1.12  | 32    | $\text{Aut}(D_{16}) \mid [32, 43]$ | $\Pi_{(0,20)} 2_4^{-2} 4_5^{-1} 8_5^{-1} 3^1$ | $\Pi_{(3,1)} 2_4^{-2} 4_1^1 8_5^{-1}$           | —        | —        | 768        |
| 55F1.13  | 32    | $C_4 \circ D_{16} \mid [32, 42]$   | $\Pi_{(0,20)} 4_5^{-1} 8_1^1 3^1$             | $\Pi_{(3,1)} 4_1^1 8_5^{-1}$                    | —        | —        | 11520      |
| 55F1.14  | 32    | $\text{Aut}(D_{16}) \mid [32, 43]$ | $\Pi_{(0,19)} 4_7^1 8_4^{-2} 3^1$             | $\Pi_{(3,2)} 4_3^{-1} 8_6^2$                    | —        | —        | —          |
| 55F1.15  | 32    | $C_4 \circ D_{16} \mid [32, 42]$   | $\Pi_{(0,19)} 4_7^1 8_0^2 3^1$                | $\Pi_{(3,2)} 4_7^1 8_2^2$                       | —        | $\times$ | —          |
| 56F1     | 12    | $A_4 \mid [12, 3]$                 | $\Pi_{(0,18)} 2_6^2 4^4$                      | $\Pi_{(3,3)} 2_2^2 4^{-4} 3^1$                  | —        | —        | —          |
| 56F1.1   | 24    | $S_4 \mid [24, 12]$                | $\Pi_{(0,21)} 4_5^{-1} 8_4^{-2} 3^1$          | $\Pi_{(3,0)} 4_3^{-1} 8_4^{-2}$                 | —        | —        | —          |
| 56F1.2   | 24    | $S_4 \mid [24, 12]$                | $\Pi_{(0,21)} 4_3^3 3^1$                      | $\Pi_{(3,0)} 4_3^3$                             | —        | —        | —          |
| 56F1.3   | 24    | $S_4 \mid [24, 12]$                | $\Pi_{(0,20)} 4_5^{-3} 8_5^{-1} 3^1$          | $\Pi_{(3,1)} 4_1^3 8_1^1$                       | —        | —        | —          |
| 58F1     | 8     | $C_2^3 \mid [8, 5]$                | $\Pi_{(0,18)} 2_4^{-2} 4_5^{-3} 8_5^{-1}$     | $\Pi_{(3,3)} 2_4^{-2} 4_3^{-3} 8_3^{-1} 3^1$    | —        | —        | —          |
| 58F1.1   | 16    | $C_2 \times D_8 \mid [16, 11]$     | $\Pi_{(0,21)} 4_3^{-1} 8_6^{-2} 3^1$          | $\Pi_{(3,0)} 4_3^{-1} 8_4^{-2}$                 | —        | —        | 128        |
| 58F1.2   | 16    | $C_2 \times D_8 \mid [16, 11]$     | $\Pi_{(0,21)} 4_7^1 8_6^2 3^1$                | $\Pi_{(3,0)} 4_3^{-1} 8_4^{-2}$                 | —        | —        | 128        |
| 58F1.3   | 16    | $C_2 \times D_8 \mid [16, 11]$     | $\Pi_{(0,21)} 2_6^2 8_7^1 3^1$                | $\Pi_{(3,0)} 2_6^{-2} 8_5^{-1}$                 | —        | —        | 23040      |
| 58F1.4   | 16    | $C_2^4 \mid [16, 14]$              | $\Pi_{(0,21)} 2_2^{-2} 8_7^1 3^1$             | $\Pi_{(3,0)} 2_6^{-2} 8_5^{-1}$                 | —        | —        | 23040      |
| 58F1.5   | 16    | $C_2^4 \mid [16, 14]$              | $\Pi_{(0,20)} 2_2^{-2} 4^2 3^1$               | $\Pi_{(3,1)} 2_6^{-2} 4^{-2}$                   | —        | —        | 768        |
| 58F1.6   | 16    | $C_2 \times D_8 \mid [16, 11]$     | $\Pi_{(0,20)} 2_1^1 4_7^1 8^2 3^1$            | $\Pi_{(3,1)} 2_1^1 4_1^1 8^2$                   | —        | —        | 32         |
| 58F1.7   | 16    | $C_2 \times D_8 \mid [16, 11]$     | $\Pi_{(0,20)} 4_7^3 8_7^1 3^1$                | $\Pi_{(3,1)} 4_1^3 8_1^1$                       | —        | —        | 32         |
| 58F1.8   | 16    | $C_2^4 \mid [16, 14]$              | $\Pi_{(0,20)} 4_5^3 8_1^1 3^1$                | $\Pi_{(3,1)} 4_1^3 8_1^1$                       | —        | —        | 32         |
| 58F1.9   | 16    | $C_2 \times D_8 \mid [16, 11]$     | $\Pi_{(0,20)} 2_2^{-2} 8_0^2 3^1$             | $\Pi_{(3,1)} 2_2^2 8_0^2$                       | —        | —        | 256        |
| 58F1.10  | 16    | $C_2 \times D_8 \mid [16, 11]$     | $\Pi_{(0,20)} 2_2^{-2} 4_7^1 8_1^1 3^1$       | $\Pi_{(3,1)} 2_4^{-2} 4_1^1 8_5^{-1}$           | —        | —        | 96         |
| 58F1.11  | 16    | $C_2^4 \mid [16, 14]$              | $\Pi_{(0,20)} 2_2^{-2} 4_7^1 8_1^1 3^1$       | $\Pi_{(3,1)} 2_4^{-2} 4_1^1 8_5^{-1}$           | —        | —        | 96         |
| 58F1.12  | 16    | $C_2 \times D_8 \mid [16, 11]$     | $\Pi_{(0,19)} 2_6^2 4_1^1 8_0^2 3^1$          | $\Pi_{(3,2)} 2_6^2 4_1^1 8_2^2$                 | —        | —        | —          |
| 58F1.13  | 16    | $C_2^4 \mid [16, 14]$              | $\Pi_{(0,19)} 4_7^5 3^1$                      | $\Pi_{(3,2)} 4_1^5$                             | —        | —        | —          |
| 58F1.14  | 16    | $C_2^4 \mid [16, 14]$              | $\Pi_{(0,19)} 2_2^{-2} 4_1^3 3^1$             | $\Pi_{(3,2)} 2_0^2 4_1^3$                       | —        | —        | —          |



Table 2: Birational symplectic effective  $\chi$ -saturated groups

| $(X, G)$ | $\#G$ | Description of $G$               | $g(\Lambda_G)$                                | $g(\Lambda^G)$                        | K3 | Cubic | Saturation |
|----------|-------|----------------------------------|-----------------------------------------------|---------------------------------------|----|-------|------------|
| 59F1     | 8     | $C_2 \times C_4 \mid [8, 2]$     | $\Pi_{(0,18)} 2_0^{-4} 8_2^2$                 | $\Pi_{(3,3)} 2_0^{-4} 8_6^2 3^1$      | —  | —     | —          |
| 59F1.1   | 16    | $M_4(2) \mid [16, 6]$            | $\Pi_{(0,21)} 4_2^{-2} 16_3^{-1} 3^1$         | $\Pi_{(3,0)} 4_2^2 16_1^1$            | —  | —     | —          |
| 59F1.2   | 16    | $C_2 \times D_8 \mid [16, 11]$   | $\Pi_{(0,21)} 4_5^{-1} 8_4^{-2} 3^1$          | $\Pi_{(3,0)} 4_3^{-1} 8_4^{-2}$       | —  | —     | 128        |
| 59F1.3   | 16    | $M_4(2) \mid [16, 6]$            | $\Pi_{(0,21)} 2_7^1 4_3^{-1} 16_3^{-1} 3^1$   | $\Pi_{(3,0)} 2_1^1 4_1^1 16_1^1$      | —  | —     | 64         |
| 59F1.4   | 16    | $C_2^2 \times C_4 \mid [16, 3]$  | $\Pi_{(0,21)} 4_6^2 8_7^1 3^1$                | $\Pi_{(3,0)} 4_2^2 8_1^1$             | —  | —     | —          |
| 59F1.5   | 16    | $C_2 \times D_8 \mid [16, 11]$   | $\Pi_{(0,21)} 2_6^2 8_3^{-1} 3^1$             | $\Pi_{(3,0)} 2_6^{-2} 8_5^{-1}$       | —  | —     | 23040      |
| 59F1.6   | 16    | $C_4 \circ D_8 \mid [16, 13]$    | $\Pi_{(0,21)} 4_5^{-1} 8_4^{-2} 3^1$          | $\Pi_{(3,0)} 4_3^{-1} 8_4^{-2}$       | —  | —     | 128        |
| 59F1.7   | 16    | $C_4 \circ D_8 \mid [16, 13]$    | $\Pi_{(0,20)} 2_1^1 4_5^{-1} 8^2 3^1$         | $\Pi_{(3,1)} 2_1^1 4_1^1 8^2$         | —  | —     | 32         |
| 59F1.8   | 16    | $C_2^2 \times C_4 \mid [16, 10]$ | $\Pi_{(0,20)} 4_5^{-3} 8_5^{-1} 3^1$          | $\Pi_{(3,1)} 4_1^3 8_1^1$             | —  | —     | 32         |
| 59F1.9   | 16    | $C_4 \circ D_8 \mid [16, 13]$    | $\Pi_{(0,20)} 2_6^2 8_0^2 3^1$                | $\Pi_{(3,1)} 2_2^2 8_0^2$             | —  | —     | 64         |
| 59F1.10  | 16    | $C_2^2 \times C_4 \mid [16, 10]$ | $\Pi_{(0,20)} 2^{-2} 8_6^{-2} 3^1$            | $\Pi_{(3,1)} 2^{-2} 8_2^{-2}$         | —  | —     | 64         |
| 59F1.11  | 16    | $C_2^2 \times C_4 \mid [16, 10]$ | $\Pi_{(0,20)} 2_4^{-2} 4_5^{-1} 8_5^{-1} 3^1$ | $\Pi_{(3,1)} 2_4^{-2} 4_1^1 8_5^{-1}$ | —  | —     | 96         |
| 59F1.12  | 16    | $C_4 \circ D_8 \mid [16, 13]$    | $\Pi_{(0,20)} 2_7^{-3} 16_3^{-1} 3^1$         | $\Pi_{(3,1)} 2_1^{-3} 16_5^{-1}$      | —  | —     | 32         |
| 59F1.13  | 16    | $C_2 \times D_8 \mid [16, 11]$   | $\Pi_{(0,19)} 2_6^{-2} 4_4^{-2} 8_5^{-1} 3^1$ | $\Pi_{(3,2)} 2_4^{-2} 4_0^2 8_5^{-1}$ | —  | —     | —          |
| 59F1.14  | 16    | $C_4 \circ D_8 \mid [16, 13]$    | $\Pi_{(0,19)} 2_3^3 8^{-2} 3^1$               | $\Pi_{(3,2)} 2_1^{-3} 8^{-2}$         | —  | —     | —          |
| 60C1     | 6     | $S_3 \mid [6, 1]$                | $\Pi_{(0,18)} 2_2^{-6} 3^{-2}$                | $\Pi_{(3,3)} 2_6^{-6} 3^1$            | —  | —     | 12         |
| 60C1.1   | 12    | $D_{12} \mid [12, 4]$            | $\Pi_{(0,20)} 2_6^{-2} 4_2^{-2} 3^{-2}$       | $\Pi_{(3,1)} 2_0^2 4_4^{-2} 3^1$      | —  | —     | 48         |
| 60C1.2   | 12    | $D_{12} \mid [12, 4]$            | $\Pi_{(0,20)} 2_6^2 4^2 3^1$                  | $\Pi_{(3,1)} 2_6^{-2} 4^{-2}$         | —  | —     | 768        |
| 60C1.3   | 12    | $D_{12} \mid [12, 4]$            | $\Pi_{(0,19)} 2_6^4 4_7^1 3^{-2}$             | $\Pi_{(3,2)} 2_0^4 4_3^{-1} 3^1$      | —  | —     | 24         |
| 60C1.4   | 12    | $D_{12} \mid [12, 4]$            | $\Pi_{(0,18)} 2_6^6 3^{-2}$                   | $\Pi_{(3,3)} 2_6^{-6} 3^1$            | —  | —     | —          |
| 60F1     | 6     | $S_3 \mid [6, 1]$                | $\Pi_{(0,18)} 2_2^{-6} 3^{-2}$                | $\Pi_{(3,3)} 2_6^{-6} 3^{-3}$         | —  | —     | —          |
| 60F1.1   | 12    | $D_{12} \mid [12, 4]$            | $\Pi_{(0,21)} 2_0^2 4_7^1 3^2$                | $\Pi_{(3,0)} 2_4^{-2} 4_1^1 3^{-1}$   | —  | —     | 1440       |
| 60F1.2   | 12    | $D_{12} \mid [12, 4]$            | $\Pi_{(0,20)} 2_2^{-2} 4^2 3^{-3}$            | $\Pi_{(3,1)} 2_6^{-2} 4^{-2} 3^{-2}$  | —  | —     | —          |
| 60F1.3   | 12    | $D_{12} \mid [12, 4]$            | $\Pi_{(0,20)} 2_6^{-2} 4_6^2 3^2$             | $\Pi_{(3,1)} 2_4^{-2} 4_0^2 3^{-1}$   | —  | —     | 48         |
| 61C1     | 6     | $S_3 \mid [6, 1]$                | $\Pi_{(0,18)} 2_6^{-6} 3^{-4}$                | $\Pi_{(3,3)} 2_2^{-6} 3^3$            | —  | —     | 12         |
| 61C1.1   | 12    | $D_{12} \mid [12, 4]$            | $\Pi_{(0,20)} 2_2^2 4^{-2} 3^3$               | $\Pi_{(3,1)} 2_6^2 4^2 3^2$           | —  | —     | 48         |
| 61C1.2   | 12    | $D_{12} \mid [12, 4]$            | $\Pi_{(0,20)} 2_6^{-2} 4_2^2 3^{-2}$          | $\Pi_{(3,1)} 2_0^2 4_4^{-2} 3^1$      | —  | —     | 48         |
| 61C1.3   | 12    | $D_{12} \mid [12, 4]$            | $\Pi_{(0,19)} 2_6^4 4_1^1 3^{-3}$             | $\Pi_{(3,2)} 2_0^4 4_1^1 3^{-2}$      | —  | —     | 24         |
| 61C1.4   | 12    | $D_{12} \mid [12, 4]$            | $\Pi_{(0,18)} 2_2^6 3^{-4}$                   | $\Pi_{(3,3)} 2_2^{-6} 3^3$            | —  | —     | —          |
| 61F1     | 6     | $S_3 \mid [6, 1]$                | $\Pi_{(0,18)} 2_6^{-6} 3^{-4}$                | $\Pi_{(3,3)} 2_2^{-6} 3^{-5}$         | —  | —     | —          |
| 61F1.1   | 12    | $D_{12} \mid [12, 4]$            | $\Pi_{(0,21)} 4_1^3 3^3$                      | $\Pi_{(3,0)} 4_7^3 3^2$               | —  | —     | 24         |
| 61F1.2   | 12    | $D_{12} \mid [12, 4]$            | $\Pi_{(0,21)} 2_0^2 4_1^1 3^3$                | $\Pi_{(3,0)} 2_6^2 4_1^1 3^2$         | —  | —     | 144        |
| 61F1.3   | 12    | $D_{12} \mid [12, 4]$            | $\Pi_{(0,20)} 2_6^{-2} 4^{-2} 3^{-5}$         | $\Pi_{(3,1)} 2_6^2 4^2 3^{-4}$        | —  | —     | —          |
| 61F1.4   | 12    | $D_{12} \mid [12, 4]$            | $\Pi_{(0,20)} 2_2^2 4_2^{-2} 3^4$             | $\Pi_{(3,1)} 2^{-2} 4_0^2 3^{-3}$     | —  | —     | —          |
| 61F1.5   | 12    | $D_{12} \mid [12, 4]$            | $\Pi_{(0,20)} 2_2^2 4_2^{-2} 3^4$             | $\Pi_{(3,1)} 2_0^2 4_4^{-2} 3^{-3}$   | —  | —     | —          |
| 63C1     | 6     | $C_6 \mid [6, 2]$                | $\Pi_{(0,18)} 2_0^6 3^{-3}$                   | $\Pi_{(3,3)} 2_0^6 3^{-2}$            | —  | —     | 12         |
| 63C1.1   | 12    | $D_{12} \mid [12, 4]$            | $\Pi_{(0,20)} 2_2^2 4_2^{-2} 3^{-2}$          | $\Pi_{(3,1)} 2_0^2 4_4^{-2} 3^1$      | —  | —     | 48         |
| 63C1.2   | 12    | $C_2 \times C_6 \mid [12, 5]$    | $\Pi_{(0,19)} 2_2^4 4_5^{-1} 3^{-3}$          | $\Pi_{(3,2)} 2_0^4 4_1^1 3^{-2}$      | —  | —     | 24         |

Table 2: Birational symplectic effective  $\chi$ -saturated groups

| $(X, G)$ | $\#G$ | Description of $G$               | $g(\Lambda_G)$                                 | $g(\Lambda^G)$                             | K3 | Cubic | Saturation |
|----------|-------|----------------------------------|------------------------------------------------|--------------------------------------------|----|-------|------------|
| 63C1.3   | 12    | $C_2 \times C_6 \mid [12, 5]$    | $\Pi_{(0,19)} 2_4^{-4} 4_5^{-1} 3^{-2}$        | $\Pi_{(3,2)} 2_0^4 4_3^{-1} 3^1$           | —  | —     | 24         |
| 63C1.4   | 12    | $D_{12} \mid [12, 4]$            | $\Pi_{(0,18)} 2_4^{-6} 3^{-3}$                 | $\Pi_{(3,3)} 2_0^6 3^{-2}$                 | —  | —     | —          |
| 63F1     | 6     | $C_6 \mid [6, 2]$                | $\Pi_{(0,18)} 2_0^6 3^{-3}$                    | $\Pi_{(3,3)} 2_0^6 3^4$                    | —  | —     | —          |
| 63F1.1   | 12    | $C_2 \times C_6 \mid [12, 5]$    | $\Pi_{(0,21)} 4_1^3 3^3$                       | $\Pi_{(3,0)} 4_7^3 3^2$                    | —  | —     | 24         |
| 63F1.2   | 12    | $C_2 \times C_6 \mid [12, 5]$    | $\Pi_{(0,21)} 2_2^{-2} 4_3^{-1} 3^3$           | $\Pi_{(3,0)} 2_6^2 4_1^1 3^2$              | —  | —     | 144        |
| 63F1.3   | 12    | $C_2 \times C_6 \mid [12, 5]$    | $\Pi_{(0,21)} 2_6^{-2} 4_5^{-1} 3^2$           | $\Pi_{(3,0)} 2_4^{-2} 4_1^1 3^{-1}$        | —  | —     | 1440       |
| 63F1.4   | 12    | $D_{12} \mid [12, 4]$            | $\Pi_{(0,20)} 2_2^{-2} 4_4^{-2} 3^3$           | $\Pi_{(3,1)} 2_0^2 4_6^2 3^2$              | —  | —     | —          |
| 68C1     | 972   | [972, 776]                       | $\Pi_{(0,19)} 2_1^1 3^{-4}$                    | $\Pi_{(3,2)} 2_7^1 3^3$                    | —  | ×     | 1944       |
| 68C1.1   | 1944  | [1944, 3498]                     | $\Pi_{(0,21)} 2_5^3 3^{-3}$                    | $\Pi_{(3,0)} 2_3^3 3^{-2}$                 | —  | —     | 3888       |
| 68C1.2   | 1944  | [1944, 3559]                     | $\Pi_{(0,21)} 2_7^{-3} 3^{-2}$                 | $\Pi_{(3,0)} 2_1^{-3} 3^1$                 | —  | —     | 7776       |
| 68C1.3   | 1944  | [1944, 3498]                     | $\Pi_{(0,20)} 2_6^{-2} 3^3$                    | $\Pi_{(3,1)} 2_6^2 3^2$                    | —  | ×     | 3888       |
| 68C1.4   | 1944  | [1944, 3536]                     | $\Pi_{(0,19)} 2_5^{-1} 3^{-4}$                 | $\Pi_{(3,2)} 2_7^1 3^3$                    | —  | ×     | —          |
| 68F1     | 972   | [972, 776]                       | $\Pi_{(0,19)} 2_1^1 3^{-4}$                    | $\Pi_{(3,2)} 2_7^1 3^{-5}$                 | —  | —     | —          |
| 69F1     | 960   | $M_{20} \mid [960, 11357]$       | $\Pi_{(0,19)} 2^{-2} 8_1^1 5^{-1}$             | $\Pi_{(3,2)} 2^{-2} 8_7^1 3^1 5^{-1}$ (81) | —  | —     | —          |
| 69F1.1   | 1920  | [1920, 240995]                   | $\Pi_{(0,21)} 2_6^2 8_7^1 3^1$                 | $\Pi_{(3,0)} 2_6^{-2} 8_5^{-1}$            | —  | —     | 23040      |
| 69F1.2   | 1920  | [1920, 240993]                   | $\Pi_{(0,21)} 2_4^{-2} 4_5^{-1} 3^1 5^{-1}$    | $\Pi_{(3,0)} 2_0^2 4_3^{-1} 5^{-1}$        | —  | —     | 3840       |
| 69F1.3   | 1920  | [1920, 240993]                   | $\Pi_{(0,20)} 4_7^1 8_3^{-1} 3^1$              | $\Pi_{(3,1)} 4_1^1 8_5^{-1}$               | —  | —     | 11520      |
| 69F1.4   | 1920  | [1920, 240995]                   | $\Pi_{(0,20)} 4_6^2 3^1 5^{-1}$                | $\Pi_{(3,1)} 4_2^2 5^{-1}$                 | —  | —     | —          |
| 70F1     | 384   | $F_{384} \mid [384, 18135]$      | $\Pi_{(0,19)} 4_3^{-1} 8_6^{-2}$               | $\Pi_{(3,2)} 4_5^{-1} 8_2^{-2} 3^1$ (80)   | —  | —     | —          |
| 70F1.1   | 768   | [768, 1086051]                   | $\Pi_{(0,21)} 2_3^{-1} 4_3^{-1} 16_3^{-1} 3^1$ | $\Pi_{(3,0)} 2_1^1 4_1^1 16_1^1$           | —  | —     | —          |
| 70F1.2   | 768   | [768, 1090134]                   | $\Pi_{(0,21)} 2_2^{-2} 8_7^1 3^1$              | $\Pi_{(3,0)} 2_6^{-2} 8_5^{-1}$            | —  | —     | 23040      |
| 70F1.3   | 768   | [768, 1090134]                   | $\Pi_{(0,21)} 2_6^2 8_3^{-1} 3^1$              | $\Pi_{(3,0)} 2_6^{-2} 8_5^{-1}$            | —  | —     | 23040      |
| 70F1.4   | 768   | [768, 1090134]                   | $\Pi_{(0,20)} 2_4^{-2} 4_7^1 8_7^1 3^1$        | $\Pi_{(3,1)} 2_4^{-2} 4_1^1 8_5^{-1}$      | —  | —     | —          |
| 70F1.5   | 768   | [768, 1090134]                   | $\Pi_{(0,20)} 4_5^{-1} 8_1^1 3^1$              | $\Pi_{(3,1)} 4_1^1 8_5^{-1}$               | —  | —     | 11520      |
| 72C1     | 360   | $A_6 \mid [360, 118]$            | $\Pi_{(0,19)} 4_5^{-1} 3^2 5^1$                | $\Pi_{(3,2)} 4_3^{-1} 3^{-1} 5^1$          | —  | ×     | 720        |
| 72C1.1   | 720   | $C_2 \times A_6 \mid [720, 766]$ | $\Pi_{(0,21)} 2_6^{-2} 4_5^{-1} 3^2$           | $\Pi_{(3,0)} 2_4^{-2} 4_1^1 3^{-1}$        | —  | —     | 1440       |
| 72C1.2   | 720   | $C_2 \times A_6 \mid [720, 766]$ | $\Pi_{(0,20)} 2^{-2} 3^2 5^1$                  | $\Pi_{(3,1)} 2^{-2} 3^{-1} 5^1$            | —  | —     | 1440       |
| 72C1.3   | 720   | $S_6 \mid [720, 763]$            | $\Pi_{(0,19)} 4_5^{-1} 3^2 5^1$                | $\Pi_{(3,2)} 4_3^{-1} 3^{-1} 5^1$          | —  | ×     | —          |
| 72F1     | 360   | $A_6 \mid [360, 118]$            | $\Pi_{(0,19)} 4_5^{-1} 3^2 5^1$                | $\Pi_{(3,2)} 4_3^{-1} 3^3 5^1$ (79)        | ×  | —     | —          |
| 72F1.1   | 720   | $M_{10} \mid [720, 765]$         | $\Pi_{(0,21)} 2_3^3 3^{-2}$                    | $\Pi_{(3,0)} 2_1^{-3} 3^1$                 | —  | —     | 40320      |
| 73C1     | 288   | $A_{4,4} \mid [288, 1026]$       | $\Pi_{(0,19)} 2^2 8_1^1 3^2$                   | $\Pi_{(3,2)} 2^2 8_7^1 3^{-1}$             | —  | —     | 576        |
| 73C1.1   | 576   | [576, 8657]                      | $\Pi_{(0,21)} 2_2^{-2} 8_7^1 3^1$              | $\Pi_{(3,0)} 2_6^{-2} 8_5^{-1}$            | —  | —     | 23040      |
| 73C1.2   | 576   | [576, 8652]                      | $\Pi_{(0,20)} 4_7^1 8_1^1 3^2$                 | $\Pi_{(3,1)} 4_1^1 8_7^1 3^{-1}$           | —  | —     | 1152       |
| 73C1.3   | 576   | [576, 8654]                      | $\Pi_{(0,20)} 4_5^{-1} 8_1^1 3^1$              | $\Pi_{(3,1)} 4_1^1 8_5^{-1}$               | —  | —     | 11520      |
| 73C1.4   | 576   | $S_2^2 \mid [576, 8653]$         | $\Pi_{(0,19)} 2^2 8_1^1 3^2$                   | $\Pi_{(3,2)} 2^2 8_7^1 3^{-1}$             | —  | —     | —          |
| 73F1     | 288   | $A_{4,4} \mid [288, 1026]$       | $\Pi_{(0,19)} 2^2 8_1^1 3^2$                   | $\Pi_{(3,2)} 2^2 8_7^1 3^3$ (78)           | —  | —     | —          |
| 73F1.1   | 576   | [576, 8654]                      | $\Pi_{(0,21)} 2_0^2 4_1^1 3^3$                 | $\Pi_{(3,0)} 2_6^2 4_1^1 3^2$              | —  | —     | 1152       |
| 73F1.2   | 576   | [576, 8652]                      | $\Pi_{(0,21)} 4_7^1 3^2$                       | $\Pi_{(3,0)} 4_1^1 3^{-1}$                 | —  | —     | 6531840    |

Table 2: Birational symplectic effective  $\chi$ -saturated groups

| $(X, G)$ | $\#G$ | Description of $G$              | $g(\Lambda_G)$                          | $g(\Lambda^G)$                    | K3   | Cubic    | Saturation |
|----------|-------|---------------------------------|-----------------------------------------|-----------------------------------|------|----------|------------|
| 73F1.3   | 576   | [576, 8657]                     | $\Pi_{(0,20)}4_2^{-2}3^3$               | $\Pi_{(3,1)}4_6^{-2}3^2$          | —    | —        | —          |
| 74F1     | 192   | $H_{192}$   [192, 955]          | $\Pi_{(0,19)}4_2^{-2}8_1^13^{-1}$       | $\Pi_{(3,2)}4_6^{-2}8_7^13^2$     | (76) | —        | —          |
| 74F1.1   | 384   | [384, 17948]                    | $\Pi_{(0,21)}2_6^28_7^13^1$             | $\Pi_{(3,0)}2_6^{-2}8_5^{-1}$     | —    | —        | 23040      |
| 74F1.2   | 384   | [384, 17948]                    | $\Pi_{(0,20)}2_4^{-2}4_4^{-2}3^{-2}$    | $\Pi_{(3,1)}2_0^24_4^{-2}3^1$     | —    | —        | —          |
| 76C1     | 192   | $T_{192}$   [192, 1493]         | $\Pi_{(0,19)}4_7^33^1$                  | $\Pi_{(3,2)}4_1^{-3}$             | —    | —        | 384        |
| 76C1.1   | 384   | [384, 5602]                     | $\Pi_{(0,21)}2_6^28_3^{-1}3^1$          | $\Pi_{(3,0)}2_6^{-2}8_5^{-1}$     | —    | —        | 23040      |
| 76C1.2   | 384   | [384, 20091]                    | $\Pi_{(0,20)}2_6^24^{-2}3^1$            | $\Pi_{(3,1)}2_6^{-2}4^{-2}$       | —    | —        | 768        |
| 76C1.3   | 384   | [384, 5608]                     | $\Pi_{(0,20)}4_7^18_3^{-1}3^1$          | $\Pi_{(3,1)}4_1^18_5^{-1}$        | —    | —        | 11520      |
| 76C1.4   | 384   | [384, 20089]                    | $\Pi_{(0,19)}4_7^33^1$                  | $\Pi_{(3,2)}4_1^{-3}$             | —    | —        | —          |
| 76F1     | 192   | $T_{192}$   [192, 1493]         | $\Pi_{(0,19)}4_7^33^1$                  | $\Pi_{(3,2)}4_1^{-3}3^{-2}$       | (77) | —        | —          |
| 76F1.1   | 384   | [384, 5608]                     | $\Pi_{(0,21)}2_6^28_1^13^2$             | $\Pi_{(3,0)}2_2^28_3^{-1}3^{-1}$  | —    | —        | 768        |
| 76F1.2   | 384   | [384, 20091]                    | $\Pi_{(0,21)}4_7^13^2$                  | $\Pi_{(3,0)}4_1^13^{-1}$          | —    | —        | 6531840    |
| 76F1.3   | 384   | [384, 5602]                     | $\Pi_{(0,20)}4_7^18_1^13^2$             | $\Pi_{(3,1)}4_1^18_7^13^{-1}$     | —    | —        | —          |
| 77F1     | 168   | $\text{PSL}(2, 7)$   [168, 42]  | $\Pi_{(0,19)}4_1^17^2$                  | $\Pi_{(3,2)}4_1^13^17^2$          | (74) | $\times$ | —          |
| 77F1.1   | 336   | $\text{PGL}(2, 7)$   [336, 208] | $\Pi_{(0,21)}2_3^{-3}3^17^{-1}$         | $\Pi_{(3,0)}2_1^37^1$             | —    | —        | 672        |
| 77F1.2   | 336   | $\text{PGL}(2, 7)$   [336, 208] | $\Pi_{(0,21)}2_3^{-3}3^17^{-1}$         | $\Pi_{(3,0)}2_1^37^1$             | —    | —        | 672        |
| 77F1.3   | 336   | $\text{PGL}(2, 7)$   [336, 208] | $\Pi_{(0,20)}2_3^{-1}4_1^13^17^{-1}$    | $\Pi_{(3,1)}2_7^14_1^17^1$        | —    | $\times$ | —          |
| 80F1     | 128   | [128, 1759]                     | $\Pi_{(0,19)}2_2^{-2}4^{-2}8_7^1$       | $\Pi_{(3,2)}2_2^24^{-2}8_1^13^1$  | —    | —        | —          |
| 80F1.1   | 256   | [256, 26541]                    | $\Pi_{(0,21)}2_2^{-2}8_7^13^1$          | $\Pi_{(3,0)}2_6^{-2}8_5^{-1}$     | —    | —        | 23040      |
| 80F1.2   | 256   | [256, 53387]                    | $\Pi_{(0,21)}2_2^{-2}8_7^13^1$          | $\Pi_{(3,0)}2_6^{-2}8_5^{-1}$     | —    | —        | 23040      |
| 80F1.3   | 256   | [256, 26541]                    | $\Pi_{(0,20)}2_2^{-2}8_0^23^1$          | $\Pi_{(3,1)}2_2^28_0^2$           | —    | —        | —          |
| 80F1.4   | 256   | [256, 53387]                    | $\Pi_{(0,20)}2_6^24^{-2}3^1$            | $\Pi_{(3,1)}2_6^{-2}4^{-2}$       | —    | —        | 768        |
| 82C1     | 120   | $S_5$   [120, 34]               | $\Pi_{(0,19)}4_3^{-1}3^15^{-2}$         | $\Pi_{(3,2)}4_5^{-1}5^{-2}$       | —    | $\times$ | 240        |
| 82C1.1   | 240   | $C_2 \times S_5$   [240, 189]   | $\Pi_{(0,21)}2_4^{-2}4_5^{-1}3^15^{-1}$ | $\Pi_{(3,0)}2_0^24_3^{-1}5^{-1}$  | —    | —        | 480        |
| 82C1.2   | 240   | $C_2 \times S_5$   [240, 189]   | $\Pi_{(0,19)}4_3^{-1}3^15^{-2}$         | $\Pi_{(3,2)}4_5^{-1}5^{-2}$       | —    | $\times$ | —          |
| 82F1     | 120   | $S_5$   [120, 34]               | $\Pi_{(0,19)}4_3^{-1}3^15^{-2}$         | $\Pi_{(3,2)}4_5^{-1}3^{-2}5^{-2}$ | (70) | $\times$ | —          |
| 82F1.1   | 240   | $C_2 \times S_5$   [240, 189]   | $\Pi_{(0,21)}2_2^24_7^13^15^1$          | $\Pi_{(3,0)}2_4^{-2}4_7^15^1$     | —    | —        | —          |
| 82F1.2   | 240   | $C_2 \times S_5$   [240, 189]   | $\Pi_{(0,21)}2_6^24_3^{-1}3^15^1$       | $\Pi_{(3,0)}2_4^{-2}4_7^15^1$     | —    | —        | —          |
| 82F1.3   | 240   | $C_2 \times S_5$   [240, 189]   | $\Pi_{(0,20)}2^{-2}3^25^1$              | $\Pi_{(3,1)}2^{-2}3^{-1}5^1$      | —    | —        | 1440       |
| 84F1     | 72    | $M_9$   [72, 41]                | $\Pi_{(0,19)}2_3^33^{-1}9^{-1}$         | $\Pi_{(3,2)}2_5^33^29^1$          | (63) | $\times$ | —          |
| 84F1.1   | 144   | $C_2 \times M_9$   [144, 187]   | $\Pi_{(0,21)}2_7^{-3}3^{-2}$            | $\Pi_{(3,0)}2_1^{-3}3^1$          | —    | —        | 40320      |
| 84F1.2   | 144   | $C_2 \times M_9$   [144, 187]   | $\Pi_{(0,21)}2_7^{-3}3^{-2}$            | $\Pi_{(3,0)}2_1^{-3}3^1$          | —    | —        | 7776       |
| 85C1     | 72    | $N_{72}$   [72, 40]             | $\Pi_{(0,19)}4_1^13^29^{-1}$            | $\Pi_{(3,2)}4_7^13^{-1}9^1$       | —    | $\times$ | 144        |
| 85C1.1   | 144   | [144, 186]                      | $\Pi_{(0,19)}4_1^13^29^{-1}$            | $\Pi_{(3,2)}4_7^13^{-1}9^1$       | —    | $\times$ | —          |
| 85F1     | 72    | $N_{72}$   [72, 40]             | $\Pi_{(0,19)}4_1^13^29^{-1}$            | $\Pi_{(3,2)}4_7^13^39^1$          | (62) | —        | —          |
| 85F1.1   | 144   | [144, 186]                      | $\Pi_{(0,21)}2_4^{-2}4_1^13^3$          | $\Pi_{(3,0)}2_6^24_1^13^2$        | —    | —        | —          |
| 87F1     | 48    | $T_{48}$   [48, 29]             | $\Pi_{(0,19)}2_3^{-1}8^{-2}3^{-1}$      | $\Pi_{(3,2)}2_1^18^{-2}3^2$       | (54) | $\times$ | —          |
| 87F1.1   | 96    | [96, 190]                       | $\Pi_{(0,21)}2_7^18^{-2}3^{-2}$         | $\Pi_{(3,0)}2_1^18^{-2}3^1$       | —    | —        | —          |

Table 2: Birational symplectic effective  $\chi$ -saturated groups

| $(X, G)$ | $\#G$ | Description of $G$                 | $g(\Lambda_G)$                            | $g(\Lambda^G)$                      | K3 | Cubic | Saturation |
|----------|-------|------------------------------------|-------------------------------------------|-------------------------------------|----|-------|------------|
| 87F1.2   | 96    | [96, 193]                          | $\Pi_{(0,21)}2_2^{-2}16_5^{-1}3^{-2}$     | $\Pi_{(3,0)}2_2^216_3^{-1}3^1$      | —  | —     | —          |
| 89F1     | 32    | $\text{Aut}(D_8) \mid [32, 43]$    | $\Pi_{(0,19)}2_1^{-3}8^2$                 | $\Pi_{(3,2)}2_7^{-3}8^23^1$         | —  | —     | —          |
| 89F1.1   | 64    | [64, 256]                          | $\Pi_{(0,21)}4_3^{-1}8_6^{-2}3^1$         | $\Pi_{(3,0)}4_3^{-1}8_4^{-2}$       | —  | —     | 128        |
| 89F1.2   | 64    | $D_8 \circ D_{16} \mid [64, 257]$  | $\Pi_{(0,21)}4_5^{-1}8_4^{-2}3^1$         | $\Pi_{(3,0)}4_3^{-1}8_4^{-2}$       | —  | —     | 128        |
| 89F1.3   | 64    | $D_8 \circ D_{16} \mid [64, 257]$  | $\Pi_{(0,21)}2_6^28_3^{-1}3^1$            | $\Pi_{(3,0)}2_6^{-2}8_5^{-1}$       | —  | —     | 23040      |
| 89F1.4   | 64    | $D_8 \circ D_{16} \mid [64, 257]$  | $\Pi_{(0,20)}2_6^28_4^{-2}3^1$            | $\Pi_{(3,1)}2_2^28_0^2$             | —  | —     | —          |
| 89F1.5   | 64    | [64, 256]                          | $\Pi_{(0,20)}2^{-2}8_6^{-2}3^1$           | $\Pi_{(3,1)}2^{-2}8_2^{-2}$         | —  | —     | —          |
| 92C1     | 24    | $S_4 \mid [24, 12]$                | $\Pi_{(0,19)}2_6^48_1^13^1$               | $\Pi_{(3,2)}2_2^48_7^1$             | —  | —     | 48         |
| 92C1.1   | 48    | $C_2 \times S_4 \mid [48, 48]$     | $\Pi_{(0,21)}2_6^28_7^13^1$               | $\Pi_{(3,0)}2_6^{-2}8_5^{-1}$       | —  | —     | 23040      |
| 92C1.2   | 48    | $C_2 \times S_4 \mid [48, 48]$     | $\Pi_{(0,20)}2_6^{-2}4_5^{-1}8_3^{-1}3^1$ | $\Pi_{(3,1)}2_4^{-2}4_1^18_5^{-1}$  | —  | —     | 96         |
| 92C1.3   | 48    | $C_2 \times S_4 \mid [48, 48]$     | $\Pi_{(0,20)}2_2^{-2}4^23^1$              | $\Pi_{(3,1)}2_6^{-2}4^{-2}$         | —  | —     | 768        |
| 92C1.4   | 48    | $C_2 \times S_4 \mid [48, 48]$     | $\Pi_{(0,19)}2_6^48_5^{-1}3^1$            | $\Pi_{(3,2)}2_2^48_7^1$             | —  | —     | —          |
| 92F1     | 24    | $S_4 \mid [24, 12]$                | $\Pi_{(0,19)}2_6^48_1^13^1$               | $\Pi_{(3,2)}2_2^48_7^13^{-2}$       | —  | —     | —          |
| 92F1.1   | 48    | $C_2 \times S_4 \mid [48, 48]$     | $\Pi_{(0,21)}2_2^{-2}8_5^{-1}3^2$         | $\Pi_{(3,0)}2_2^28_3^{-1}3^{-1}$    | —  | —     | 768        |
| 92F1.2   | 48    | $C_2 \times S_4 \mid [48, 48]$     | $\Pi_{(0,21)}2_4^{-2}4_7^13^2$            | $\Pi_{(3,0)}2_4^{-2}4_1^13^{-1}$    | —  | —     | 1440       |
| 92F1.3   | 48    | $C_2 \times S_4 \mid [48, 48]$     | $\Pi_{(0,20)}2_0^24_0^23^2$               | $\Pi_{(3,1)}2_4^{-2}4_0^23^{-1}$    | —  | —     | —          |
| 94F1     | 16    | $C_2 \times Q_8 \mid [16, 12]$     | $\Pi_{(0,19)}2_4^416_1^1$                 | $\Pi_{(3,2)}2_0^{-4}16_7^13^1$      | —  | —     | —          |
| 94F1.1   | 32    | $\Gamma_{6a_2} \mid [32, 44]$      | $\Pi_{(0,21)}2_7^14_3^{-1}16_3^{-1}3^1$   | $\Pi_{(3,0)}2_1^14_1^116_1^1$       | —  | —     | 64         |
| 94F1.2   | 32    | $2_-^{1+4} \mid [32, 50]$          | $\Pi_{(0,20)}2_3^316_3^{-1}3^1$           | $\Pi_{(3,1)}2_1^{-3}16_5^{-1}$      | —  | —     | —          |
| 95F1     | 16    | $C_2 \times D_8 \mid [16, 11]$     | $\Pi_{(0,19)}2_0^24_5^{-1}8_0^2$          | $\Pi_{(3,2)}2_0^24_3^{-1}8_0^23^1$  | —  | —     | —          |
| 95F1.1   | 32    | $2_+^{1+4} \mid [32, 49]$          | $\Pi_{(0,21)}4_3^{-1}8_6^{-2}3^1$         | $\Pi_{(3,0)}4_3^{-1}8_4^{-2}$       | —  | —     | 128        |
| 95F1.2   | 32    | $C_2^2 \times D_8 \mid [32, 46]$   | $\Pi_{(0,21)}4_7^38_6^23^1$               | $\Pi_{(3,0)}4_3^{-1}8_4^{-2}$       | —  | —     | 128        |
| 95F1.3   | 32    | $\text{Aut}(D_{16}) \mid [32, 43]$ | $\Pi_{(0,21)}2_1^14_5^{-1}16_7^13^1$      | $\Pi_{(3,0)}2_1^14_1^116_1^1$       | —  | —     | 64         |
| 95F1.4   | 32    | $C_2^2 \times D_8 \mid [32, 46]$   | $\Pi_{(0,21)}2_2^{-2}8_7^13^1$            | $\Pi_{(3,0)}2_6^{-2}8_5^{-1}$       | —  | —     | 23040      |
| 95F1.5   | 32    | $2_+^{1+4} \mid [32, 49]$          | $\Pi_{(0,20)}2_5^{-1}4_5^{-1}8^23^1$      | $\Pi_{(3,1)}2_1^14_1^18^2$          | —  | —     | —          |
| 95F1.6   | 32    | $C_2^2 \times D_8 \mid [32, 46]$   | $\Pi_{(0,20)}4_7^38_7^13^1$               | $\Pi_{(3,1)}4_1^38_1^1$             | —  | —     | —          |
| 95F1.7   | 32    | $C_2^2 \times D_8 \mid [32, 46]$   | $\Pi_{(0,20)}2_2^24_5^{-1}8_7^13^1$       | $\Pi_{(3,1)}2_4^{-2}4_1^18_5^{-1}$  | —  | —     | 96         |
| 97C1     | 12    | $D_{12} \mid [12, 4]$              | $\Pi_{(0,19)}2_2^{-4}4_7^13^{-2}$         | $\Pi_{(3,2)}2_0^44_3^{-1}3^1$       | —  | —     | 24         |
| 97C1.1   | 24    | $C_2^2 \times S_3 \mid [24, 14]$   | $\Pi_{(0,20)}2_0^24_4^{-2}3^{-2}$         | $\Pi_{(3,1)}2_0^24_4^{-2}3^1$       | —  | —     | 48         |
| 97C1.2   | 24    | $C_2^2 \times S_3 \mid [24, 14]$   | $\Pi_{(0,19)}2_6^44_7^13^{-2}$            | $\Pi_{(3,2)}2_0^44_3^{-1}3^1$       | —  | —     | —          |
| 97F1     | 12    | $D_{12} \mid [12, 4]$              | $\Pi_{(0,19)}2_2^{-4}4_7^13^{-2}$         | $\Pi_{(3,2)}2_0^44_3^{-1}3^{-3}$    | —  | —     | —          |
| 97F1.1   | 24    | $C_2^2 \times S_3 \mid [24, 14]$   | $\Pi_{(0,21)}2_0^24_7^13^2$               | $\Pi_{(3,0)}2_4^{-2}4_1^13^{-1}$    | —  | —     | 1440       |
| 98C1     | 12    | $D_{12} \mid [12, 4]$              | $\Pi_{(0,19)}2_6^{-4}4_5^{-1}3^{-3}$      | $\Pi_{(3,2)}2_2^{-4}4_3^{-1}3^{-2}$ | —  | —     | 24         |
| 98C1.1   | 24    | $C_2^2 \times S_3 \mid [24, 14]$   | $\Pi_{(0,20)}2_4^{-2}4_4^{-2}3^{-2}$      | $\Pi_{(3,1)}2_0^24_4^{-2}3^1$       | —  | —     | 48         |
| 98C1.2   | 24    | $C_2^2 \times S_3 \mid [24, 14]$   | $\Pi_{(0,19)}2_2^44_5^{-1}3^{-3}$         | $\Pi_{(3,2)}2_2^{-4}4_3^{-1}3^{-2}$ | —  | —     | —          |
| 98F1     | 12    | $D_{12} \mid [12, 4]$              | $\Pi_{(0,19)}2_6^{-4}4_5^{-1}3^{-3}$      | $\Pi_{(3,2)}2_2^{-4}4_3^{-1}3^4$    | —  | —     | —          |
| 98F1.1   | 24    | $C_2^2 \times S_3 \mid [24, 14]$   | $\Pi_{(0,21)}4_1^33^3$                    | $\Pi_{(3,0)}4_7^33^2$               | —  | —     | —          |
| 98F1.2   | 24    | $C_2^2 \times S_3 \mid [24, 14]$   | $\Pi_{(0,21)}2_6^24_3^{-1}3^3$            | $\Pi_{(3,0)}2_6^24_1^13^2$          | —  | —     | 144        |

Table 2: Birational symplectic effective  $\chi$ -saturated groups

| $(X, G)$ | $\#G$ | Description of $G$                 | $g(\Lambda_G)$                              | $g(\Lambda^G)$                          | K3 | Cubic | Saturation |
|----------|-------|------------------------------------|---------------------------------------------|-----------------------------------------|----|-------|------------|
| 101C1    | 29160 | $C_3^4 \rtimes A_6$                | $\Pi_{(0,20)} 3^2 9^1$                      | $\Pi_{(3,1)} 3^{-1} 9^{-1}$             | —  | ×     | 58320      |
| 101C1.1  | 58320 | $C_3^4 \rtimes S_6$                | $\Pi_{(0,20)} 3^2 9^1$                      | $\Pi_{(3,1)} 3^{-1} 9^{-1}$             | —  | ×     | —          |
| 101F1    | 29160 | $C_3^4 \rtimes A_6$                | $\Pi_{(0,20)} 3^2 9^1$                      | $\Pi_{(3,1)} 3^3 9^{-1}$                | —  | —     | —          |
| 102F1    | 20160 | $\text{PSL}(3, 4)$                 | $\Pi_{(0,20)} 2^{-2} 3^{-1} 7^{-1}$         | $\Pi_{(3,1)} 2^{-2} 3^2 7^1$            | —  | —     | —          |
| 102F1.1  | 40320 | $\text{PSL}(3, 4) \rtimes C_2$     | $\Pi_{(0,21)} 2_3^3 3^{-2}$                 | $\Pi_{(3,0)} 2_1^{-3} 3^1$              | —  | —     | —          |
| 106C1    | 5760  | $C_2^4 \rtimes A_6$                | $\Pi_{(0,20)} 4_7^1 8_3^{-1} 3^1$           | $\Pi_{(3,1)} 4_1^1 8_5^{-1}$            | —  | —     | 11520      |
| 106C1.1  | 11520 | $(C_2^4 \rtimes A_6) \rtimes C_2$  | $\Pi_{(0,21)} 2_6^2 8_3^{-1} 3^1$           | $\Pi_{(3,0)} 2_6^{-2} 8_5^{-1}$         | —  | —     | 23040      |
| 106C1.2  | 11520 | $C_2^4 \rtimes S_6$                | $\Pi_{(0,20)} 4_7^1 8_3^{-1} 3^1$           | $\Pi_{(3,1)} 4_1^1 8_5^{-1}$            | —  | —     | —          |
| 106F1    | 5760  | $C_2^4 \rtimes A_6$                | $\Pi_{(0,20)} 4_7^1 8_3^{-1} 3^1$           | $\Pi_{(3,1)} 4_1^1 8_5^{-1} 3^{-2}$     | —  | —     | —          |
| 106F1.1  | 11520 | $(C_2^4 \rtimes A_6) \rtimes C_2$  | $\Pi_{(0,21)} 4_7^1 3^2$                    | $\Pi_{(3,0)} 4_1^1 3^{-1}$              | —  | —     | 6531840    |
| 108C1    | 2520  | $A_7$                              | $\Pi_{(0,20)} 3^1 5^1 7^1$                  | $\Pi_{(3,1)} 5^1 7^{-1}$                | —  | ×     | 5040       |
| 108C1.1  | 5040  | $S_7$                              | $\Pi_{(0,20)} 3^1 5^1 7^1$                  | $\Pi_{(3,1)} 5^1 7^{-1}$                | —  | ×     | —          |
| 108F1    | 2520  | $A_7$                              | $\Pi_{(0,20)} 3^1 5^1 7^1$                  | $\Pi_{(3,1)} 3^{-2} 5^1 7^{-1}$         | —  | ×     | —          |
| 109C1    | 1944  | [1944, 3559]                       | $\Pi_{(0,20)} 2_6^{-2} 3^3$                 | $\Pi_{(3,1)} 2_6^2 3^2$                 | —  | ×     | 3888       |
| 109C1.1  | 3888  | —                                  | $\Pi_{(0,21)} 4_1^1 3^3$                    | $\Pi_{(3,0)} 4_7^1 3^2$                 | —  | —     | 7776       |
| 109C1.2  | 3888  | —                                  | $\Pi_{(0,21)} 2_3^3 3^{-2}$                 | $\Pi_{(3,0)} 2_1^{-3} 3^1$              | —  | —     | 7776       |
| 109C1.3  | 3888  | —                                  | $\Pi_{(0,21)} 4_1^1 3^2$                    | $\Pi_{(3,0)} 4_1^1 3^{-1}$              | —  | —     | 6531840    |
| 109C1.4  | 3888  | —                                  | $\Pi_{(0,20)} 2_6^{-2} 3^3$                 | $\Pi_{(3,1)} 2_6^2 3^2$                 | —  | ×     | —          |
| 109F1    | 1944  | [1944, 3559]                       | $\Pi_{(0,20)} 2_6^{-2} 3^3$                 | $\Pi_{(3,1)} 2_6^2 3^{-4}$              | —  | —     | —          |
| 110F1    | 1920  | [1920, 240993]                     | $\Pi_{(0,20)} 4_5^{-1} 8_7^1 5^{-1}$        | $\Pi_{(3,1)} 4_3^{-1} 8_1^1 3^1 5^{-1}$ | —  | —     | —          |
| 110F1.1  | 3840  | $C_2^5 \rtimes S_5$                | $\Pi_{(0,21)} 2_2^{-2} 8_7^1 3^1$           | $\Pi_{(3,0)} 2_6^{-2} 8_5^{-1}$         | —  | —     | 23040      |
| 110F1.2  | 3840  | $C_2^5 \rtimes S_5$                | $\Pi_{(0,21)} 2_4^{-2} 4_5^{-1} 3^1 5^{-1}$ | $\Pi_{(3,0)} 2_0^2 4_3^{-1} 5^{-1}$     | —  | —     | —          |
| 111F1    | 1344  | [1344, 11686]                      | $\Pi_{(0,20)} 4_2^2 7^1$                    | $\Pi_{(3,1)} 4_6^2 3^1 7^{-1}$          | —  | —     | —          |
| 112F1    | 1152  | [1152, 155478]                     | $\Pi_{(0,20)} 8_6^{-2} 3^{-1}$              | $\Pi_{(3,1)} 8_2^{-2} 3^2$              | —  | —     | —          |
| 114C1    | 972   | [972, 812]                         | $\Pi_{(0,20)} 2^{-2} 3^4$                   | $\Pi_{(3,1)} 2^{-2} 3^{-3}$             | —  | —     | 1944       |
| 114C1.1  | 1944  | [1944, 3579]                       | $\Pi_{(0,21)} 2_5^3 3^{-3}$                 | $\Pi_{(3,0)} 2_3^3 3^{-2}$              | —  | —     | 3888       |
| 114C1.2  | 1944  | [1944, 3499]                       | $\Pi_{(0,21)} 4_1^1 3^3$                    | $\Pi_{(3,0)} 4_7^1 3^2$                 | —  | —     | 7776       |
| 114C1.3  | 1944  | [1944, 3537]                       | $\Pi_{(0,20)} 2^{-2} 3^4$                   | $\Pi_{(3,1)} 2^{-2} 3^{-3}$             | —  | —     | —          |
| 116F1    | 768   | [768, 1090135]                     | $\Pi_{(0,20)} 2_6^2 8_2^{-2}$               | $\Pi_{(3,1)} 2_2^2 8_6^{-2} 3^1$        | —  | —     | —          |
| 116F1.1  | 1536  | —                                  | $\Pi_{(0,21)} 2_2^{-2} 8_7^1 3^1$           | $\Pi_{(3,0)} 2_6^{-2} 8_5^{-1}$         | —  | —     | 23040      |
| 118C1    | 720   | $S_6 \mid [720, 763]$              | $\Pi_{(0,20)} 2^{-2} 3^2 5^1$               | $\Pi_{(3,1)} 2^{-2} 3^{-1} 5^1$         | —  | —     | 1440       |
| 118C1.1  | 1440  | $C_2 \times S_6 \mid [1440, 5842]$ | $\Pi_{(0,20)} 2^{-2} 3^2 5^1$               | $\Pi_{(3,1)} 2^{-2} 3^{-1} 5^1$         | —  | —     | —          |
| 118F1    | 720   | $S_6 \mid [720, 763]$              | $\Pi_{(0,20)} 2^{-2} 3^2 5^1$               | $\Pi_{(3,1)} 2^{-2} 3^3 5^1$            | —  | —     | —          |
| 119F1    | 720   | $M_{10} \mid [720, 765]$           | $\Pi_{(0,20)} 2_3^{-1} 4_1^1 3^{-1} 5^1$    | $\Pi_{(3,1)} 2_5^{-1} 4_1^1 3^2 5^1$    | —  | ×     | —          |
| 120F1    | 660   | $\text{PSL}(2, 11) \mid [660, 13]$ | $\Pi_{(0,20)} 11^2$                         | $\Pi_{(3,1)} 3^1 11^2$                  | —  | ×     | —          |
| 121C1    | 576   | [576, 8654]                        | $\Pi_{(0,20)} 4_7^1 8_1^1 3^2$              | $\Pi_{(3,1)} 4_1^1 8_7^1 3^{-1}$        | —  | —     | 1152       |
| 121C1.1  | 1152  | [1152, 157852]                     | $\Pi_{(0,21)} 2_2^{-2} 8_7^1 3^1$           | $\Pi_{(3,0)} 2_6^{-2} 8_5^{-1}$         | —  | —     | 23040      |
| 121C1.2  | 1152  | [1152, 157849]                     | $\Pi_{(0,20)} 4_7^1 8_1^1 3^2$              | $\Pi_{(3,1)} 4_1^1 8_7^1 3^{-1}$        | —  | —     | —          |

Table 2: Birational symplectic effective  $\chi$ -saturated groups

| $(X, G)$ | $\#G$ | Description of $G$                            | $g(\Lambda_G)$                          | $g(\Lambda^G)$                     | K3 | Cubic    | Saturation |
|----------|-------|-----------------------------------------------|-----------------------------------------|------------------------------------|----|----------|------------|
| 121F1    | 576   | [576, 8654]                                   | $\Pi_{(0,20)}4_7^18_1^13^2$             | $\Pi_{(3,1)}4_1^18_7^13^3$         | —  | —        | —          |
| 121F1.1  | 1152  | [1152, 157852]                                | $\Pi_{(0,21)}2_4^{-2}4_1^13^3$          | $\Pi_{(3,0)}2_6^24_1^13^2$         | —  | —        | —          |
| 122F1    | 500   | [500, 23]                                     | $\Pi_{(0,20)}5^3$                       | $\Pi_{(3,1)}3^15^3$                | —  | —        | —          |
| 123C1    | 384   | [384, 20097]                                  | $\Pi_{(0,20)}2_6^24^{-2}3^1$            | $\Pi_{(3,1)}2_6^{-2}4^{-2}$        | —  | —        | 768        |
| 123C1.1  | 768   | [768, 1088556]                                | $\Pi_{(0,21)}2_6^28_3^{-1}3^1$          | $\Pi_{(3,0)}2_6^{-2}8_5^{-1}$      | —  | —        | 23040      |
| 123C1.2  | 768   | [768, 1090220]                                | $\Pi_{(0,20)}2_6^24^{-2}3^1$            | $\Pi_{(3,1)}2_6^{-2}4^{-2}$        | —  | —        | —          |
| 123F1    | 384   | [384, 20097]                                  | $\Pi_{(0,20)}2_6^24^{-2}3^1$            | $\Pi_{(3,1)}2_6^{-2}4^{-2}3^{-2}$  | —  | —        | —          |
| 123F1.1  | 768   | [768, 1088556]                                | $\Pi_{(0,21)}2_6^28_1^13^2$             | $\Pi_{(3,0)}2_2^28_3^{-1}3^{-1}$   | —  | —        | —          |
| 124F1    | 384   | [384, 18134]                                  | $\Pi_{(0,20)}2_3^316_7^1$               | $\Pi_{(3,1)}2_7^{-3}16_1^13^1$     | —  | —        | —          |
| 128C1    | 360   | $\Gamma L_2(\mathbb{F}_4) \mid [360, 120]$    | $\Pi_{(0,20)}3^{-2}5^{-2}$              | $\Pi_{(3,1)}3^15^{-2}$             | —  | $\times$ | 720        |
| 128C1.1  | 720   | $S_3 \times S_5 \mid [720, 767]$              | $\Pi_{(0,20)}3^{-2}5^{-2}$              | $\Pi_{(3,1)}3^15^{-2}$             | —  | $\times$ | —          |
| 128F1    | 360   | $\Gamma L_2(\mathbb{F}_4) \mid [360, 120]$    | $\Pi_{(0,20)}3^{-2}5^{-2}$              | $\Pi_{(3,1)}3^{-3}5^{-2}$          | —  | —        | —          |
| 129F1    | 336   | $C_2 \times \text{PSL}(3, 2) \mid [336, 209]$ | $\Pi_{(0,20)}2^27^2$                    | $\Pi_{(3,1)}2^23^17^2$             | —  | —        | —          |
| 129F1.1  | 672   | [672, 1254]                                   | $\Pi_{(0,21)}2_3^{-3}3^17^{-1}$         | $\Pi_{(3,0)}2_1^37^1$              | —  | —        | —          |
| 129F1.2  | 672   | [672, 1254]                                   | $\Pi_{(0,21)}2_3^{-3}3^17^{-1}$         | $\Pi_{(3,0)}2_1^37^1$              | —  | —        | —          |
| 131F1    | 192   | [192, 1494]                                   | $\Pi_{(0,20)}2_2^{-2}8_2^{-2}$          | $\Pi_{(3,1)}2_2^28_6^{-2}3^1$      | —  | —        | —          |
| 133F1    | 144   | $C_2 \times M_9 \mid [144, 187]$              | $\Pi_{(0,20)}2_4^49^{-1}$               | $\Pi_{(3,1)}2_0^{-4}3^19^1$        | —  | —        | —          |
| 134F1    | 144   | $\text{AGL}_1(\mathbb{F}_9) \mid [144, 182]$  | $\Pi_{(0,20)}2_7^14_3^{-1}3^{-1}9^{-1}$ | $\Pi_{(3,1)}2_7^14_7^13^29^1$      | —  | —        | —          |
| 137C1    | 120   | $S_5 \mid [120, 34]$                          | $\Pi_{(0,20)}2_6^43^15^{-1}$            | $\Pi_{(3,1)}2_6^{-4}5^{-1}$        | —  | —        | 240        |
| 137C1.1  | 240   | $C_2 \times S_5 \mid [240, 189]$              | $\Pi_{(0,21)}2_4^{-2}4_5^{-1}3^15^{-1}$ | $\Pi_{(3,0)}2_0^24_3^{-1}5^{-1}$   | —  | —        | 480        |
| 137C1.2  | 240   | $C_2 \times S_5 \mid [240, 189]$              | $\Pi_{(0,20)}2_6^43^15^{-1}$            | $\Pi_{(3,1)}2_6^{-4}5^{-1}$        | —  | —        | —          |
| 137F1    | 120   | $S_5 \mid [120, 34]$                          | $\Pi_{(0,20)}2_6^43^15^{-1}$            | $\Pi_{(3,1)}2_6^{-4}3^{-2}5^{-1}$  | —  | —        | —          |
| 137F1.1  | 240   | $C_2 \times S_5 \mid [240, 189]$              | $\Pi_{(0,21)}2_0^24_7^13^2$             | $\Pi_{(3,0)}2_4^{-2}4_1^13^{-1}$   | —  | —        | 1440       |
| 138C1    | 108   | [108, 17]                                     | $\Pi_{(0,20)}3^29^2$                    | $\Pi_{(3,1)}3^{-1}9^2$             | —  | —        | —          |
| 141C1    | 72    | $N_{72} \mid [72, 40]$                        | $\Pi_{(0,20)}2_2^{-4}3^19^{-1}$         | $\Pi_{(3,1)}2_2^49^1$              | —  | —        | 144        |
| 141C1.1  | 144   | [144, 186]                                    | $\Pi_{(0,20)}2_2^{-4}3^19^{-1}$         | $\Pi_{(3,1)}2_2^49^1$              | —  | —        | —          |
| 141F1    | 72    | $N_{72} \mid [72, 40]$                        | $\Pi_{(0,20)}2_2^{-4}3^19^{-1}$         | $\Pi_{(3,1)}2_2^43^{-2}9^1$        | —  | —        | —          |
| 143F1    | 64    | $D_8 \circ D_{16} \mid [64, 257]$             | $\Pi_{(0,20)}2_3^{-1}4_5^{-1}8^2$       | $\Pi_{(3,1)}2_1^14_3^{-1}8^23^1$   | —  | —        | —          |
| 143F1.1  | 128   | [128, 2317]                                   | $\Pi_{(0,21)}4_7^18_6^23^1$             | $\Pi_{(3,0)}4_3^{-1}8_4^{-2}$      | —  | —        | —          |
| 144C1    | 60    | $A_5 \mid [60, 5]$                            | $\Pi_{(0,20)}2^{-2}3^4$                 | $\Pi_{(3,1)}2^{-2}3^{-3}$          | —  | —        | —          |
| 148C1    | 48    | $C_2 \times S_4 \mid [48, 48]$                | $\Pi_{(0,20)}2_4^{-2}4_7^18_7^13^1$     | $\Pi_{(3,1)}2_2^{-2}4_3^{-1}8_1^1$ | —  | —        | 96         |
| 148C1.1  | 96    | $C_2^2 \times S_4 \mid [96, 226]$             | $\Pi_{(0,21)}2_6^28_3^{-1}3^1$          | $\Pi_{(3,0)}2_6^{-2}8_5^{-1}$      | —  | —        | 23040      |
| 148C1.2  | 96    | $C_2^2 \times S_4 \mid [96, 226]$             | $\Pi_{(0,20)}2_0^24_7^18_3^{-1}3^1$     | $\Pi_{(3,1)}2_2^{-2}4_3^{-1}8_1^1$ | —  | —        | —          |
| 148F1    | 48    | $C_2 \times S_4 \mid [48, 48]$                | $\Pi_{(0,20)}2_4^{-2}4_7^18_7^13^1$     | $\Pi_{(3,1)}2_0^24_1^18_1^13^{-2}$ | —  | —        | —          |
| 148F1.1  | 96    | $C_2^2 \times S_4 \mid [96, 226]$             | $\Pi_{(0,21)}2_0^24_7^13^2$             | $\Pi_{(3,0)}2_4^{-2}4_1^13^{-1}$   | —  | —        | 1440       |
| 149F1    | 40    | $C_2 \times F_5 \mid [40, 12]$                | $\Pi_{(0,20)}2_4^45^2$                  | $\Pi_{(3,1)}2_0^{-4}3^15^2$        | —  | —        | —          |
| 149F1.1  | 80    | $C_2^2 \times F_5 \mid [80, 50]$              | $\Pi_{(0,21)}2_6^24_7^13^15^{-1}$       | $\Pi_{(3,0)}2_0^24_3^{-1}5^{-1}$   | —  | —        | 480        |
| 150C1    | 36    | $C_2 \times C_3 \rtimes S_3 \mid [36, 13]$    | $\Pi_{(0,20)}2_0^{-4}3^4$               | $\Pi_{(3,1)}2_0^{-4}3^{-3}$        | —  | —        | 72         |

Table 2: Birational symplectic effective  $\chi$ -saturated groups

| $(X, G)$ | $\#G$   | Description of $G$                           | $g(\Lambda_G)$                              | $g(\Lambda^G)$                          | K3 | Cubic | Saturation |
|----------|---------|----------------------------------------------|---------------------------------------------|-----------------------------------------|----|-------|------------|
| 150C1.1  | 72      | $C_2^2 \times C_3 \rtimes S_3 \mid [72, 49]$ | $\Pi_{(0,21)} 2_4^{-2} 4_1^1 3^3$           | $\Pi_{(3,0)} 2_6^2 4_1^1 3^2$           | —  | —     | 144        |
| 150C1.2  | 72      | $C_2 \times C_3^2 \rtimes C_4 \mid [72, 45]$ | $\Pi_{(0,21)} 2_4^{-2} 4_1^1 3^3$           | $\Pi_{(3,0)} 2_6^2 4_1^1 3^2$           | —  | —     | 144        |
| 150C1.3  | 72      | $C_2 \times S_3^2 \mid [72, 46]$             | $\Pi_{(0,20)} 2_4^4 3^4$                    | $\Pi_{(3,1)} 2_0^{-4} 3^{-3}$           | —  | —     | —          |
| 151C1    | 36      | $S_3^2 \mid [36, 10]$                        | $\Pi_{(0,20)} 2_6^{-4} 3^3$                 | $\Pi_{(3,1)} 2_6^4 3^2$                 | —  | —     | 72         |
| 151C1.1  | 72      | $N_{72} \mid [72, 40]$                       | $\Pi_{(0,21)} 2_4^{-2} 4_1^1 3^3$           | $\Pi_{(3,0)} 2_6^2 4_1^1 3^2$           | —  | —     | 144        |
| 151C1.2  | 72      | $C_2 \times S_3^2 \mid [72, 46]$             | $\Pi_{(0,21)} 2_0^2 4_7^1 3^2$              | $\Pi_{(3,0)} 2_4^{-2} 4_1^1 3^{-1}$     | —  | —     | 1440       |
| 151C1.3  | 72      | $N_{72} \mid [72, 40]$                       | $\Pi_{(0,20)} 2_6^{-4} 3^3$                 | $\Pi_{(3,1)} 2_6^4 3^2$                 | —  | —     | —          |
| 151C2    | 36      | $S_3^2 \mid [36, 10]$                        | $\Pi_{(0,20)} 2_6^{-4} 3^3$                 | $\Pi_{(3,1)} 2_6^4 3^2$                 | —  | —     | 72         |
| 151C2.1  | 72      | $C_2 \times S_3^2 \mid [72, 46]$             | $\Pi_{(0,21)} 2_4^{-2} 4_1^1 3^3$           | $\Pi_{(3,0)} 2_6^2 4_1^1 3^2$           | —  | —     | 144        |
| 151C2.2  | 72      | $N_{72} \mid [72, 40]$                       | $\Pi_{(0,21)} 2_4^{-2} 4_7^1 3^2$           | $\Pi_{(3,0)} 2_4^{-2} 4_1^1 3^{-1}$     | —  | —     | 1440       |
| 151C2.3  | 72      | $C_2 \times S_3^2 \mid [72, 46]$             | $\Pi_{(0,20)} 2_6^{-4} 3^3$                 | $\Pi_{(3,1)} 2_6^4 3^2$                 | —  | —     | —          |
| 151F1    | 36      | $S_3^2 \mid [36, 10]$                        | $\Pi_{(0,20)} 2_6^{-4} 3^3$                 | $\Pi_{(3,1)} 2_6^4 3^{-4}$              | —  | —     | —          |
| 152F1    | 32      | $C_2 \times QD_{16} \mid [32, 40]$           | $\Pi_{(0,20)} 2_4^{-2} 4_3^{-1} 16_1^1$     | $\Pi_{(3,1)} 2_0^2 4_5^{-1} 16_7^1 3^1$ | —  | —     | —          |
| 152F1.1  | 64      | $D_8 \circ QD_{16} \mid [64, 258]$           | $\Pi_{(0,21)} 2_5^{-1} 4_5^{-1} 16_7^1 3^1$ | $\Pi_{(3,0)} 2_1^1 4_1^1 16_1^1$        | —  | —     | —          |
| 154C1    | 24      | $C_2^2 \times S_3 \mid [24, 14]$             | $\Pi_{(0,20)} 2_4^{-2} 4_4^{-2} 3^{-2}$     | $\Pi_{(3,1)} 2_0^2 4_4^{-2} 3^1$        | —  | —     | 48         |
| 154C1.1  | 48      | $D_8 \times S_3 \mid [48, 38]$               | $\Pi_{(0,21)} 2_6^2 8_1^1 3^{-2}$           | $\Pi_{(3,0)} 2_6^2 8_3^{-1} 3^1$        | —  | —     | 288        |
| 154C1.2  | 48      | $D_8 \times S_3 \mid [48, 38]$               | $\Pi_{(0,21)} 2_2^{-2} 8_7^1 3^1$           | $\Pi_{(3,0)} 2_6^{-2} 8_5^{-1}$         | —  | —     | 23040      |
| 154C1.3  | 48      | $C_2^3 \times S_3 \mid [48, 51]$             | $\Pi_{(0,20)} 2_2^2 4_2^2 3^{-2}$           | $\Pi_{(3,1)} 2_0^2 4_4^{-2} 3^1$        | —  | —     | —          |
| 154F1    | 24      | $C_2^2 \times S_3 \mid [24, 14]$             | $\Pi_{(0,20)} 2_4^{-2} 4_4^{-2} 3^{-2}$     | $\Pi_{(3,1)} 2_0^2 4_4^{-2} 3^{-3}$     | —  | —     | —          |
| 154F1.1  | 48      | $D_8 \times S_3 \mid [48, 38]$               | $\Pi_{(0,21)} 2_2^{-2} 8_7^1 3^{-3}$        | $\Pi_{(3,0)} 2_6^{-2} 8_5^{-1} 3^{-2}$  | —  | —     | —          |
| 157C1    | 24      | $D_{24} \mid [24, 6]$                        | $\Pi_{(0,20)} 2_2^2 4^{-2} 3^3$             | $\Pi_{(3,1)} 2_2^{-2} 4^{-2} 3^2$       | —  | —     | 48         |
| 157C1.1  | 48      | $C_2 \times D_{24} \mid [48, 36]$            | $\Pi_{(0,21)} 2_6^{-2} 8_1^1 3^{-2}$        | $\Pi_{(3,0)} 2_6^2 8_3^{-1} 3^1$        | —  | —     | 288        |
| 157C1.2  | 48      | $D_8 \times S_3 \mid [48, 38]$               | $\Pi_{(0,20)} 2_2^2 4^{-2} 3^3$             | $\Pi_{(3,1)} 2_2^{-2} 4^{-2} 3^2$       | —  | —     | —          |
| 157F1    | 24      | $D_{24} \mid [24, 6]$                        | $\Pi_{(0,20)} 2_6^{-2} 4^2 3^3$             | $\Pi_{(3,1)} 2_6^2 4^2 3^{-4}$          | —  | —     | —          |
| 157F1.1  | 48      | $D_8 \times S_3 \mid [48, 38]$               | $\Pi_{(0,21)} 2_2^2 8_1^1 3^4$              | $\Pi_{(3,0)} 2_2^{-2} 8_7^1 3^{-3}$     | —  | —     | —          |
| 161C1    | 12      | $D_{12} \mid [12, 4]$                        | $\Pi_{(0,20)} 2_0^{-4} 3^4$                 | $\Pi_{(3,1)} 2_0^{-4} 3^{-3}$           | —  | —     | —          |
| 163C1    | 3265920 | $\text{PSU}(4, 3)$                           | $\Pi_{(0,21)} 4_7^1 3^2$                    | $\Pi_{(3,0)} 4_1^1 3^{-1}$              | —  | —     | 6531840    |
| 163C1.1  | 6531840 | —                                            | $\Pi_{(0,21)} 4_7^1 3^2$                    | $\Pi_{(3,0)} 4_1^1 3^{-1}$              | —  | —     | —          |
| 163F1    | 3265920 | $\text{PSU}(4, 3)$                           | $\Pi_{(0,21)} 4_7^1 3^2$                    | $\Pi_{(3,0)} 4_1^1 3^3$                 | —  | —     | —          |
| 165F1    | 443520  | $M_{22}$                                     | $\Pi_{(0,21)} 4_5^{-1} 11^1$                | $\Pi_{(3,0)} 4_3^{-1} 3^1 11^{-1}$      | —  | —     | —          |
| 165F2    | 443520  | $M_{22}$                                     | $\Pi_{(0,21)} 4_5^{-1} 11^1$                | $\Pi_{(3,0)} 4_3^{-1} 3^1 11^{-1}$      | —  | —     | —          |
| 167F1    | 126000  | $\text{PSU}(3, 5)$                           | $\Pi_{(0,21)} 2_7^1 5^{-2}$                 | $\Pi_{(3,0)} 2_5^{-1} 3^1 5^{-2}$       | —  | —     | —          |
| 167F2    | 126000  | $\text{PSU}(3, 5)$                           | $\Pi_{(0,21)} 2_7^1 5^{-2}$                 | $\Pi_{(3,0)} 2_1^1 3^1 5^{-2}$          | —  | —     | —          |
| 169F1    | 58320   | —                                            | $\Pi_{(0,21)} 2_5^{-1} 3^{-1} 9^1$          | $\Pi_{(3,0)} 2_3^{-1} 3^2 9^{-1}$       | —  | —     | —          |
| 170F1    | 40320   | —                                            | $\Pi_{(0,21)} 4_3^{-1} 3^{-1} 7^{-1}$       | $\Pi_{(3,0)} 4_5^{-1} 3^2 7^1$          | —  | —     | —          |
| 171F1    | 40320   | —                                            | $\Pi_{(0,21)} 2_5^3 7^{-1}$                 | $\Pi_{(3,0)} 2_7^{-3} 3^1 7^1$          | —  | —     | —          |
| 171F2    | 40320   | —                                            | $\Pi_{(0,21)} 2_5^3 7^{-1}$                 | $\Pi_{(3,0)} 2_7^{-3} 3^1 7^1$          | —  | —     | —          |

Table 2: Birational symplectic effective  $\chi$ -saturated groups

| $(X, G)$ | $\#G$ | Description of $G$                                       | $g(\Lambda_G)$                    | $g(\Lambda^G)$                         | K3 | Cubic | Saturation |
|----------|-------|----------------------------------------------------------|-----------------------------------|----------------------------------------|----|-------|------------|
| 172F1    | 40320 | —                                                        | $\Pi_{(0,21)}8_1^17^1$            | $\Pi_{(3,0)}8_7^13^17^{-1}$            | —  | —     | —          |
| 175C1    | 20160 | $A_8$                                                    | $\Pi_{(0,21)}4_1^13^15^1$         | $\Pi_{(3,0)}4_7^15^1$                  | —  | —     | 40320      |
| 175C1.1  | 40320 | $S_8$                                                    | $\Pi_{(0,21)}4_1^13^15^1$         | $\Pi_{(3,0)}4_7^15^1$                  | —  | —     | —          |
| 175F1    | 20160 | $A_8$                                                    | $\Pi_{(0,21)}4_1^13^15^1$         | $\Pi_{(3,0)}4_7^13^{-2}5^1$            | —  | —     | —          |
| 178C1    | 11520 | —                                                        | $\Pi_{(0,21)}2_2^{-2}8_7^13^1$    | $\Pi_{(3,0)}2_6^28_1^1$                | —  | —     | 23040      |
| 178C1.1  | 23040 | —                                                        | $\Pi_{(0,21)}2_2^{-2}8_7^13^1$    | $\Pi_{(3,0)}2_6^{-2}8_5^{-1}$          | —  | —     | —          |
| 178F1    | 11520 | —                                                        | $\Pi_{(0,21)}2_2^{-2}8_7^13^1$    | $\Pi_{(3,0)}2_6^{-2}8_5^{-1}3^{-2}$    | —  | —     | —          |
| 180F1    | 10752 | —                                                        | $\Pi_{(0,21)}2_6^216_5^{-1}$      | $\Pi_{(3,0)}2_2^216_3^{-1}3^1$         | —  | —     | —          |
| 182F1    | 7920  | $M_{11}$                                                 | $\Pi_{(0,21)}2_7^13^{-1}11^{-1}$  | $\Pi_{(3,0)}2_1^13^211^1$              | —  | —     | —          |
| 183F1    | 5760  | —                                                        | $\Pi_{(0,21)}8_1^13^15^{-1}$      | $\Pi_{(3,0)}8_7^13^25^{-1}$            | —  | —     | —          |
| 184F1    | 4608  | —                                                        | $\Pi_{(0,21)}2_3^{-1}8^{-2}$      | $\Pi_{(3,0)}2_1^18^{-2}3^1$            | —  | —     | —          |
| 186C1    | 3888  | —                                                        | $\Pi_{(0,21)}4_1^13^3$            | $\Pi_{(3,0)}4_7^13^2$                  | —  | —     | 7776       |
| 186C1.1  | 7776  | —                                                        | $\Pi_{(0,21)}4_1^13^3$            | $\Pi_{(3,0)}4_7^13^2$                  | —  | —     | —          |
| 187C1    | 3888  | —                                                        | $\Pi_{(0,21)}2_7^{-3}3^{-2}$      | $\Pi_{(3,0)}2_1^{-3}3^1$               | —  | —     | 7776       |
| 187C1.1  | 7776  | —                                                        | $\Pi_{(0,21)}2_7^{-3}3^{-2}$      | $\Pi_{(3,0)}2_1^{-3}3^1$               | —  | —     | —          |
| 187F1    | 3888  | —                                                        | $\Pi_{(0,21)}2_7^{-3}3^{-2}$      | $\Pi_{(3,0)}2_1^{-3}3^{-3}$            | —  | —     | —          |
| 191C1    | 1944  | [1944, 3536]                                             | $\Pi_{(0,21)}2_1^{-3}3^{-3}$      | $\Pi_{(3,0)}2_3^33^{-2}$               | —  | —     | 3888       |
| 191C1.1  | 3888  | —                                                        | $\Pi_{(0,21)}2_1^{-3}3^{-3}$      | $\Pi_{(3,0)}2_3^33^{-2}$               | —  | —     | —          |
| 193F1    | 1440  | [1440, 5844]                                             | $\Pi_{(0,21)}2_2^24_5^{-1}5^1$    | $\Pi_{(3,0)}2_2^{-2}4_3^{-1}3^15^1$    | —  | —     | —          |
| 193F2    | 1440  | [1440, 5844]                                             | $\Pi_{(0,21)}2_2^24_5^{-1}5^1$    | $\Pi_{(3,0)}2_0^24_1^13^15^1$          | —  | —     | —          |
| 194F1    | 1440  | [1440, 5841]                                             | $\Pi_{(0,21)}2_5^33^{-1}5^1$      | $\Pi_{(3,0)}2_7^{-3}3^25^1$            | —  | —     | —          |
| 194F2    | 1440  | [1440, 5841]                                             | $\Pi_{(0,21)}2_5^33^{-1}5^1$      | $\Pi_{(3,0)}2_7^{-3}3^25^1$            | —  | —     | —          |
| 197F1    | 768   | [768, 1086051]                                           | $\Pi_{(0,21)}2_7^14_1^116_3^{-1}$ | $\Pi_{(3,0)}2_1^14_3^{-1}16_1^13^1$    | —  | —     | —          |
| 197F2    | 768   | [768, 1086051]                                           | $\Pi_{(0,21)}2_7^14_1^116_3^{-1}$ | $\Pi_{(3,0)}2_7^14_1^116_5^{-1}3^1$    | —  | —     | —          |
| 200C1    | 720   | $S_6 \mid [720, 763]$                                    | $\Pi_{(0,21)}2_6^24_1^13^2$       | $\Pi_{(3,0)}2_4^{-2}4_1^13^{-1}$       | —  | —     | 1440       |
| 200C1.1  | 1440  | $C_2 \times S_6 \mid [1440, 5842]$                       | $\Pi_{(0,21)}2_6^24_1^13^2$       | $\Pi_{(3,0)}2_4^{-2}4_1^13^{-1}$       | —  | —     | —          |
| 200F1    | 720   | $S_6 \mid [720, 763]$                                    | $\Pi_{(0,21)}2_6^24_1^13^2$       | $\Pi_{(3,0)}2_6^24_3^{-1}3^3$          | —  | —     | —          |
| 200F2    | 720   | $S_6 \mid [720, 763]$                                    | $\Pi_{(0,21)}2_6^24_1^13^2$       | $\Pi_{(3,0)}2_6^24_3^{-1}3^3$          | —  | —     | —          |
| 201C1    | 432   | $\text{AGL}_2(\mathbb{F}_3) \mid [432, 734]$             | $\Pi_{(0,21)}2_7^13^29^{-1}$      | $\Pi_{(3,0)}2_5^{-1}3^{-1}9^1$         | —  | —     | —          |
| 203F1    | 288   | $C_2 \times \text{AGL}_1(\mathbb{F}_9) \mid [288, 1027]$ | $\Pi_{(0,21)}2_6^{-2}4_1^19^{-1}$ | $\Pi_{(3,0)}2_2^24_3^{-1}3^19^1$       | —  | —     | —          |
| 203F2    | 288   | $C_2 \times \text{AGL}_1(\mathbb{F}_9) \mid [288, 1027]$ | $\Pi_{(0,21)}2_6^{-2}4_1^19^{-1}$ | $\Pi_{(3,0)}2_2^24_3^{-1}3^19^1$       | —  | —     | —          |
| 205C1    | 240   | $C_2 \times S_5 \mid [240, 189]$                         | $\Pi_{(0,21)}2_6^24_7^13^15^{-1}$ | $\Pi_{(3,0)}2_6^{-2}4_1^15^{-1}$       | —  | —     | 480        |
| 205C1.1  | 480   | $C_2^2 \times S_5 \mid [480, 1186]$                      | $\Pi_{(0,21)}2_6^24_7^13^15^{-1}$ | $\Pi_{(3,0)}2_0^24_3^{-1}5^{-1}$       | —  | —     | —          |
| 205F1    | 240   | $C_2 \times S_5 \mid [240, 189]$                         | $\Pi_{(0,21)}2_6^24_7^13^15^{-1}$ | $\Pi_{(3,0)}2_0^24_3^{-1}3^{-2}5^{-1}$ | —  | —     | —          |
| 205F2    | 240   | $C_2 \times S_5 \mid [240, 189]$                         | $\Pi_{(0,21)}2_6^24_7^13^15^{-1}$ | $\Pi_{(3,0)}2_6^{-2}4_1^13^{-2}5^{-1}$ | —  | —     | —          |
| 207F1    | 168   | $\text{AGL}_1(\mathbb{F}_8) \mid [168, 43]$              | $\Pi_{(0,21)}2_3^{-1}8^{-2}$      | $\Pi_{(3,0)}2_1^18^{-2}3^1$            | —  | —     | —          |



Table 2: Birational symplectic effective  $\chi$ -saturated groups

| $(X, G)$ | $\#G$ | Description of $G$                           | $g(\Lambda_G)$                          | $g(\Lambda^G)$                      | K3 | Cubic | Saturation |
|----------|-------|----------------------------------------------|-----------------------------------------|-------------------------------------|----|-------|------------|
| 208C1    | 144   | $S_3 \times S_4 \mid [144, 183]$             | $\Pi_{(0,21)} 2_6^{-2} 8_5^{-1} 3^{-2}$ | $\Pi_{(3,0)} 2_2^{-2} 8_7^1 3^1$    | —  | —     | 288        |
| 208C1.1  | 288   | $C_2 \times S_3 \times S_4 \mid [288, 1028]$ | $\Pi_{(0,21)} 2_6^{-2} 8_5^{-1} 3^{-2}$ | $\Pi_{(3,0)} 2_6^2 8_3^{-1} 3^1$    | —  | —     | —          |
| 208F1    | 144   | $S_3 \times S_4 \mid [144, 183]$             | $\Pi_{(0,21)} 2_6^{-2} 8_5^{-1} 3^{-2}$ | $\Pi_{(3,0)} 2_6^2 8_3^{-1} 3^{-3}$ | —  | —     | —          |
| 208F2    | 144   | $S_3 \times S_4 \mid [144, 183]$             | $\Pi_{(0,21)} 2_6^{-2} 8_5^{-1} 3^{-2}$ | $\Pi_{(3,0)} 2_6^2 8_3^{-1} 3^{-3}$ | —  | —     | —          |
| 211C1    | 120   | $S_5 \mid [120, 34]$                         | $\Pi_{(0,21)} 2_1^{-3} 3^{-3}$          | $\Pi_{(3,0)} 2_3^3 3^{-2}$          | —  | —     | —          |
| 212F1    | 96    | $C_2 \times T_{48} \mid [96, 189]$           | $\Pi_{(0,21)} 2_0^2 16_1^1 3^{-1}$      | $\Pi_{(3,0)} 2_0^2 16_7^1 3^2$      | —  | —     | —          |
| 214C1    | 72    | $C_2 \times S_3^2 \mid [72, 46]$             | $\Pi_{(0,21)} 2_4^{-2} 4_1^1 3^3$       | $\Pi_{(3,0)} 2_6^2 4_1^1 3^2$       | —  | —     | 144        |
| 214C1.1  | 144   | $C_2^2 \times S_3^2 \mid [144, 192]$         | $\Pi_{(0,21)} 2_4^{-2} 4_1^1 3^3$       | $\Pi_{(3,0)} 2_6^2 4_1^1 3^2$       | —  | —     | —          |
| 214C2    | 72    | $C_2 \times S_3^2 \mid [72, 46]$             | $\Pi_{(0,21)} 2_4^{-2} 4_1^1 3^3$       | $\Pi_{(3,0)} 2_6^2 4_1^1 3^2$       | —  | —     | 144        |
| 214C2.1  | 144   | $[144, 186]$                                 | $\Pi_{(0,21)} 2_4^{-2} 4_1^1 3^3$       | $\Pi_{(3,0)} 2_6^2 4_1^1 3^2$       | —  | —     | —          |
| 220F1    | 42    | $F_7 \mid [42, 1]$                           | $\Pi_{(0,21)} 2_3^3 7^{-2}$             | $\Pi_{(3,0)} 2_1^{-3} 3^1 7^{-2}$   | —  | —     | —          |
| 220F2    | 42    | $F_7 \mid [42, 1]$                           | $\Pi_{(0,21)} 2_3^3 7^{-2}$             | $\Pi_{(3,0)} 2_1^{-3} 3^1 7^{-2}$   | —  | —     | —          |
